# Supplementary material for: Rethinking and Recomputing the Value of Machine Learning Models
Source: arXiv:2209.15157 source file (2025-04-23)
Supplement: Supplementary file 1 [file supplement.tex]

\section{Supplementary material}
\subsection{Datasets}
\label{app:DataAndAlg}
Table \ref{tab:datasets} shows the details of each dataset used in our experiments. %Algorithm \ref{alg:expFlow} shows the flow of our experiments.

\subsection{Limitation to NLP}
\label{app:limitToNLPs}
For the time being, our work is limited to NLP because of the following reasons:

\begin{itemize}
    \item Our idea stems from our experience in industrial use cases that were all NLP based, and in fact, they are all classifiers that have an NLP aspect in them. This does not mean that value-based approaches cannot apply in other contexts, and in fact, we believe they may apply to many non-NLP classifications or image processing problems, root cause analysis, and more. However, while we do have customers that use for example document intelligence and causal analysis capabilities, the way quality is measured and the workflow for integrating models into production is very different in that context - at least, that is our experience. Because one of the points we make in the paper is that we want to connect model quality metrics to use cases - and specifically enterprise AI use cases - we focus on the broad class of use cases we routinely work with and where we know the considerations of value definitely apply.
    \item We have an NLP-specific hypothesis we postulate and briefly discuss in the paper, which stems from what we have witnessed in proprietary datasets: when text encoders are pre-trained on general-purpose datasets and applied on enterprise datasets where the language is often a company-specific kind of “dialect”, then the difference between value and accuracy is significant. Indeed, this observation and the realization that we would be using the wrong model to serve our customers if we used accuracy is what led to this line of work. Because we could not post proprietary datasets we showed what happens with public out-of-domain datasets.
    \item Further considerations can be made when applying pre-trained or fine-tuned LLMs, such as T5, and we show in this paper that it can work great out of the box in some cases but if we disregard the “confidence” and filtering aspect (a common trend, as we have witnessed), this can prove to be very damaging depending on the cost ratio, and again can lead to choosing the wrong model (or choosing a T5 base vs large, with very different calibration profiles). 
    \item We believe the notion of value to be useful in general, but if we find that value and accuracy are very strongly correlated (also in ranking models), then we can perfectly live with accuracy. We have found that this correlation exists only in some cases but is in no way general for NLP problems. We cannot broaden the statement (for now) beyond the experiments we have made.
\end{itemize}

\newpage
\subsection{Further Results}
\label{app:FurtherResults}

\subsubsection{Binary datasets - Supplementary results for cost-sensitive learning}

%\begin{figure*}
% \centering
%    \includegraphics[width=.24\linewidth]{figs/Badj., Exp1.png}
%    \includegraphics[width=.24\linewidth]{figs/Badj., Exp2.png}
%    \includegraphics[width=.24\linewidth]{figs/Agr., Exp1.png}
%    \includegraphics[width=.24\linewidth]{figs/Agr., Exp2.png}
    
%    \caption{\label{fig:confDistSOTAHateSpeech} Confidence distributions of SOTA models on Hate Speech Dataset.}
%      \vspace{-0.15in}
%\end{figure*}%

\begin{figure*}[!htbp]
 \centering
    \includegraphics[width=.245\linewidth]{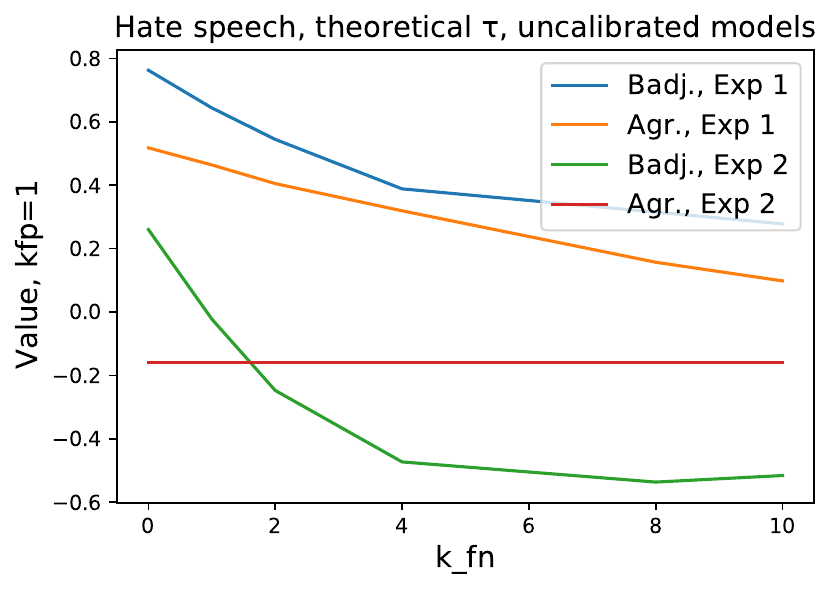} 
    \includegraphics[width=.245\linewidth]{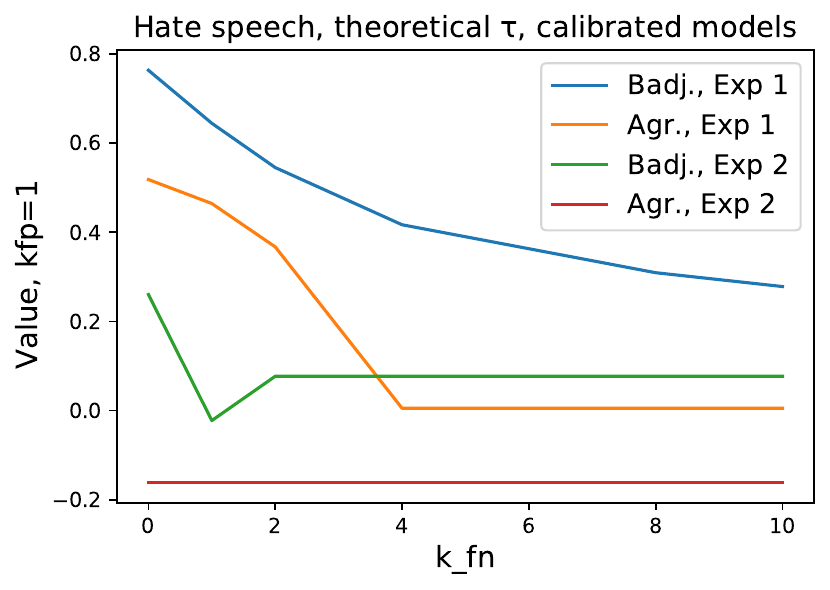} 
    \includegraphics[width=.245\linewidth]{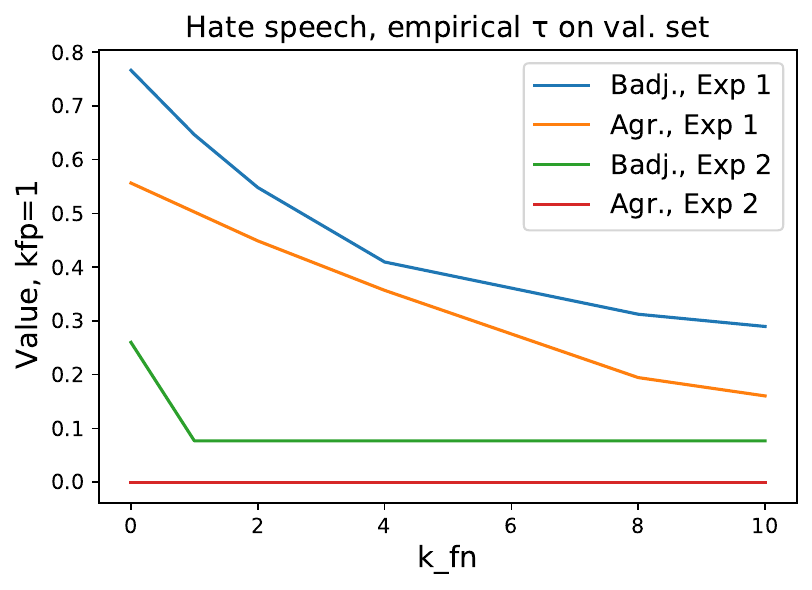} 
    \includegraphics[width=.245\linewidth]{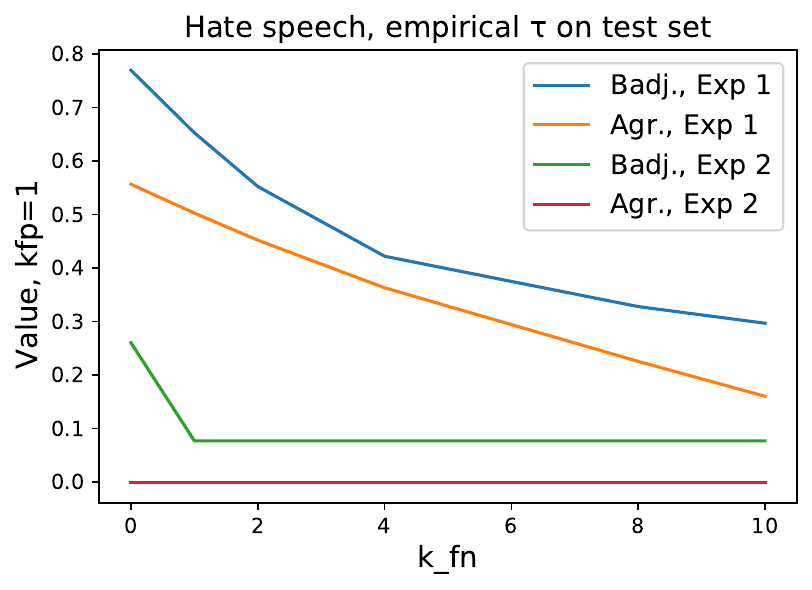}
    \includegraphics[width=.245\linewidth]{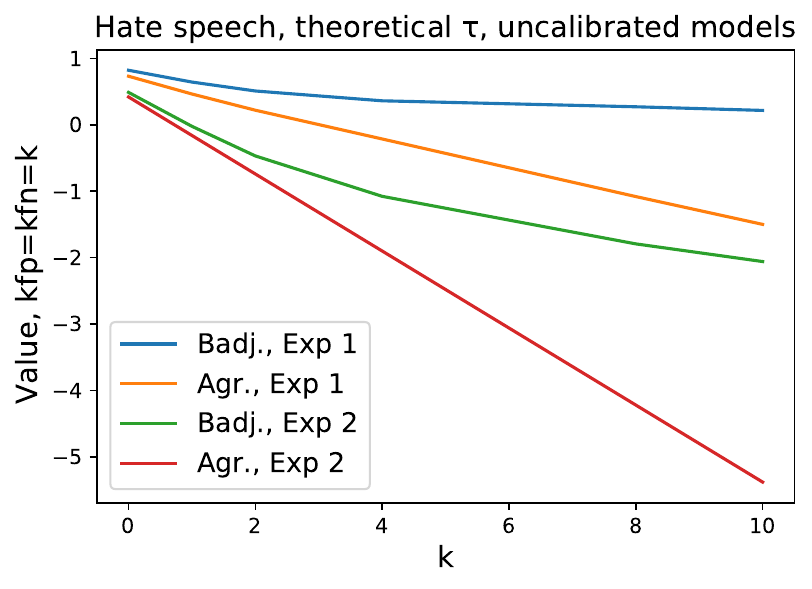} 
    \includegraphics[width=.245\linewidth]{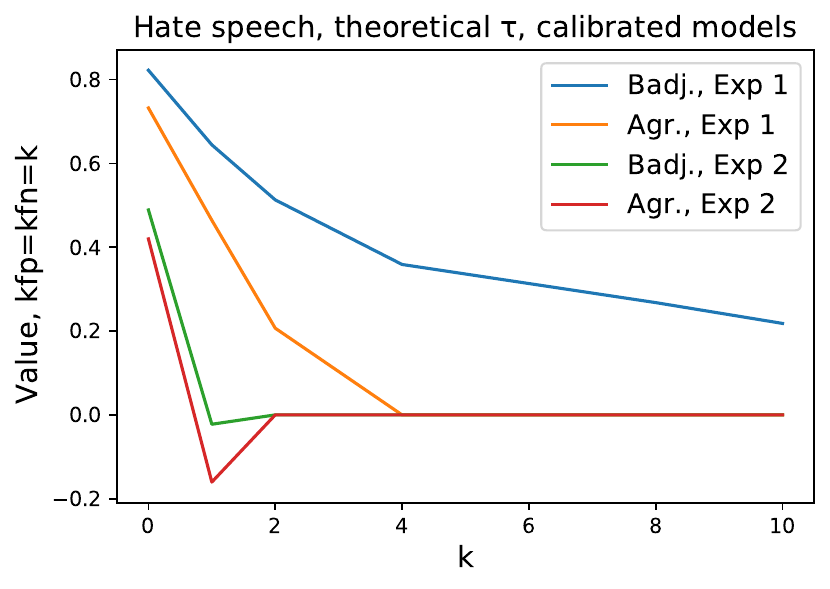} 
    \includegraphics[width=.245\linewidth]{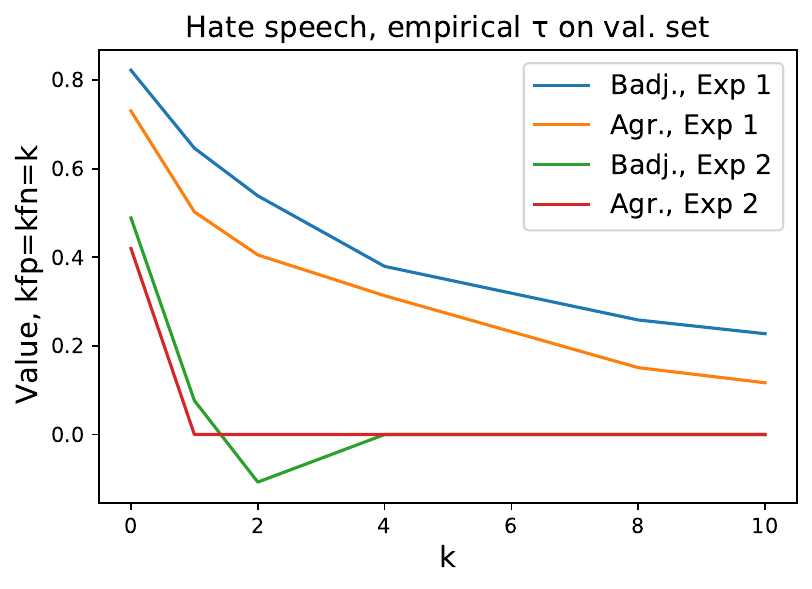} 
    \includegraphics[width=.245\linewidth]{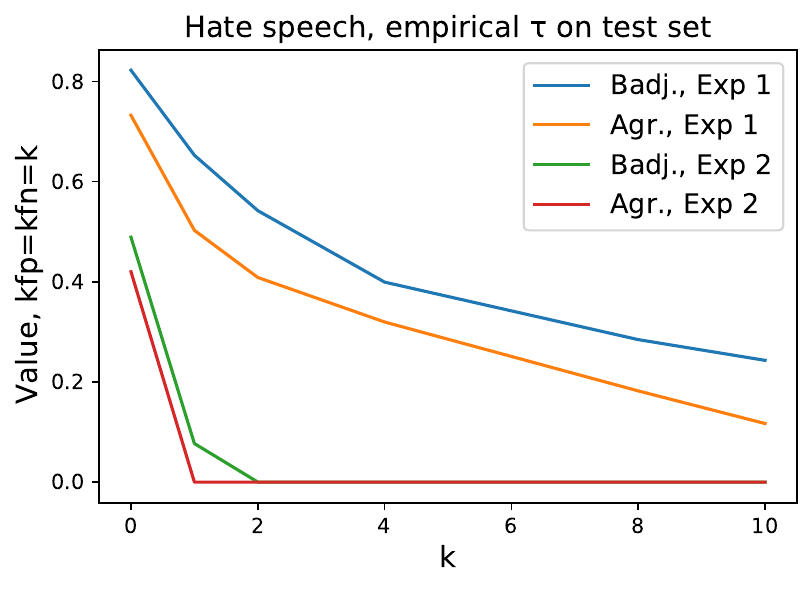}

    \includegraphics[width=.245\linewidth]{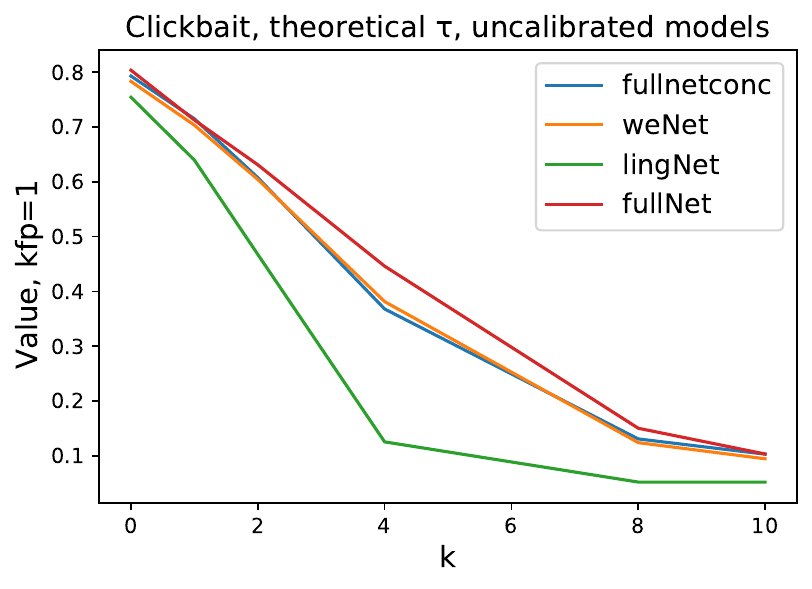}
    \includegraphics[width=.245\linewidth]{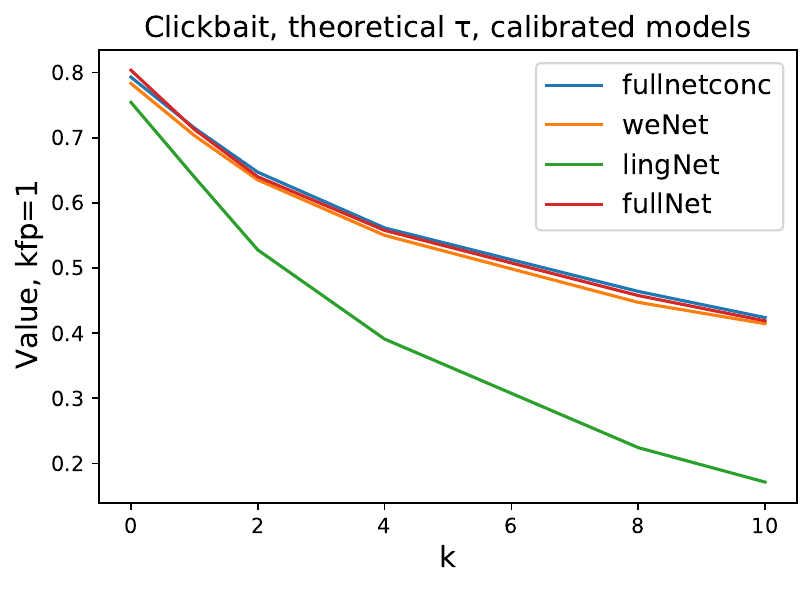}
    \includegraphics[width=.245\linewidth]{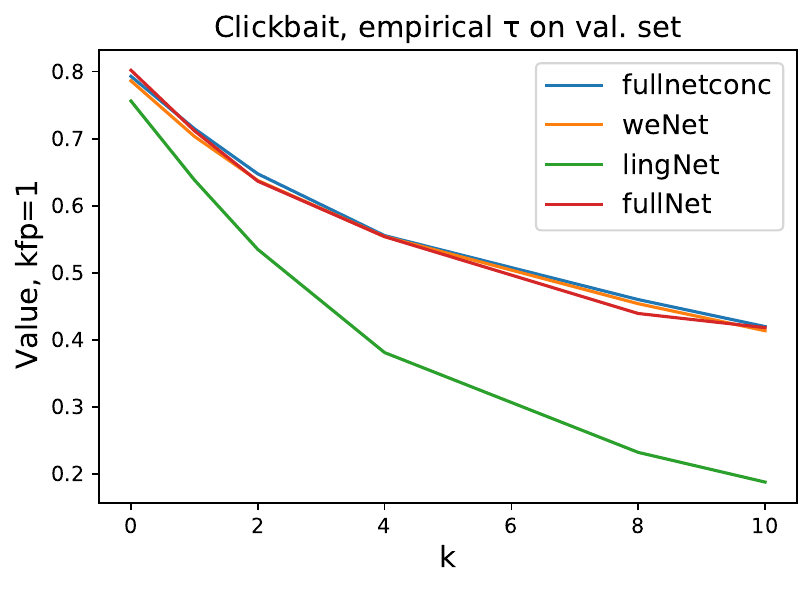}
    \includegraphics[width=.245\linewidth]{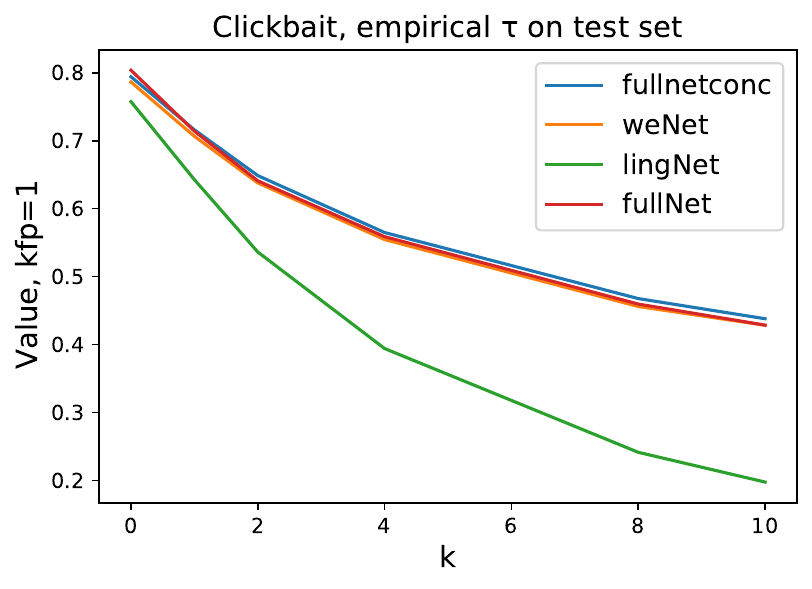}
    \includegraphics[width=.245\linewidth]{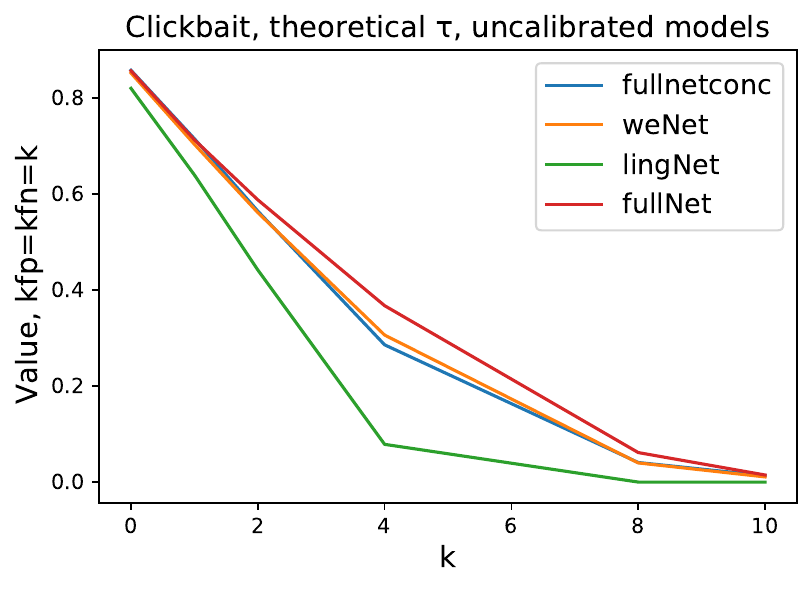}
    \includegraphics[width=.245\linewidth]{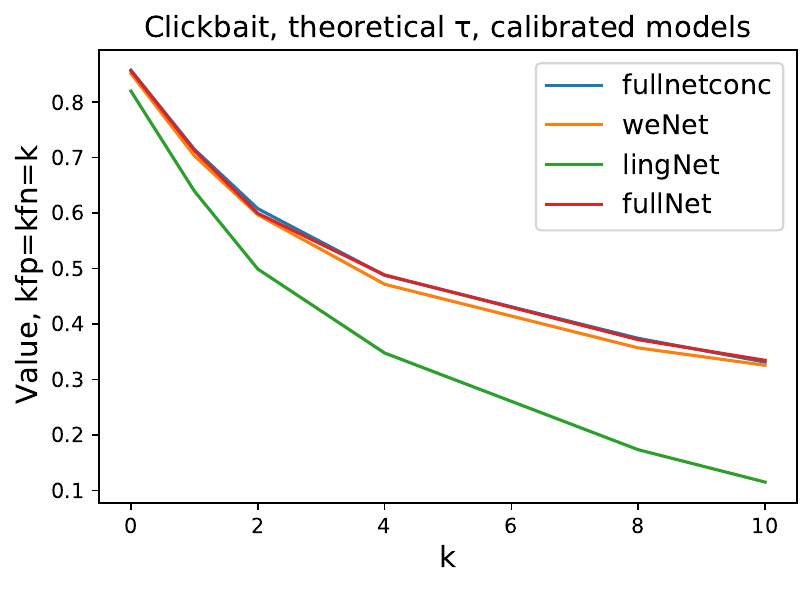}
    \includegraphics[width=.245\linewidth]{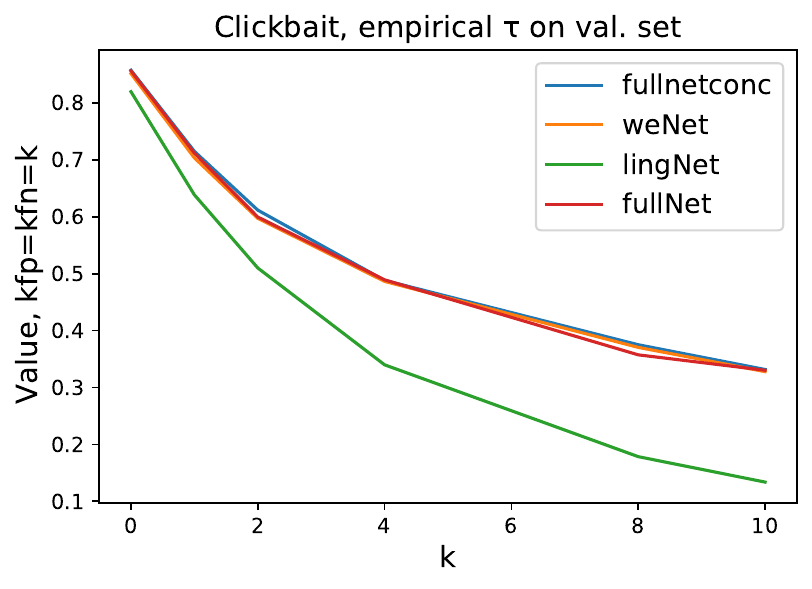}
    \includegraphics[width=.245\linewidth]{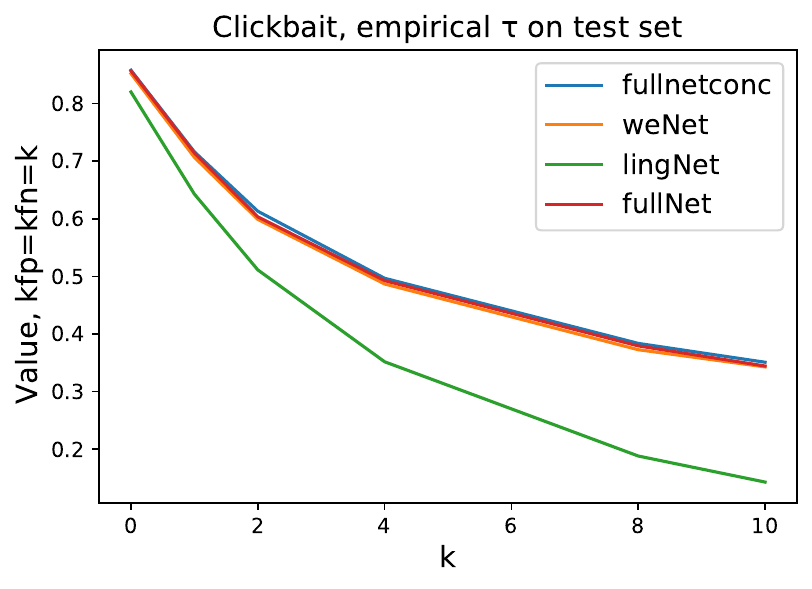}
    
    \caption{\label{fig:app-value_leaderboards_REP}Value curves of binary datasets for increasing $k$.}
\end{figure*}%%

\newpage

\begin{table*}[ht]
    \begin{center}
    \begin{small}
    \begin{sc}
    \scalebox{0.75}{%
    \centering
    \begin{tabular}{llllllll}
    \hline
   \multirow{2}{*}{\textbf{Task}} & \multirow{2}{*}{\textbf{Model}} & \multirow{2}{*}{\textbf{Accuracy}} & \multirow{2}{*}{\textbf{$Value_1$}} & \multirow{2}{*}{\textbf{$Value_2$}} & \multirow{2}{*}{\textbf{$Value_4$}} & \multirow{2}{*}{\textbf{$Value_8$}} & \multirow{2}{*}{\textbf{$Value_{10}$}}\\
    \\

    & & ($k_{fn} = k_{fp} = 0$) & ($k_{fn} =1$) & ($k_{fn} =2$) & ($k_{fn} =4$) & ($k_{fn} =8$) & ($k_{fn} =10$)
     \\

         \hline
         Hate-speech & Badj. et al., \textit{Exp. 1} & \textbf{0.822} & \textbf{0.644} & \textbf{0.545} & \textbf{0.389} & \textbf{0.315} & \textbf{0.278} \\
         & Agr. et al., \textit{Exp. 1} & 0.732 & 0.464 & 0.405 & 0.32 & 0.157 & 0.098\\ 
         & Badj. et al., \textit{Exp. 2} & \textbf{0.489} & \textbf{-0.022} & -0.248 & -0.473 & -0.537 & -0.516 \\ 
         & Agr. et al., \textit{Exp. 2} & 0.42 & -0.16 & \textbf{-0.16} & \textbf{-0.16} & \textbf{-0.16} & \textbf{-0.16} \\ 
  
         Clickbait & fullnetconc & \textbf{0.857} & \textbf{0.715} & 0.608 & 0.368 & 0.131 & \textbf{0.103} \\ 
         & weNet & 0.852 & 0.703 & 0.604 & 0.381 & 0.124 & 0.094 \\ 
         & lingNet & 0.82 & 0.64 & 0.467 & 0.125 & 0.052 & 0.052 \\ 
         & fullNet & 0.856 & 0.713 & \textbf{0.631} & \textbf{0.446} & \textbf{0.15} & \textbf{0.103} \\ 
         \hline
    \end{tabular}%
    }
    \end{sc}
    \end{small}
    \end{center}
    \caption{Performance of SOTA models, with theoretical threshold ($k_{fp}$ is set to 1, and $k_{fn} \in \{ 1, 2, 4, 8, 10\}$).}
    \label{tab:performanceSOTACase1}
\end{table*}

\begin{table*}[!htbp]
    \begin{center}
    \begin{small}
    \begin{sc}
    \scalebox{0.75}{%
    \centering
    \begin{tabular}{llllllll}
    \hline
   \multirow{2}{*}{\textbf{Task}} & \multirow{2}{*}{\textbf{Model}} & \multirow{2}{*}{\textbf{Accuracy}} & \multirow{2}{*}{\textbf{$Value_1$}} & \multirow{2}{*}{\textbf{$Value_2$}} & \multirow{2}{*}{\textbf{$Value_4$}} & \multirow{2}{*}{\textbf{$Value_8$}} & \multirow{2}{*}{\textbf{$Value_{10}$}}\\
    \\

    & & ($k_{fn} = k_{fp} = 0$) & ($k_{fn} =1$) & ($k_{fn} =2$) & ($k_{fn} =4$) & ($k_{fn} =8$) & ($k_{fn} =10$)
     \\

         \hline
         Hate-speech & Badj. et al., \textit{Exp. 1} & \textbf{0.822} & \textbf{0.644} & \textbf{0.51} & \textbf{0.362} & \textbf{0.272} & \textbf{0.217} \\
         & Agr. et al., \textit{Exp. 1} & 0.732 & 0.464 & 0.22 & -0.213 & -1.081 & -1.499\\ 
         & Badj. et al., \textit{Exp. 2} & \textbf{0.489} & \textbf{-0.022} & \textbf{-0.469} & \textbf{-1.077} & \textbf{-1.793} & \textbf{-2.06} \\
         & Agr. et al., \textit{Exp. 2} & 0.42 & -0.16 & -0.74 & -1.901 & -4.221 & -5.382\\ 

         Clickbait & fullnetconc & \textbf{0.857} & \textbf{0.715} & 0.564 & 0.286 & 0.041 & 0.013 \\ 
         & weNet & 0.852 & 0.703 & 0.561 & 0.306 & 0.04 & 0.011 \\ 
         & lingNet & 0.82 & 0.64 & 0.442 & 0.079 & 0.0 & 0.0 \\ 
         & fullNet & 0.856 & 0.713 & \textbf{0.588} & \textbf{0.367} & \textbf{0.061} & \textbf{0.015} \\ 
         \hline
    \end{tabular}%
    }
    \end{sc}
    \end{small}
    \end{center}
    \caption{Performance of SOTA models, with theoretical threshold ($k_{fp}$ = $k_{fn} \in \{ 1, 2, 4, 8, 10\}$).}
    \label{tab:performanceSOTACase1Eq}
\end{table*}

\begin{table*}[!htbp]
    \begin{center}
    \begin{small}
    \begin{sc}
    \scalebox{0.75}{%
    \begin{tabular}{llllllll}
    \hline
    \multirow{2}{*}{\textbf{Task}} & \multirow{2}{*}{\textbf{Model}} & \multirow{2}{*}{\textbf{Accuracy}} & \multirow{2}{*}{\textbf{$Value_1$}} & \multirow{2}{*}{\textbf{$Value_2$}} & \multirow{2}{*}{\textbf{$Value_4$}} & \multirow{2}{*}{\textbf{$Value_8$}} & \multirow{2}{*}{\textbf{$Value_{10}$}}\\
    \\

    & & ($k_{fn} = k_{fp} = 0$) & ($k_{fn} =1$) & ($k_{fn} =2$) & ($k_{fn} =4$) & ($k_{fn} =8$) & ($k_{fn} =10$)
     \\

         \hline
         Hate-speech & Badj. et al., \textit{Exp. 1} & \textbf{0.822} & \textbf{0.644} & \textbf{0.545} & \textbf{0.417} & \textbf{0.309} & \textbf{0.278} \\
         & Agr. et al., \textit{Exp. 1} & 0.732 & 0.464 & 0.367 & 0.005 & 0.005 & 0.005 \\ 
         & Badj. et al., \textit{Exp. 2} & \textbf{0.489} & \textbf{-0.022} & \textbf{0.077} & \textbf{0.077} & \textbf{0.077} & \textbf{0.077} \\ 
         & Agr. et al., \textit{Exp. 2} & 0.42 & -0.16 & -0.16 & -0.16 & -0.16 & -0.16\\ 
       
         Clickbait & fullnetconc & \textbf{0.857} & \textbf{0.715} & \textbf{0.647} & \textbf{0.562} & \textbf{0.464} & \textbf{0.424} \\ 
         & weNet & 0.852 & 0.703 & 0.635 & 0.55 & 0.447 & 0.414 \\ 
         & lingNet & 0.82 & 0.64 & 0.528 & 0.391 & 0.224 & 0.171 \\ 
         & fullNet & 0.856 & 0.713 & 0.64 & 0.558 & 0.458 & 0.419 \\ 
         \hline
    \end{tabular}%
    }
    \end{sc}
    \end{small}
    \end{center}
    \caption{Performance of SOTA models after temperature scaling, with theoretical threshold ($k_{fp}$ is set to 1)}
    \label{tab:performanceSOTACase2}
\end{table*}

\begin{table*}[!htbp]
    \begin{center}
    \begin{small}
    \begin{sc}
    \scalebox{0.75}{%
    \begin{tabular}{llllllll}
    \hline
    \multirow{2}{*}{\textbf{Task}} & \multirow{2}{*}{\textbf{Model}} & \multirow{2}{*}{\textbf{Accuracy}} & \multirow{2}{*}{\textbf{$Value_1$}} & \multirow{2}{*}{\textbf{$Value_2$}} & \multirow{2}{*}{\textbf{$Value_4$}} & \multirow{2}{*}{\textbf{$Value_8$}} & \multirow{2}{*}{\textbf{$Value_{10}$}}\\
    \\

    & & ($k_{fn} = k_{fp} = 0$) & ($k_{fn} =1$) & ($k_{fn} =2$) & ($k_{fn} =4$) & ($k_{fn} =8$) & ($k_{fn} =10$)
     \\

         \hline
         Hate-speech & Badj. et al., \textit{Exp. 1} & \textbf{0.822} & \textbf{0.644} & \textbf{0.513} & \textbf{0.359} & \textbf{0.268} & \textbf{0.218} \\
         & Agr. et al., \textit{Exp. 1} & 0.732 & 0.464 & 0.207 & 0.0 & 0.0 & 0.0 \\ 
         & Badj. et al., \textit{Exp. 2} & \textbf{0.489} & \textbf{-0.022} & 0.0 & 0.0 & 0.0 & 0.0 \\ 
         & Agr. et al., \textit{Exp. 2} & 0.42 & -0.16 & 0.0 & 0.0 & 0.0 & 0.0 \\ 
   
         Clickbait & fullnetconc & \textbf{0.857} & \textbf{0.715} & \textbf{0.608} & \textbf{0.488} & \textbf{0.374} & 0.331 \\ 
         & weNet & 0.852 & 0.703 & 0.597 & 0.472 & 0.357 & 0.326 \\ 
         & lingNet & 0.82 & 0.64 & 0.499 & 0.348 & 0.173 & 0.115 \\ 
         & fullNet & 0.856 & 0.713 & 0.6 & \textbf{0.488} & 0.372 & \textbf{0.335} \\ 
         \hline
    \end{tabular}%
    }
    \end{sc}
    \end{small}
    \end{center}
        \caption{Performance of SOTA models after temperature scaling, with theoretical threshold ($k_{fp}$ = $k_{fn}$)}.
    \label{tab:performanceSOTACase2Eq}
\end{table*}

\newpage

\begin{table*}[!htbp]
    \begin{center}
    \begin{small}
    \begin{sc}
    \scalebox{0.75}{%
    \begin{tabular}{llllllll}
    \hline
    \multirow{2}{*}{\textbf{Task}} & \multirow{2}{*}{\textbf{Model}} & \multirow{2}{*}{\textbf{Accuracy}} & \multirow{2}{*}{\textbf{$Value_1$}} & \multirow{2}{*}{\textbf{$Value_2$}} & \multirow{2}{*}{\textbf{$Value_4$}} & \multirow{2}{*}{\textbf{$Value_8$}} & \multirow{2}{*}{\textbf{$Value_{10}$}}\\
    \\

    & & ($k_{fn} = k_{fp} = 0$) & ($k_{fn} =1$) & ($k_{fn} =2$) & ($k_{fn} =4$) & ($k_{fn} =8$) & ($k_{fn} =10$)
     \\

         \hline
         Hate-speech & Badj. et al., \textit{Exp. 1} & \textbf{0.822} & \textbf{0.646} & \textbf{0.548} & \textbf{0.41} & \textbf{0.312} & \textbf{0.29} \\
         & Agr. et al., \textit{Exp. 1} & 0.732 & 0.503 & 0.449 & 0.357 & 0.194 & 0.16 \\
         & Badj. et al., \textit{Exp. 2} & \textbf{0.489} & \textbf{0.077} & \textbf{0.077} & \textbf{0.077} & \textbf{0.077} & \textbf{0.077} \\ 
         & Agr. et al., \textit{Exp. 2} & 0.42 & 0.0 & 0.0 & 0.0 & 0.0 & 0.0\\ 
  
         Clickbait & fullnetconc & \textbf{0.857} & \textbf{0.715} & \textbf{0.648} & \textbf{0.556} & \textbf{0.46} & \textbf{0.42} \\ 
         & weNet & 0.852 & 0.703 & 0.638 & 0.554 & 0.454 & 0.414 \\ 
         & lingNet & 0.82 & 0.639 & 0.535 & 0.381 & 0.232 & 0.188 \\ 
         & fullNet & 0.856 & 0.712 & 0.637 & 0.554 & 0.439 & 0.418 \\ 
         \hline
    \end{tabular}%
    }
    \end{sc}
    \end{small}
    \end{center}
        \caption{Performance of SOTA models, with empirical threshold (found on the validation set, $k_{fp}$ is set to 1)}
    \label{tab:performanceSOTACase3}
\end{table*}

\begin{table*}[!htbp]
    \begin{center}
    \begin{small}
    \begin{sc}
    \scalebox{0.75}{%
    \begin{tabular}{llllllll}
    \hline
    \multirow{2}{*}{\textbf{Task}} & \multirow{2}{*}{\textbf{Model}} & \multirow{2}{*}{\textbf{Accuracy}} & \multirow{2}{*}{\textbf{$Value_1$}} & \multirow{2}{*}{\textbf{$Value_2$}} & \multirow{2}{*}{\textbf{$Value_4$}} & \multirow{2}{*}{\textbf{$Value_8$}} & \multirow{2}{*}{\textbf{$Value_{10}$}}\\
    \\

    & & ($k_{fn} = k_{fp} = 0$) & ($k_{fn} =1$) & ($k_{fn} =2$) & ($k_{fn} =4$) & ($k_{fn} =8$) & ($k_{fn} =10$)
     \\

         \hline
         Hate-speech & Badj. et al., \textit{Exp. 1} & \textbf{0.822} & \textbf{0.646} & \textbf{0.539} & \textbf{0.38} & \textbf{0.259} & \textbf{0.228} \\
         & Agr. et al., \textit{Exp. 1} & 0.732 & 0.503 & 0.405 & 0.313 & 0.151 & 0.117 \\ 
         & Badj. et al., \textit{Exp. 2} & \textbf{0.489} & \textbf{0.077} & -0.107 & 0.0 & 0.0 & 0.0 \\ 
         & Agr. et al., \textit{Exp. 2} & 0.42 & 0.0 & \textbf{0.0} & 0.0 & 0.0 & 0.0 \\ 

         Clickbait & fullnetconc & \textbf{0.857} & \textbf{0.715} & \textbf{0.612} & 0.488 & \textbf{0.375} & \textbf{0.332} \\ 
         & weNet & 0.852 & 0.703 & 0.597 & 0.486 & 0.371 & 0.328 \\ 
         & lingNet & 0.82 & 0.639 & 0.51 & 0.34 & 0.179 & 0.134 \\ 
         & fullNet & 0.856 & 0.712 & 0.6 & \textbf{0.489} & 0.357 & 0.33 \\ 
         \hline
    \end{tabular}%
    }
    \end{sc}
    \end{small}
    \end{center}
    \caption{Performance of SOTA models with empirical threshold (found on validation set, $k_{fp}$ = $k_{fn}$)}.
    \label{tab:performanceSOTACase3Eq}
\end{table*}

\begin{table*}[ht]
    \begin{center}
    \begin{small}
    \begin{sc}
    \scalebox{0.75}{%
    \begin{tabular}{llllllll}
    \hline
    \multirow{2}{*}{\textbf{Task}} & \multirow{2}{*}{\textbf{Model}} & \multirow{2}{*}{\textbf{Accuracy}} & \multirow{2}{*}{\textbf{$Value_1$}} & \multirow{2}{*}{\textbf{$Value_2$}} & \multirow{2}{*}{\textbf{$Value_4$}} & \multirow{2}{*}{\textbf{$Value_8$}} & \multirow{2}{*}{\textbf{$Value_{10}$}}\\
    \\

    & & ($k_{fn} = k_{fp} = 0$) & ($k_{fn} =1$) & ($k_{fn} =2$) & ($k_{fn} =4$) & ($k_{fn} =8$) & ($k_{fn} =10$)
     \\

         \hline
        Hate-speech & Badj. et al., \textit{Exp. 1} & \textbf{0.822} & \textbf{0.653} & \textbf{0.552} & \textbf{0.422} & \textbf{0.328} & \textbf{0.297} \\
         & Agr. et al., \textit{Exp. 1} & 0.732 & 0.503 & 0.452 & 0.363 & 0.225 & 0.16 \\ 
         & Badj. et al., \textit{Exp. 2} & \textbf{0.489} & \textbf{0.077} & \textbf{0.077} & \textbf{0.077} & \textbf{0.077} & \textbf{0.077} \\ 
         & Agr. et al., \textit{Exp. 2} & 0.42 & 0.0 & 0.0 & 0.0 & 0.0 & 0.0 \\ 

         Clickbait & fullnetconc & \textbf{0.857} & \textbf{0.716} & \textbf{0.649} & \textbf{0.565} & \textbf{0.468} & \textbf{0.438} \\ 
         & weNet & 0.852 & 0.706 & 0.638 & 0.555 & 0.456 & 0.428 \\ 
         & lingNet & 0.82 & 0.643 & 0.536 & 0.394 & 0.242 & 0.198 \\ 
         & fullNet & 0.856 & 0.714 & 0.641 & 0.559 & 0.46 & 0.429\\ 
         \hline
    \end{tabular}%
    }
    \end{sc}
    \end{small}
    \end{center}
    \caption{Performance of SOTA models, with empirical threshold (found on the test set, $k_{fp}$ is set to 1)}
    \label{tab:performanceSOTACase4}
\end{table*}

\begin{table*}[!htbp]
    \begin{center}
    \begin{small}
    \begin{sc}
    \scalebox{0.75}{%
    \begin{tabular}{llllllll}
    \hline
    \multirow{2}{*}{\textbf{Task}} & \multirow{2}{*}{\textbf{Model}} & \multirow{2}{*}{\textbf{Accuracy}} & \multirow{2}{*}{\textbf{$Value_1$}} & \multirow{2}{*}{\textbf{$Value_2$}} & \multirow{2}{*}{\textbf{$Value_4$}} & \multirow{2}{*}{\textbf{$Value_8$}} & \multirow{2}{*}{\textbf{$Value_{10}$}}\\
    \\

    & & ($k_{fn} = k_{fp} = 0$) & ($k_{fn} =1$) & ($k_{fn} =2$) & ($k_{fn} =4$) & ($k_{fn} =8$) & ($k_{fn} =10$)
     \\

         \hline
         Hate-speech & Badj. et al., \textit{Exp. 1} & \textbf{0.822} & \textbf{0.653} & \textbf{0.542} & \textbf{0.399} & \textbf{0.284} & \textbf{0.243} \\
         & Agr. et al., \textit{Exp. 1} & 0.732 & 0.503 & 0.408 & 0.32 & 0.182 & 0.117 \\ 
         & Badj. et al., \textit{Exp. 2} & \textbf{0.489} & \textbf{0.077} & 0.0 & 0.0 & 0.0 & 0.0 \\ 
         & Agr. et al., \textit{Exp. 2} & 0.42 & 0.0 & 0.0 & 0.0 & 0.0 & 0.0 \\ 
         Clickbait & fullnetconc & \textbf{0.857} & \textbf{0.716} & \textbf{0.613} & \textbf{0.497} & \textbf{0.384} & \textbf{0.351} \\ 
         & weNet & 0.852 & 0.706 & 0.599 & 0.487 & 0.373 & 0.343 \\ 
         & lingNet & 0.82 & 0.643 & 0.511 & 0.352 & 0.188 & 0.143 \\ 
         & fullNet & 0.856 & 0.714 & 0.603 & 0.493 & 0.379 & 0.344 \\ 
         \hline
    \end{tabular}%
    }
    \end{sc}
    \end{small}
    \end{center}
    \caption{Performance of SOTA models after temperature scaling, with empirical threshold (on test set, $k_{fp}$ = $k_{fn}$)}
    \label{tab:performanceSOTACase4Eq}
\end{table*}
\newpage

\twocolumn
\subsubsection{MDS dataset - Supplementary Results}

\begin{table}[!htbp]
    \begin{center}
    \begin{small}
    \begin{sc}
    \scalebox{0.7}{%
    \centering
    \begin{tabular}{lllllll}
    \hline
    \multirow{2}{*}{\textbf{Model}} & \multirow{2}{*}{\textbf{Accuracy}} &  \multicolumn{5}{c}{\textbf{Value}}  \\
    & & k=1 & k=2 & k=4 & k=8 & k=10 \\
    \hline
      LogReg & 0.74 & 0.48 & 0.375 & 0.295 & 0.255 & \textbf{0.251}    \\
      MLP1 &  0.728 & 0.457 & 0.36 & 0.298 & \textbf{0.26} & \textbf{0.251}   \\
      MLP4 &  0.72 & 0.439 & 0.327 & 0.16 & -0.089 & -0.193   \\
      mttri &  0.753 & 0.506 & 0.352 & 0.072 & -0.431 & -0.663  \\
      T5 &  0.789 & 0.578 & 0.47 & 0.253 & -0.179 & -0.395\\
      SieBERT &  \textbf{0.836} & \textbf{0.672} & \textbf{0.577} & \textbf{0.392} & 0.029 & -0.15 \\
    \hline
    \end{tabular}
    }
    \end{sc}
    \end{small}
    \end{center}
    \caption{Performance of models on Multi Domain Sentiment Dataset, TARGET = DVD, $k_{fp} = 1$, $k_{fn}=k$ (Value with theoretical threshold)}
    \label{tab:perfMDS_dvd_1}
\end{table}

\begin{table}[!htbp]
    \begin{center}
    \begin{small}
    \begin{sc}
    \scalebox{0.7}{%
    \centering
    \begin{tabular}{lllllll}
    \hline
    \multirow{2}{*}{\textbf{Model}} & \multirow{2}{*}{\textbf{Accuracy}} &  \multicolumn{5}{c}{\textbf{Value}}  \\
    & & k=1 & k=2 & k=4 & k=8 & k=10 \\
    \hline
      LogReg &  0.74 & 0.48 & 0.283 & 0.122 & 0.038 & 0.027 \\
      MLP1 & 0.728 & 0.457 & 0.274 & 0.133 & \textbf{0.054} & \textbf{0.038} \\
      MLP4 & 0.72 & 0.439 & 0.202 & -0.158 & -0.737 & -0.981  \\
      mttri & 0.753 & 0.506 & 0.28 & -0.123 & -0.84 & -1.166  \\
      T5 &  0.789 & 0.578 & 0.367 & -0.056 & -0.9 & -1.323\\
      SieBERT & \textbf{0.836} & \textbf{0.672} & \textbf{0.508} & \textbf{0.193} & -0.436 & -0.747 \\
    \hline
    \end{tabular}
    }
    \end{sc}
    \end{small}
    \end{center}
    \caption{Performance of models on Multi Domain Sentiment Dataset, TARGET = DVD, $k_{fp}=k_{fn}=k$ (Value with theoretical threshold)}
    \label{tab:perfMDS_dvd}
\end{table}

\begin{table}[!htbp]
    \begin{center}
    \begin{small}
    \begin{sc}
    \scalebox{0.7}{%
    \centering
    \begin{tabular}{lllllll}
    \hline
    \multirow{2}{*}{\textbf{Model}} & \multirow{2}{*}{\textbf{Accuracy}} &  \multicolumn{5}{c}{\textbf{Value}}  \\
    & & k=1 & k=2 & k=4 & k=8 & k=10 \\
    \hline
      LogReg &  0.704 & 0.408 & 0.332 & 0.269 & \textbf{0.222} & \textbf{0.219} \\
      MLP1 &  0.691 & 0.382 & 0.272 & 0.197 & 0.18 & 0.183 \\
      MLP4 &  0.696 & 0.393 & 0.258 & 0.081 & -0.183 & -0.283 \\
      mttri & 0.742 & 0.484 & 0.32 & 0.018 & -0.52 & -0.789  \\
      T5 & 0.77 & 0.541 & 0.468 & 0.321 & 0.029 & -0.117 \\
      SieBERT & \textbf{0.826} & \textbf{0.652} & \textbf{0.564} & \textbf{0.389} & 0.038 & -0.131 \\
    \hline
    \end{tabular}%
    }
    \end{sc}
    \end{small}
    \end{center}
    \caption{Performance of models on Multi Domain Sentiment Dataset, TARGET = Books, $k_{fp} = 1$, $k_{fn}=k$ (Value with theoretical threshold)}
    \label{tab:perfMDS_books_1}
\end{table}

\begin{table}[!htbp]
    \begin{center}
    \begin{small}
    \begin{sc}
    \scalebox{0.7}{%
    \centering
    \begin{tabular}{lllllll}
    \hline
    \multirow{2}{*}{\textbf{Model}} & \multirow{2}{*}{\textbf{Accuracy}} &  \multicolumn{5}{c}{\textbf{Value}}  \\
    & & k=1 & k=2 & k=4 & k=8 & k=10 \\
    \hline
      LogReg & 0.704 & 0.408 & 0.228 & 0.102 & \textbf{0.022} & \textbf{0.015}  \\
      MLP1 & 0.691 & 0.382 & 0.134 & 0.013 & -0.017 & -0.013 \\
      MLP4 & 0.696 & 0.393 & 0.154 & -0.171 & -0.666 & -0.86  \\
      mttri & 0.742 & 0.484 & 0.254 & -0.16 & -0.869 & -1.215  \\
      T5 & 0.77 & 0.541 & 0.311 & -0.148 & -1.066 & -1.525 \\
      SieBERT & \textbf{0.826} & \textbf{0.652} & \textbf{0.479} & \textbf{0.136} & -0.547 & -0.879 \\
    \hline
    \end{tabular}%
    }
    \end{sc}
    \end{small}
    \end{center}
    \caption{Performance of models on Multi Domain Sentiment Dataset, TARGET = Books, $k_{fp}=k_{fn}=k$ (Value with theoretical threshold)}
    \label{tab:perfMDS_books}
\end{table}

\begin{table}[!htbp]
    \begin{center}
    \begin{small}
    \begin{sc}
    \scalebox{0.7}{%
    \centering
    \begin{tabular}{lllllll}
    \hline
    \multirow{2}{*}{\textbf{Model}} & \multirow{2}{*}{\textbf{Accuracy}} &  \multicolumn{5}{c}{\textbf{Value}}  \\
    & & k=1 & k=2 & k=4 & k=8 & k=10 \\
    \hline
      LogReg & 0.762 & 0.524 & 0.442 & \textbf{0.355} & \textbf{0.293} & \textbf{0.282} \\
      MLP1 & 0.749 & 0.497 & 0.413 & 0.338 & 0.284 & 0.274 \\
      MLP4 & 0.735 & 0.47 & 0.33 & 0.09 & -0.313 & -0.492 \\
      mttri & 0.808 & 0.616 & 0.495 & 0.286 & -0.085 & -0.245 \\
      T5 & 0.784 & 0.568 & 0.417 & 0.116 & -0.486 & -0.787 \\
      SieBERT & \textbf{0.842} & \textbf{0.685} & \textbf{0.572} & 0.349 & -0.093 & -0.314 \\
    \hline
    \end{tabular}%
    }
    \end{sc}
    \end{small}
    \end{center}
    \caption{Performance of models on Multi Domain Sentiment Dataset, TARGET = Electronics, $k_{fp} = 1$, $k_{fn}=k$ (Value with theoretical threshold)}
    \label{tab:perfMDS_electronics_1}
\end{table}

\begin{table}[!htbp]
    \begin{center}
    \begin{small}
    \begin{sc}
    \scalebox{0.7}{%
    \centering
    \begin{tabular}{lllllll}
    \hline
    \multirow{2}{*}{\textbf{Model}} & \multirow{2}{*}{\textbf{Accuracy}} &  \multicolumn{5}{c}{\textbf{Value}}  \\
    & & k=1 & k=2 & k=4 & k=8 & k=10 \\
    \hline
      LogReg & 0.762 & 0.524 & 0.339 & 0.162 & 0.053 & 0.033 \\
      MLP1 & 0.749 & 0.497 & 0.327 & 0.18 & \textbf{0.081} & \textbf{0.062} \\
      MLP4 & 0.735 & 0.47 & 0.24 & -0.143 & -0.78 & -1.06 \\
      mttri & 0.808 & 0.616 & 0.441 & 0.148 & -0.354 & -0.58 \\
      T5 &  0.784 & 0.568 & 0.352 & -0.08 & -0.944 & -1.376\\
      SieBERT & \textbf{0.842} & \textbf{0.685} & \textbf{0.527} & \textbf{0.217} & -0.397 & -0.705
\\
    \hline
    \end{tabular}%
    }
    \end{sc}
    \end{small}
    \end{center}
    \caption{Performance of models on Multi Domain Sentiment Dataset, TARGET = Electronics, $k_{fp}=k_{fn}=k$ (Value with theoretical threshold)}
    \label{tab:perfMDS_electronics}
\end{table}

\begin{table}[!htbp]
    \begin{center}
    \begin{small}
    \begin{sc}
    \scalebox{0.7}{%
    \centering
    \begin{tabular}{lllllll}
    \hline
    \multirow{2}{*}{\textbf{Model}} & \multirow{2}{*}{\textbf{Accuracy}} &  \multicolumn{5}{c}{\textbf{Value}}  \\
    & & k=1 & k=2 & k=4 & k=8 & k=10 \\
    \hline
      LogReg & 0.782 & 0.565 & 0.466 & 0.365 & 0.306 & 0.295 \\
      MLP1 & 0.765 & 0.53 & 0.433 & 0.339 & 0.292 & 0.279 \\
      MLP4 & 0.761 & 0.521 & 0.416 & 0.263 & 0.026 & -0.076 \\
      mttri & 0.821 & 0.642 & 0.589 & 0.503 & \textbf{0.376} & \textbf{0.31} \\
      T5 & 0.777 & 0.555 & 0.427 & 0.172 & -0.338 & -0.594 \\
      SieBERT & \textbf{0.865} & \textbf{0.73} & \textbf{0.644} & \textbf{0.477} & 0.147 & -0.018 \\
    \hline
    \end{tabular}%
    }
    \end{sc}
    \end{small}
    \end{center}
    \caption{Performance of models on Multi Domain Sentiment Dataset, TARGET = Kitchen, $k_{fp} = 1$, $k_{fn}=k$ (Value with theoretical threshold) }
    \label{tab:perfMDS_kitchen_1}
\end{table}

\begin{table}[!htbp]
    \begin{center}
    \begin{small}
    \begin{sc}
    \scalebox{0.7}{%
    \centering
    \begin{tabular}{lllllll}
    \hline
    \multirow{2}{*}{\textbf{Model}} & \multirow{2}{*}{\textbf{Accuracy}} &  \multicolumn{5}{c}{\textbf{Value}}  \\
    & & k=1 & k=2 & k=4 & k=8 & k=10 \\
    \hline
      LogReg & 0.782 & 0.565 & 0.374 & 0.176 & 0.06 & 0.034 \\
      MLP1 & 0.765 & 0.53 & 0.337 & 0.164 & \textbf{0.07} & \textbf{0.044}\\
      MLP4 & 0.761 & 0.521 & 0.312 & 0.003 & -0.478 & -0.685\\
      mttri & 0.821 & 0.642 & 0.489 & 0.235 & -0.192 & -0.384 \\
      T5 &  0.777 & 0.555 & 0.332 & -0.113 & -1.004 & -1.449 \\
      SieBERT & \textbf{0.865} & \textbf{0.73} & \textbf{0.595} & \textbf{0.328} & -0.195 & -0.454 \\
    \hline
    \end{tabular}%
    }
    \end{sc}
    \end{small}
    \end{center}
    \caption{Performance of models on Multi Domain Sentiment Dataset, TARGET = Kitchen, $k_{fp}=k_{fn}=k$ (Value with theoretical threshold) }
    \label{tab:perfMDS_kitchen}
\end{table}

\begin{table}[!htbp]
    \begin{center}
    \begin{small}
    \begin{sc}
    \scalebox{0.6}{%
    \centering
    \begin{tabular}{llllll}
    \hline
    & & \multicolumn{4}{c}{\textbf{Source}} \\
     &  &    \textbf{DVD} &  \textbf{Books} & \textbf{Electronics} & \textbf{Kitchen} \\
    \hline
    \multirow{4}{*}{\textbf{Target}} & \multicolumn{1}{|c}{\textbf{DVD}}         &    -    &  \textbf{0.782} & 0.716 & 0.723  \\
    & \multicolumn{1}{|c}{\textbf{Books}}       & \textbf{0.718}   &   -   & 0.694 & 0.7  \\
    & \multicolumn{1}{|c}{\textbf{Electronics}} & 0.731 & 0.723  &       -      &  \textbf{0.831}  \\
    & \multicolumn{1}{|c}{\textbf{Kitchen}}     & 0.762 & 0.746 & \textbf{0.839}  & -  \\
    \hline
    \end{tabular}%
    }
    \end{sc}
    \end{small}
    \end{center}
    \caption{Accuracy of LogReg model on Multi Domain Sentiment Dataset.}
    \label{tab:accMDS_LogReg}
\end{table}

\begin{table}[!htbp]
    \begin{center}
    \begin{small}
    \begin{sc}
    \scalebox{0.6}{%
    \centering
    \begin{tabular}{llllll}
    \hline
    & & \multicolumn{4}{c}{\textbf{Source}} \\
     &  &    \textbf{DVD} &  \textbf{Books} & \textbf{Electronics} & \textbf{Kitchen} \\
    \hline
    \multirow{4}{*}{\textbf{Target}} &
    \multicolumn{1}{|c}{\textbf{DVD}}         &    -    & \textbf{0.761} & 0.704 & 0.72 \\
    & \multicolumn{1}{|c}{\textbf{Books}}       &   \textbf{0.711} &   -   & 0.68  &  0.683  \\
    & \multicolumn{1}{|c}{\textbf{Electronics}} &  0.712 & 0.706 &       -      &  \textbf{0.828}  \\
    & \multicolumn{1}{|c}{\textbf{Kitchen}}     & 0.743 & 0.722 & \textbf{0.83}    & -        \\
    \hline
    \end{tabular}%
    }
    \end{sc}
    \end{small}
    \end{center}
    \caption{Accuracy of MLP1 model on Multi Domain Sentiment Dataset.}
    \label{tab:accMDS_MLP1}
\end{table}

\begin{table}[!htbp]
    \begin{center}
    \begin{small}
    \begin{sc}
    \scalebox{0.6}{%
    \centering
    \begin{tabular}{llllll}
    \hline
    & & \multicolumn{4}{c}{\textbf{Source}} \\
     &  &    \textbf{DVD} &  \textbf{Books} & \textbf{Electronics} & \textbf{Kitchen} \\
    \hline
    \multirow{4}{*}{\textbf{Target}} & \multicolumn{1}{|c}{\textbf{DVD}}         &    -    & \textbf{0.763} & 0.692 & 0.704  \\
    & \multicolumn{1}{|c}{\textbf{Books}}       & \textbf{0.714}   &   -   & 0.681 & 0.695  \\
    & \multicolumn{1}{|c}{\textbf{Electronics}} & 0.689 & 0.683 &       -      &  \textbf{0.832}  \\
    & \multicolumn{1}{|c}{\textbf{Kitchen}}     &  0.74 & 0.715 & \textbf{0.827}  & -  \\
    \hline
    \end{tabular}%
    }
    \end{sc}
    \end{small}
    \end{center}
    \caption{Accuracy of MLP4 model on Multi Domain Sentiment Dataset.}
    \label{tab:accMDS_MLP4}
\end{table}

\begin{table}[!htbp]
    \begin{center}
    \begin{small}
    \begin{sc}
    \scalebox{0.6}{%
    \centering
    \begin{tabular}{llllll}
    \hline
    & & \multicolumn{4}{c}{\textbf{Source}} \\
     &  &    \textbf{DVD} &  \textbf{Books} & \textbf{Electronics} & \textbf{Kitchen} \\
    \hline
    \multirow{4}{*}{\textbf{Target}} & \multicolumn{1}{|c}{\textbf{DVD}}         &    -    &  \textbf{0.808} & 0.727 & 0.724     \\
    & \multicolumn{1}{|c}{\textbf{Books}}       &  \textbf{0.753} &   -     &       0.733 &   0.741 \\
    & \multicolumn{1}{|c}{\textbf{Electronics}} &  0.761 & 0.801 &   -  &  \textbf{0.862}\\
    & \multicolumn{1}{|c}{\textbf{Kitchen}}     &  0.828 &  0.777 & \textbf{0.859} & -        \\
    \hline
    \end{tabular}%
    }
    \end{sc}
    \end{small}
    \end{center}
    \caption{Accuracy of mttri model on Multi Domain Sentiment Dataset}
    \label{tab:accMDS_mttri}
\end{table}

\onecolumn
\begin{figure*}[!htbp]
 \centering  
    \includegraphics[width=.245\linewidth]{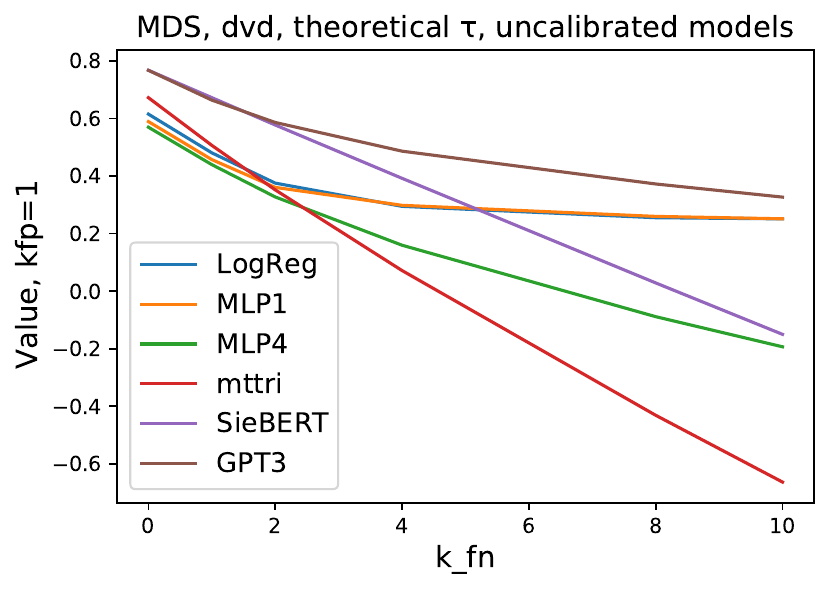} 
    \includegraphics[width=.245\linewidth]{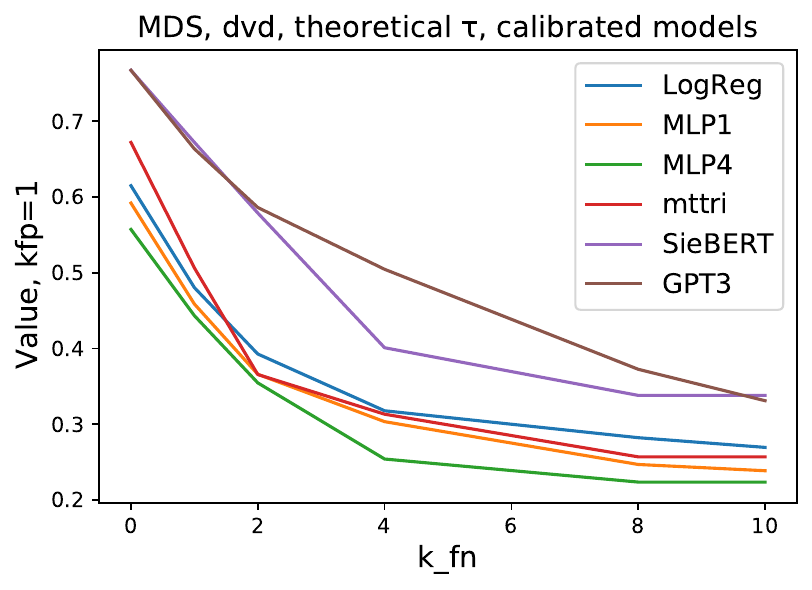} 
    \includegraphics[width=.245\linewidth]{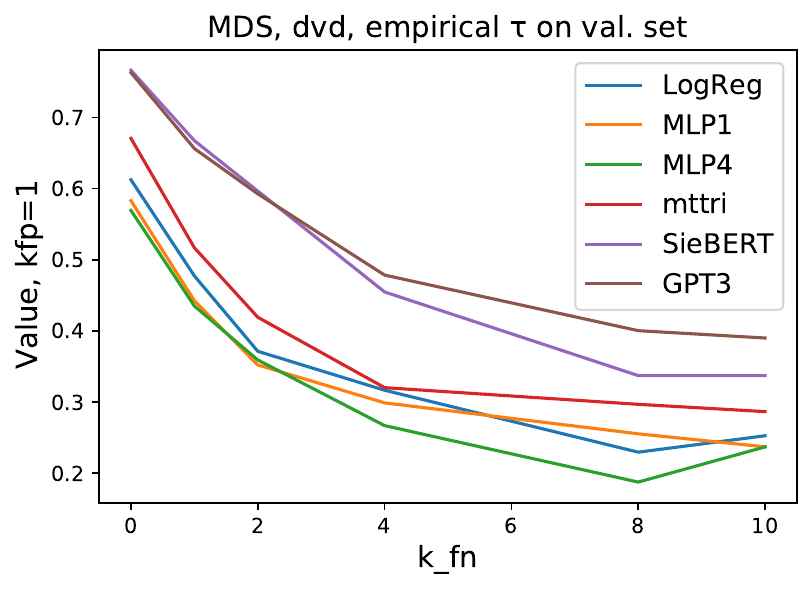} 
    \includegraphics[width=.245\linewidth]{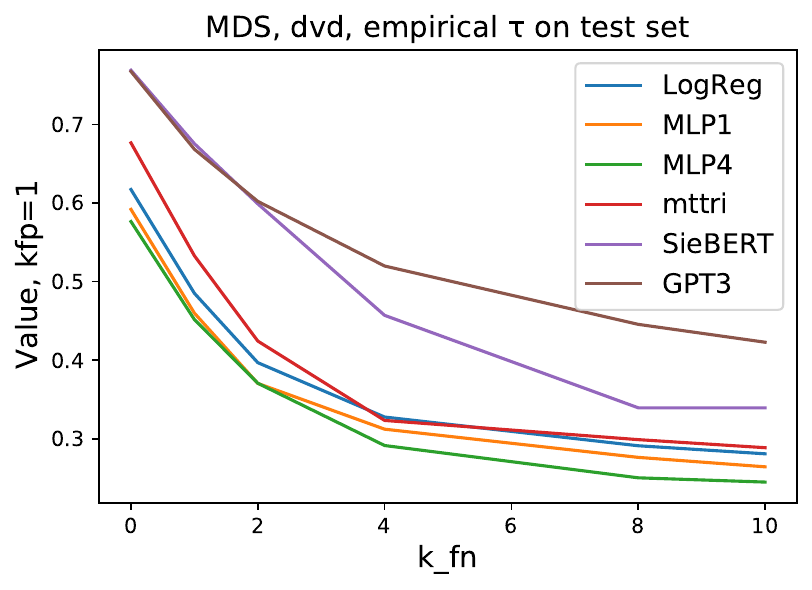} 
    \includegraphics[width=.245\linewidth]{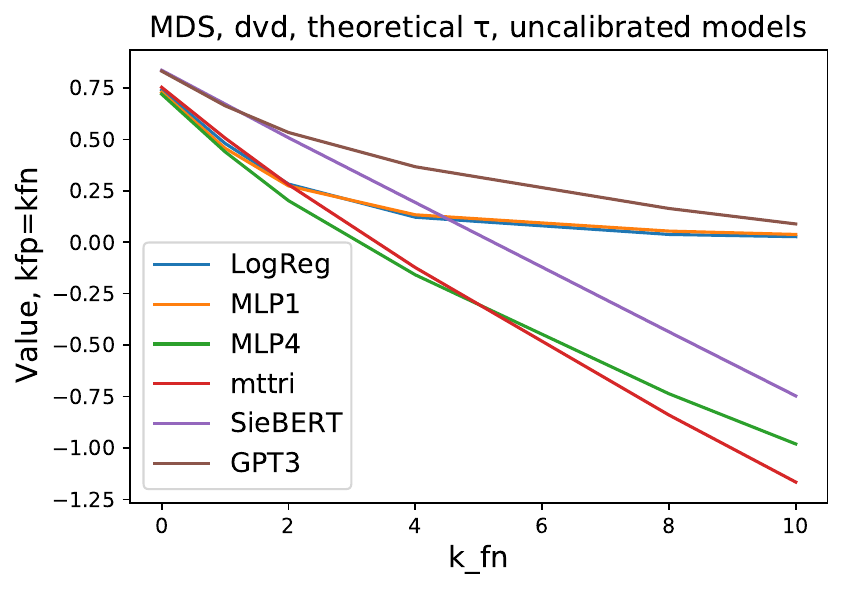} 
    \includegraphics[width=.245\linewidth]{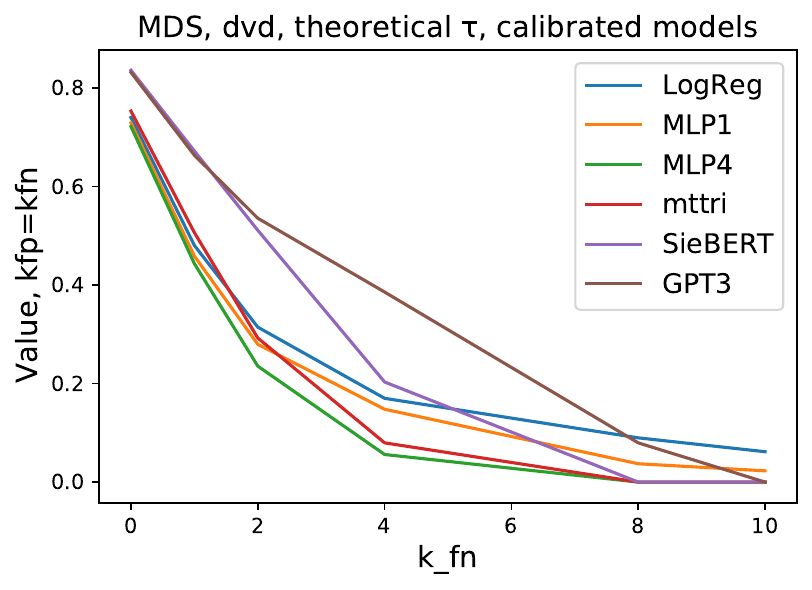} 
    \includegraphics[width=.245\linewidth]{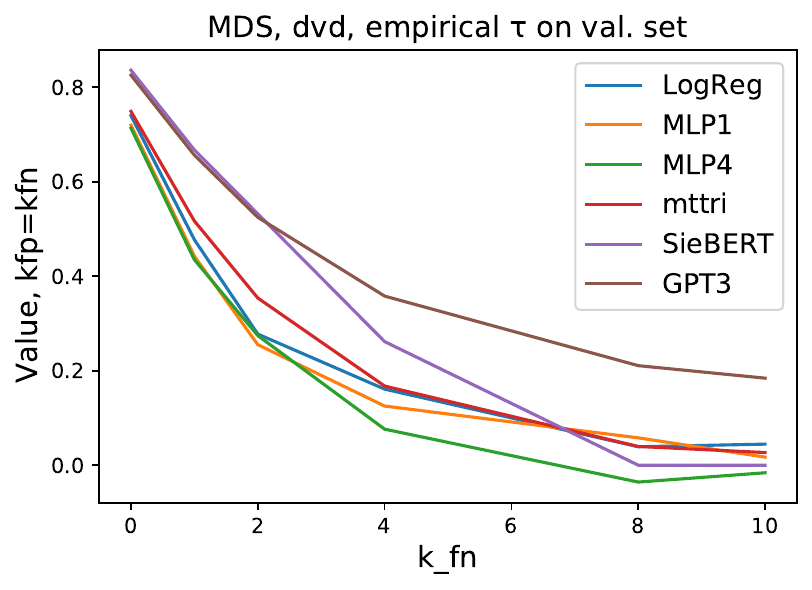} 
    \includegraphics[width=.245\linewidth]{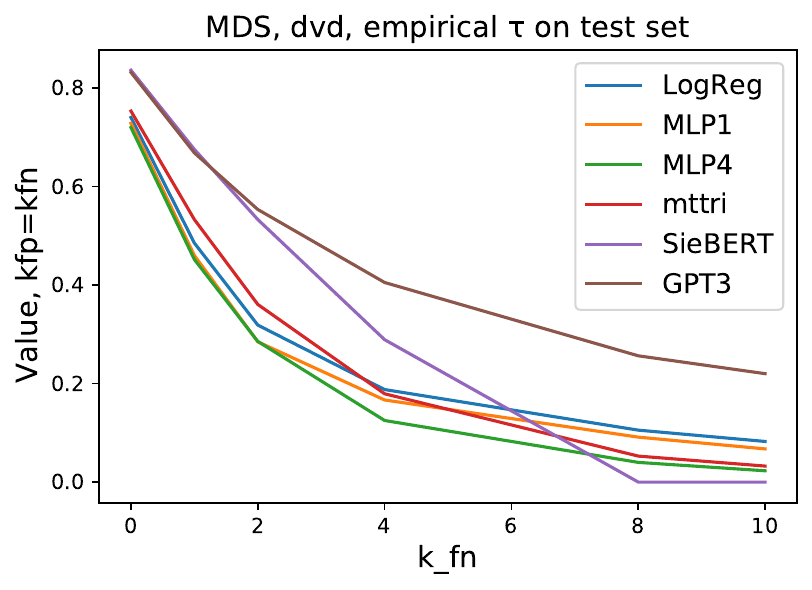} 
    
    \includegraphics[width=.245\linewidth]{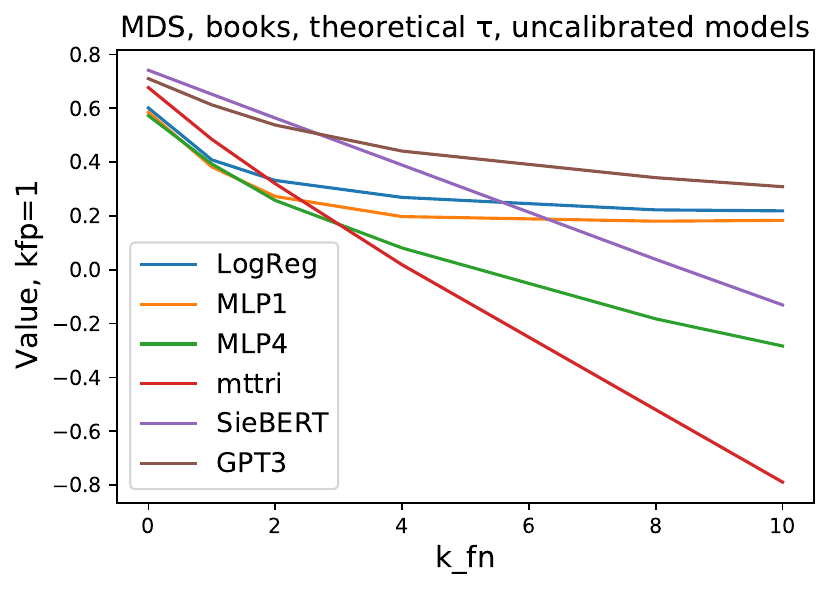} 
    \includegraphics[width=.245\linewidth]{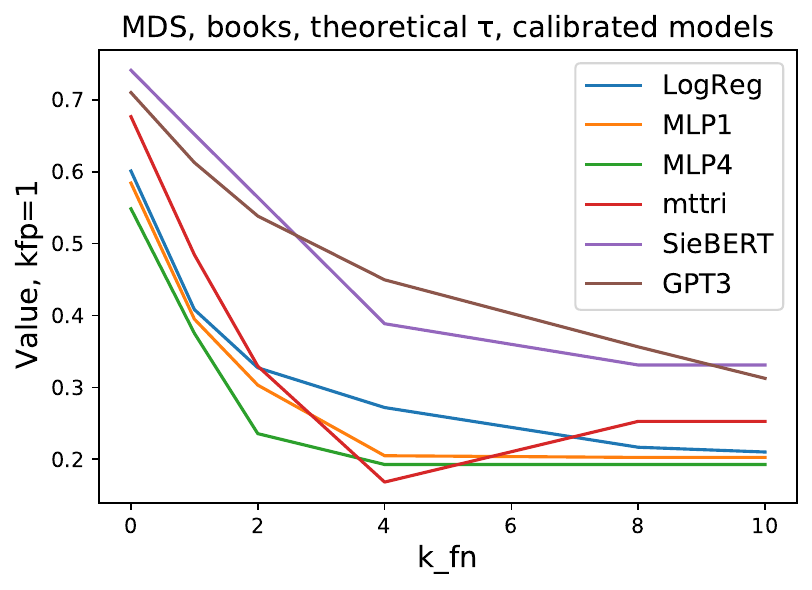} 
    \includegraphics[width=.245\linewidth]{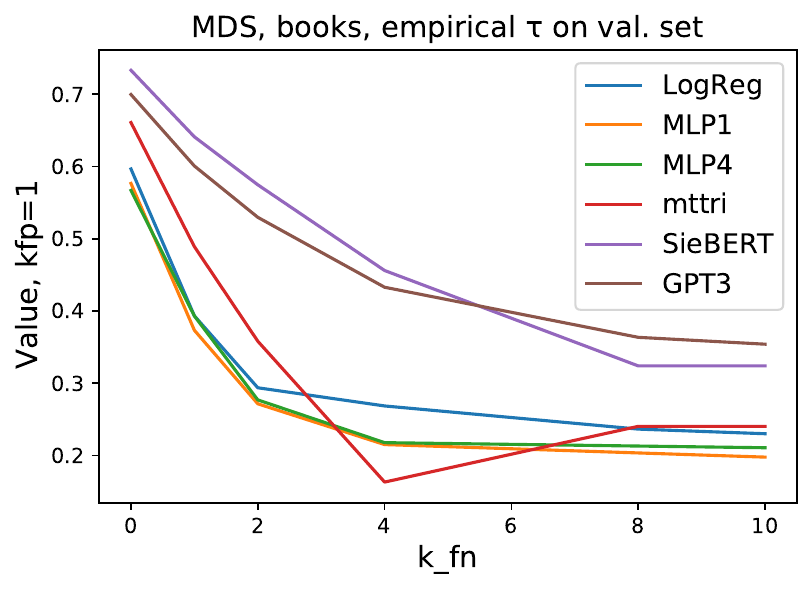} 
    \includegraphics[width=.245\linewidth]{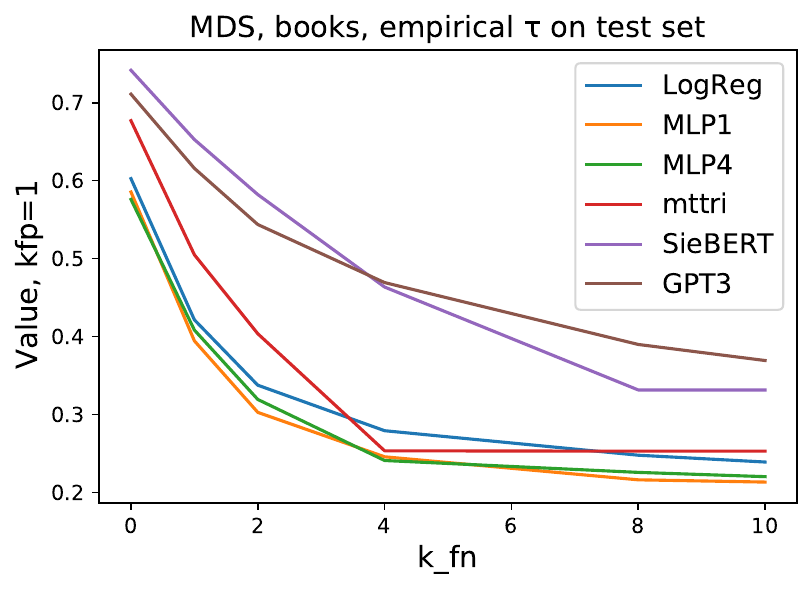} 
    \includegraphics[width=.245\linewidth]{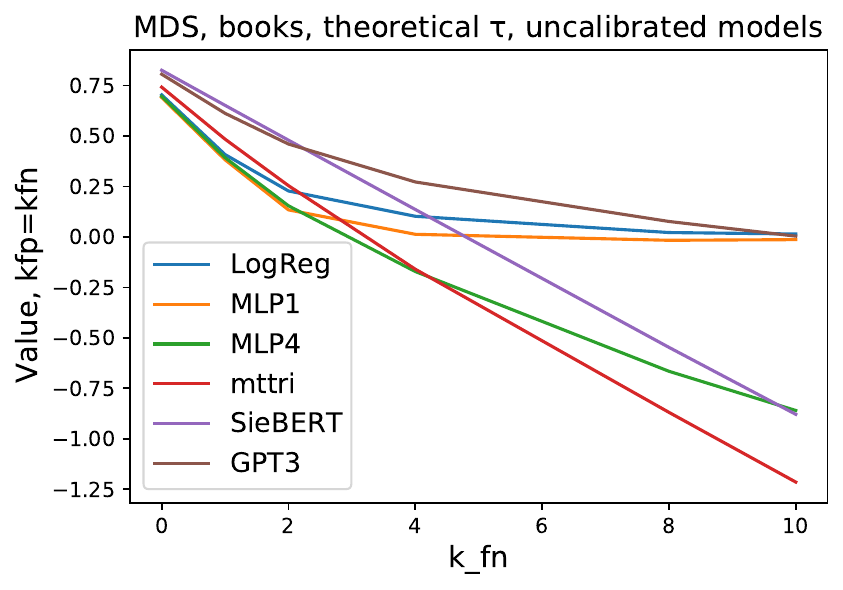} 
    \includegraphics[width=.245\linewidth]{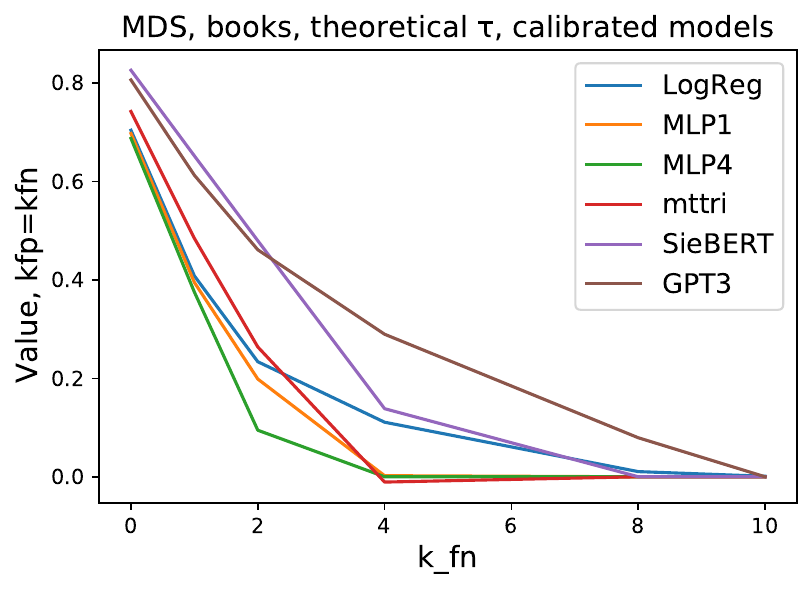} 
    \includegraphics[width=.245\linewidth]{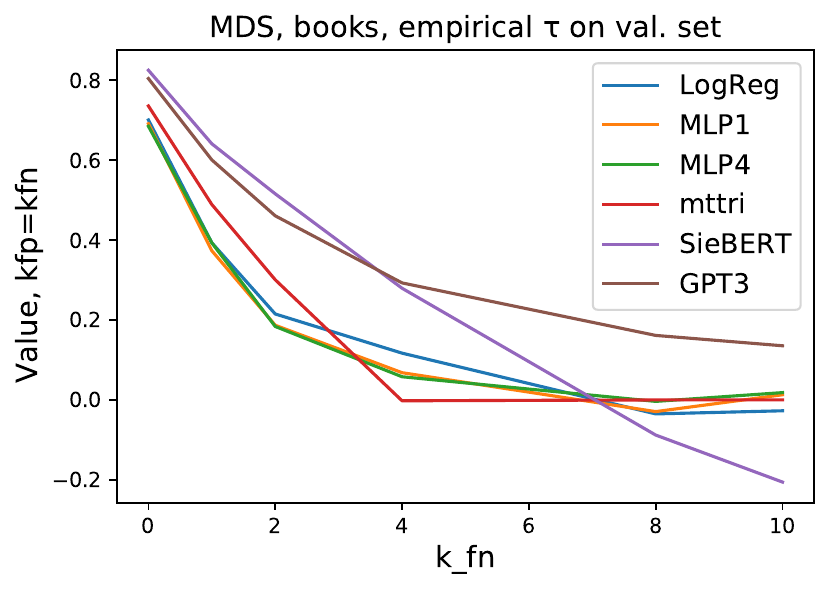} 
    \includegraphics[width=.245\linewidth]{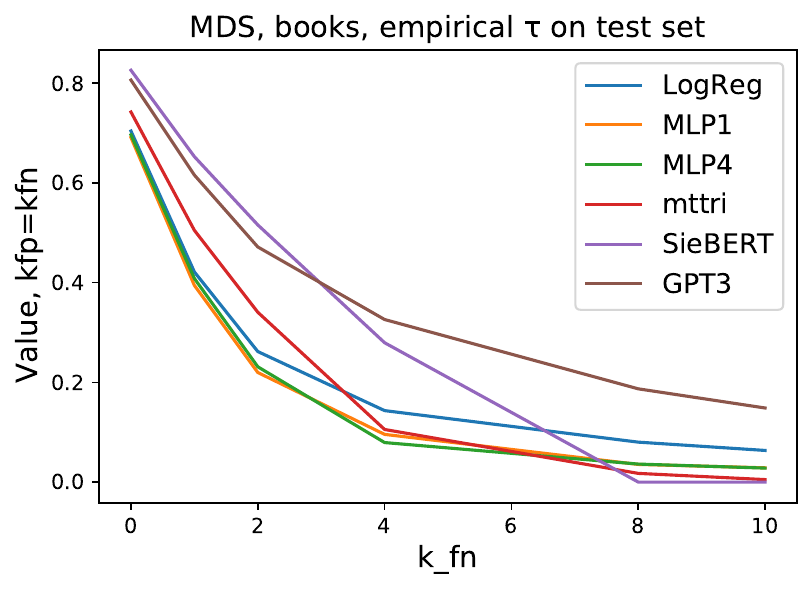} 
    
    \includegraphics[width=.245\linewidth]{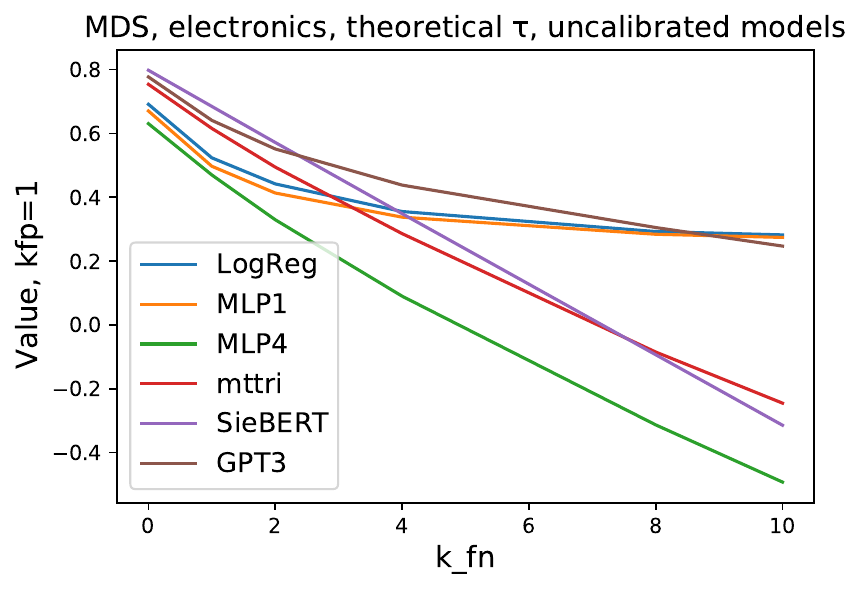} 
    \includegraphics[width=.245\linewidth]{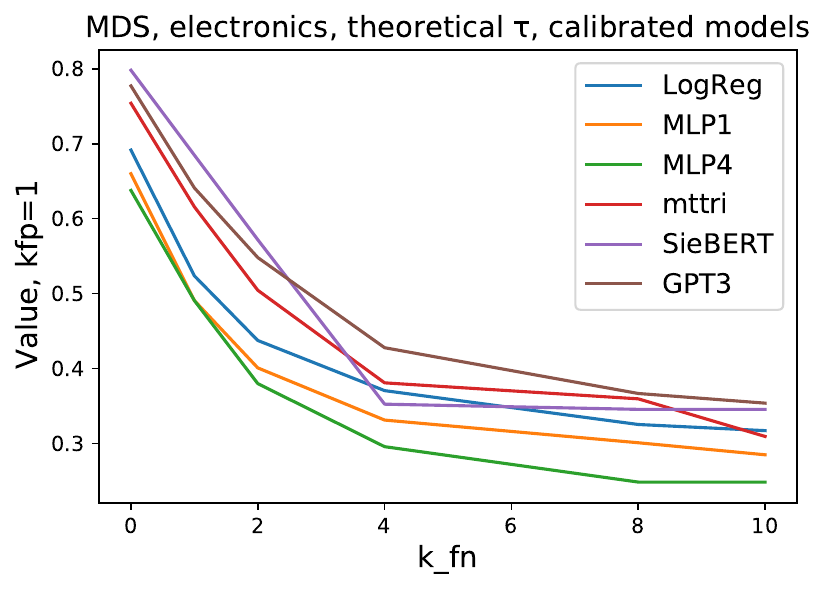} 
    \includegraphics[width=.245\linewidth]{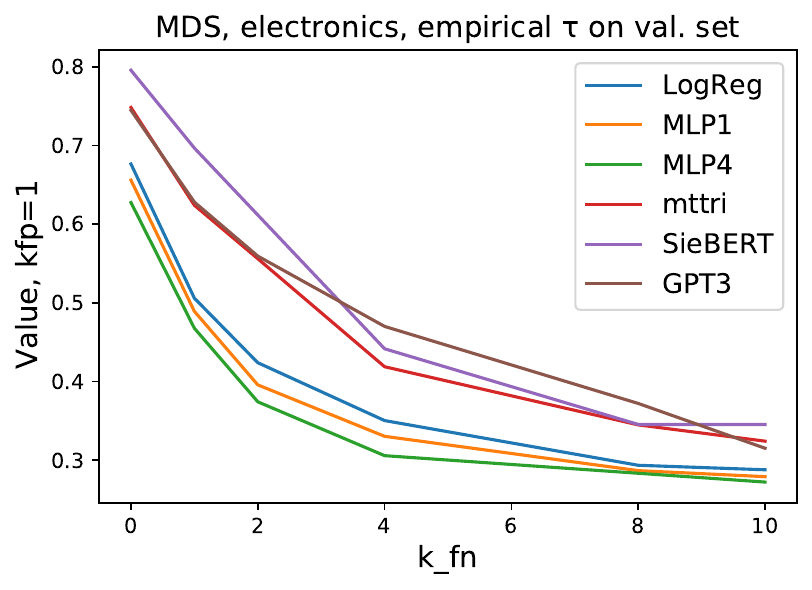} 
    \includegraphics[width=.245\linewidth]{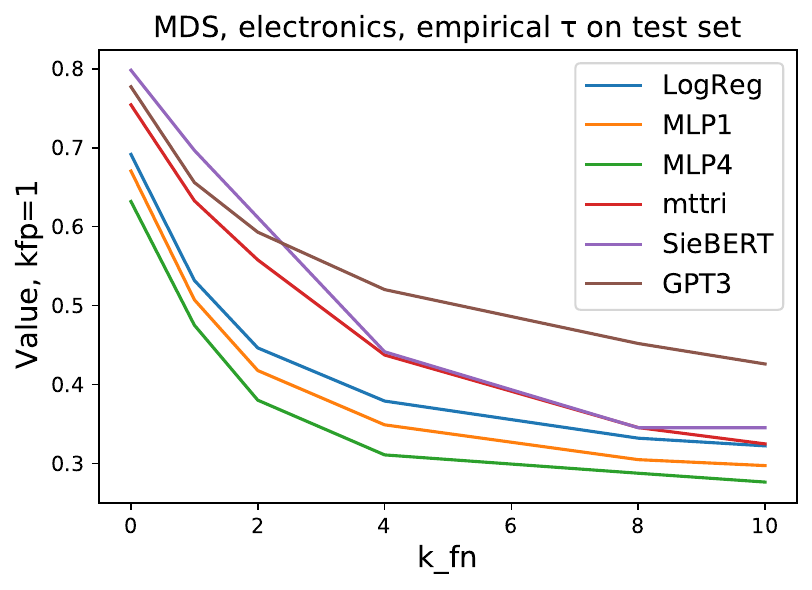} 
    \includegraphics[width=.245\linewidth]{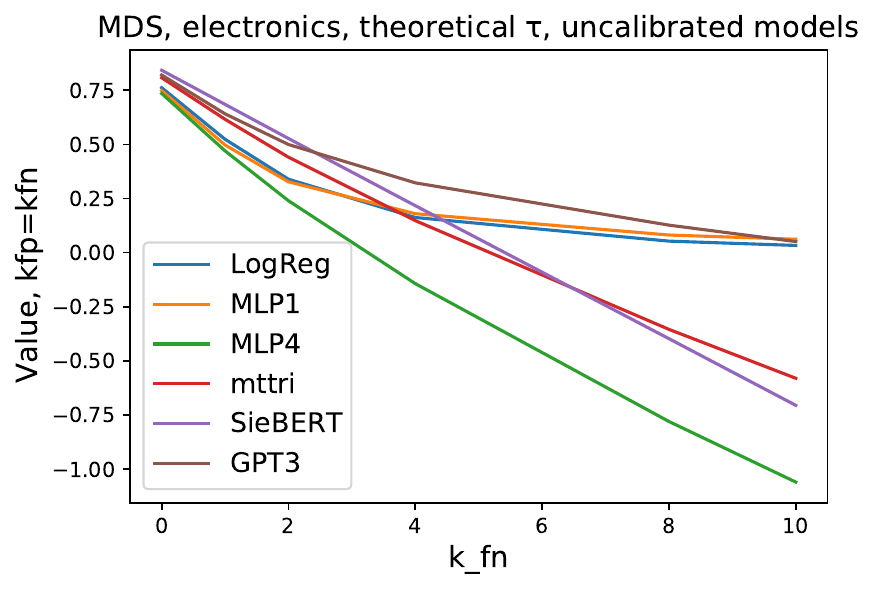} 
    \includegraphics[width=.245\linewidth]{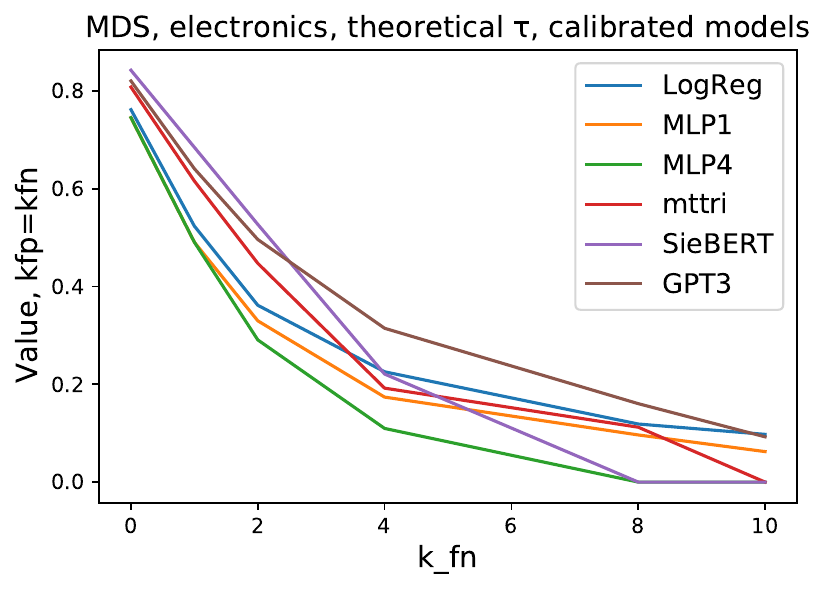} 
    \includegraphics[width=.245\linewidth]{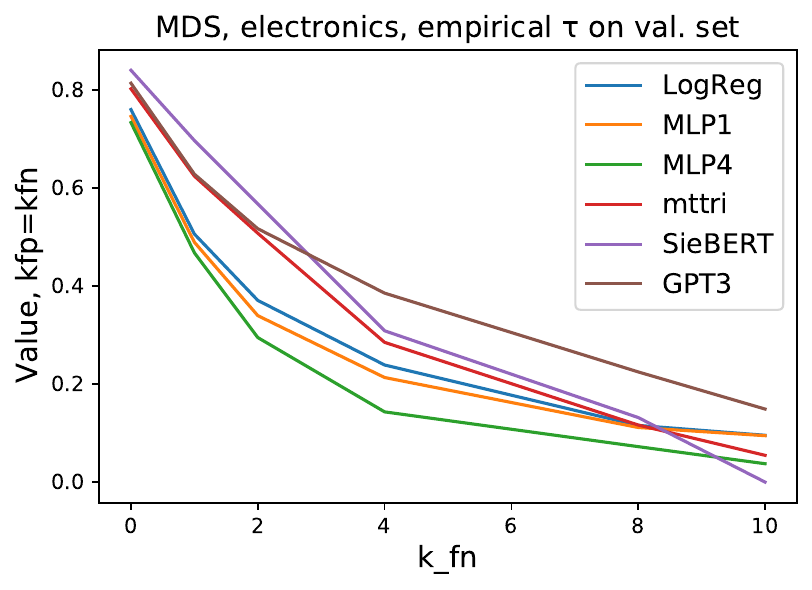} 
    \includegraphics[width=.245\linewidth]{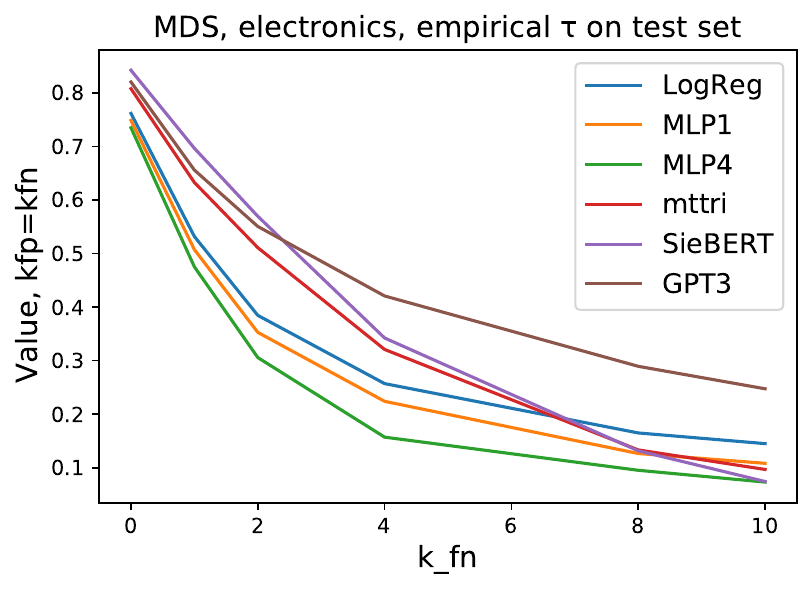}
    
    \includegraphics[width=.245\linewidth]{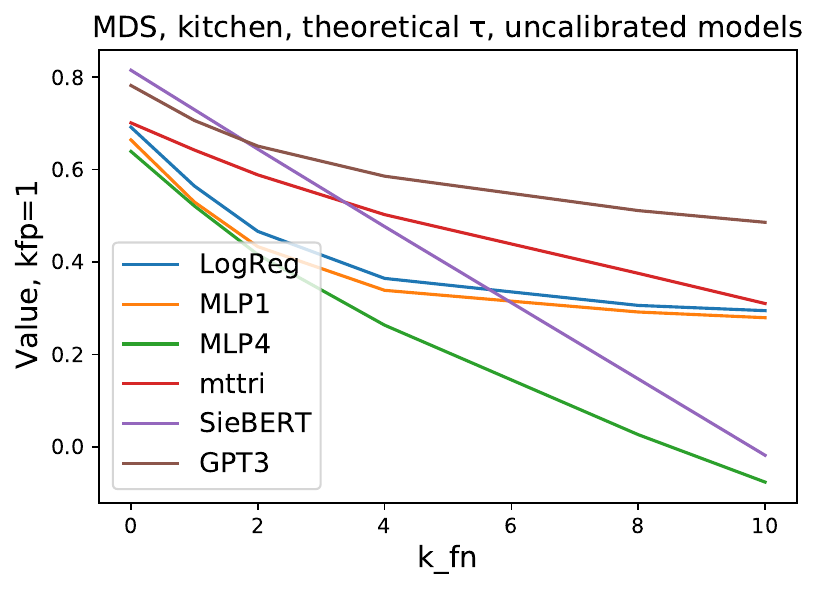} 
    \includegraphics[width=.245\linewidth]{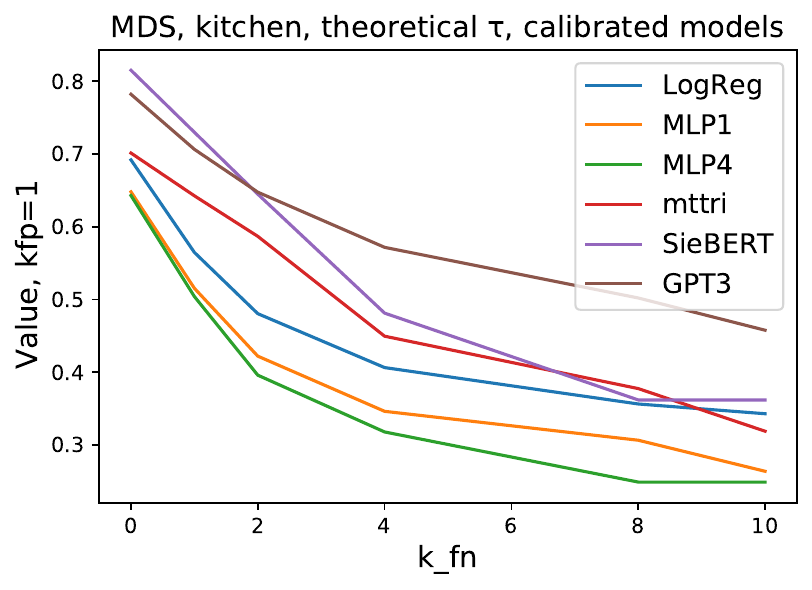} 
    \includegraphics[width=.245\linewidth]{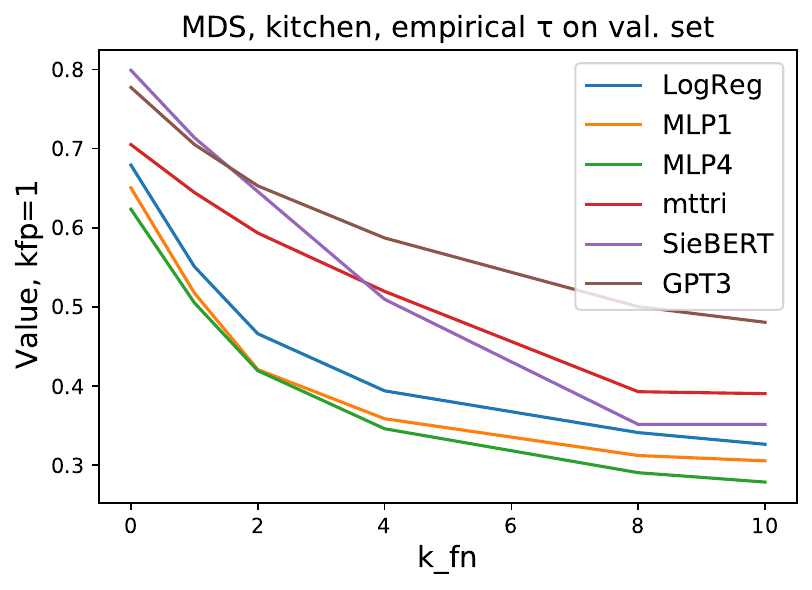} 
    \includegraphics[width=.245\linewidth]{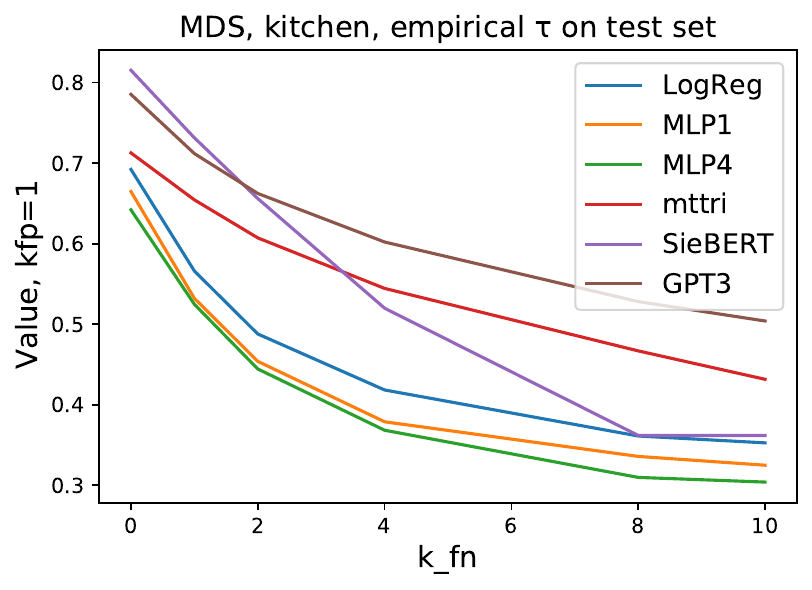} 
    \includegraphics[width=.245\linewidth]{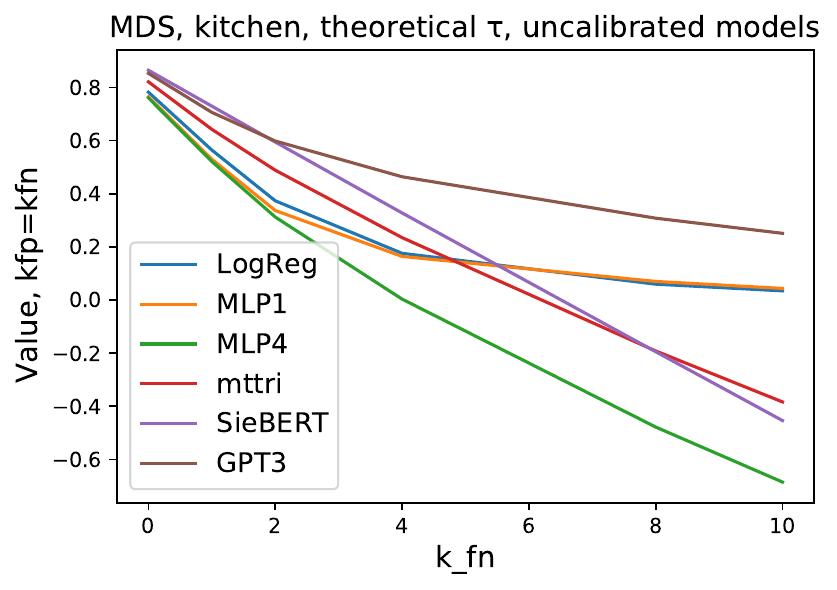} 
    \includegraphics[width=.245\linewidth]{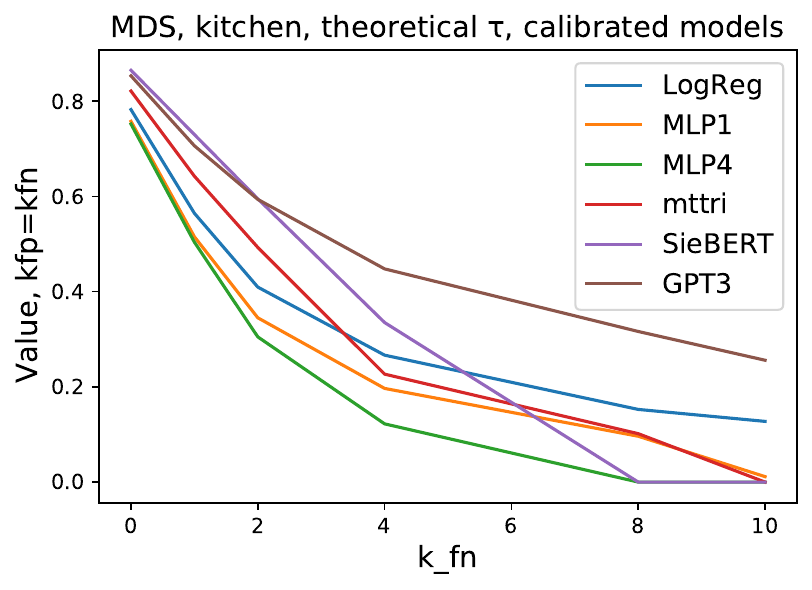} 
    \includegraphics[width=.245\linewidth]{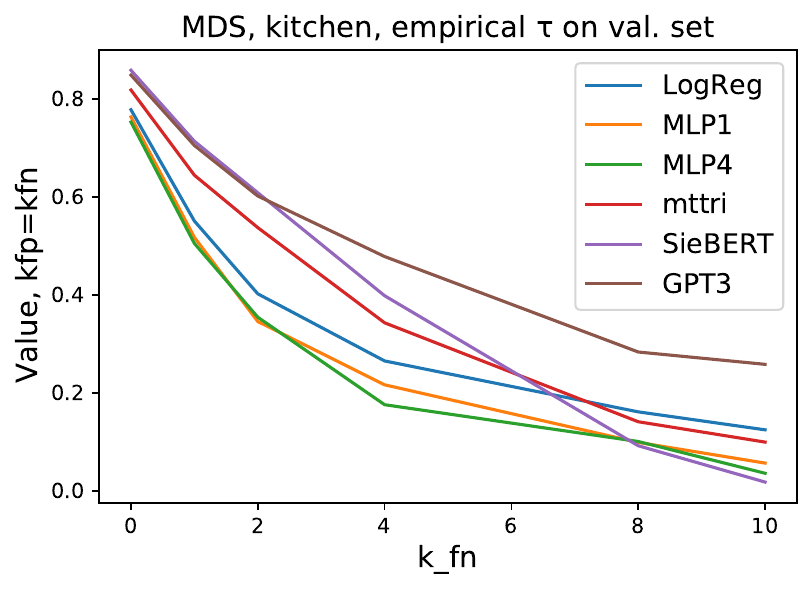} 
    \includegraphics[width=.245\linewidth]{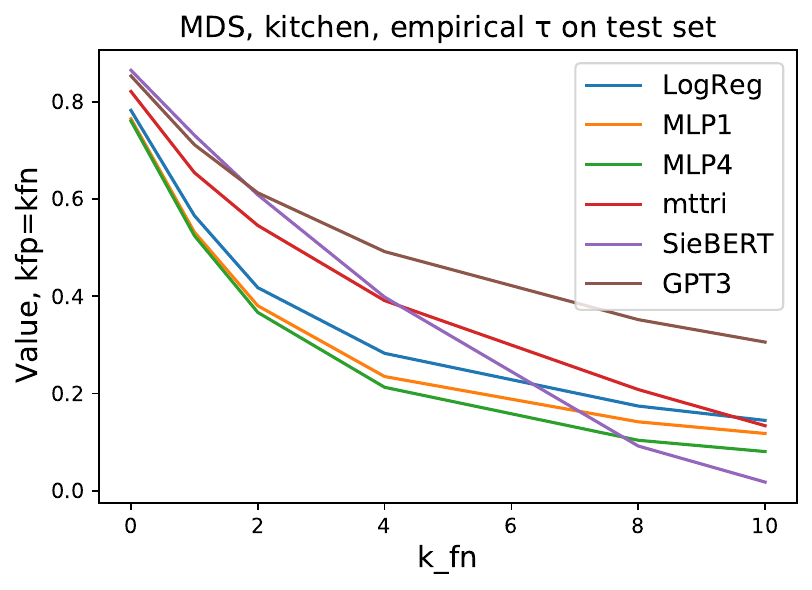}
  
    \caption{\label{fig:app:MDS_value_avg_gpt}Value curves on Multi Domain Sentiment dataset for increasing $k_{fn}$, Values are averaged for simple models, the 'mttri' model, and GPT-3.}
\end{figure*}%%

\begin{figure*}[!htbp]
 \centering  
    \includegraphics[width=.245\linewidth]{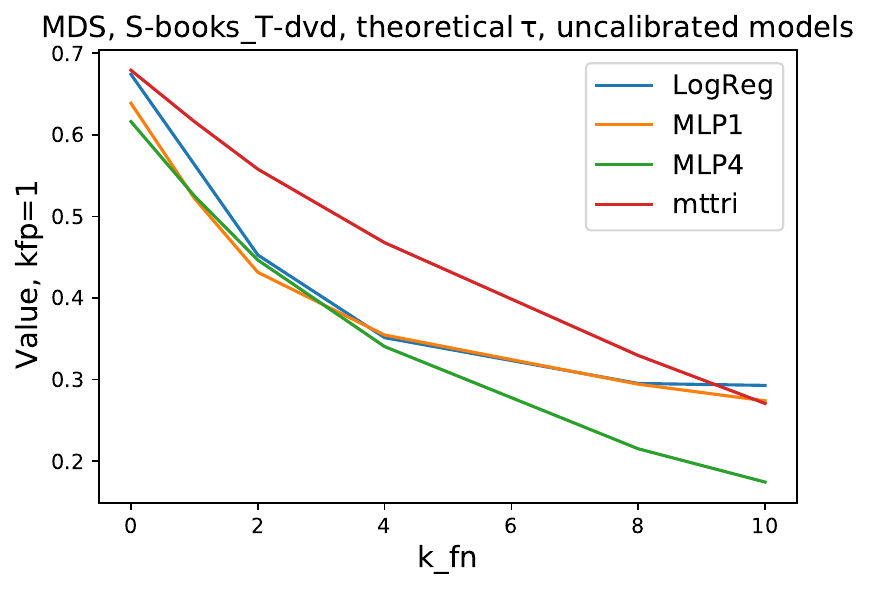} 
    \includegraphics[width=.245\linewidth]{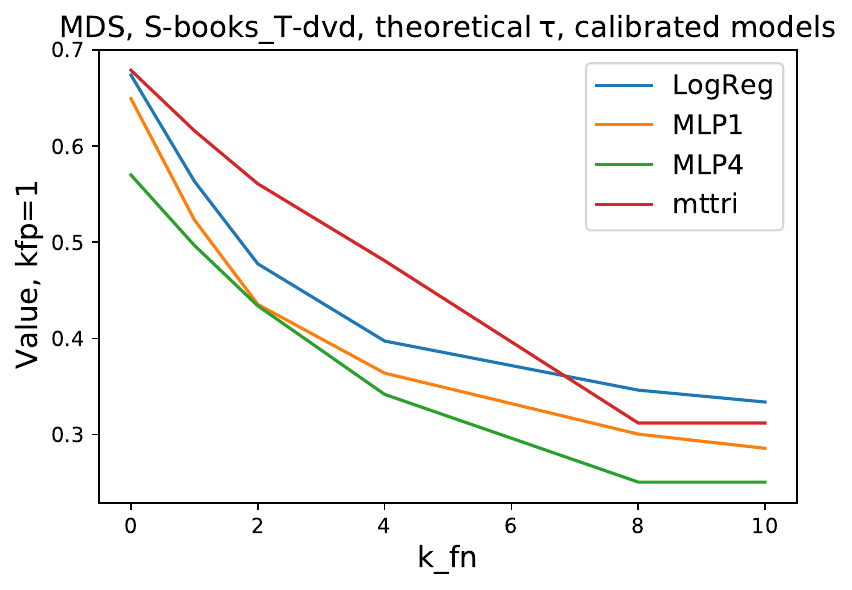}
    \includegraphics[width=.245\linewidth]{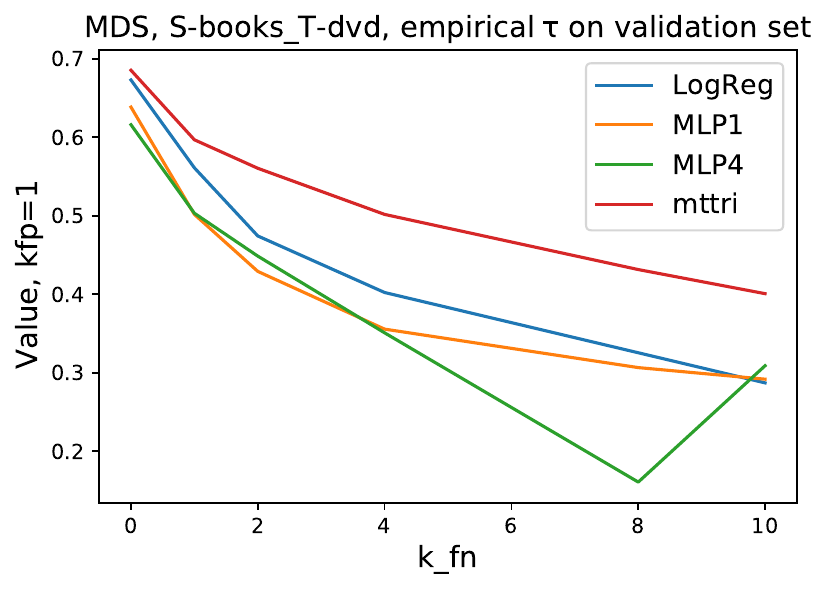}
    \includegraphics[width=.245\linewidth]{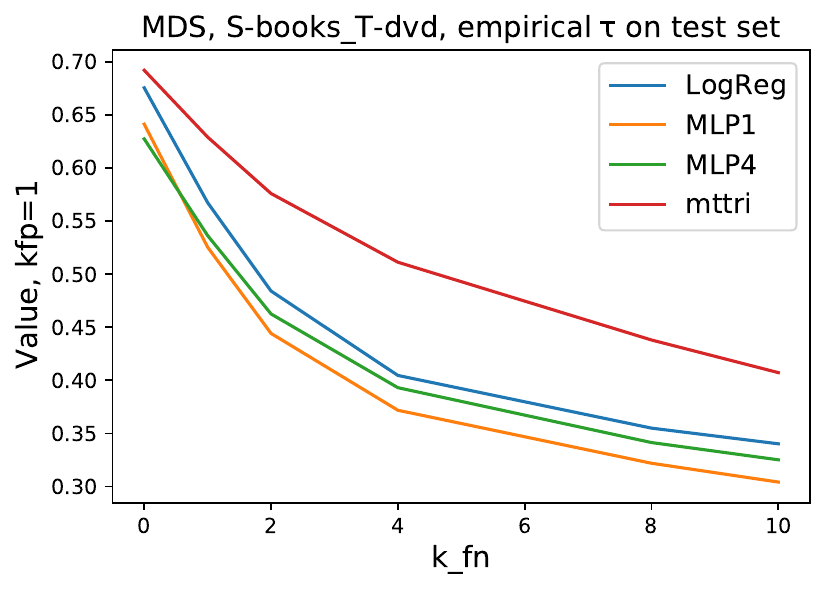}
    \includegraphics[width=.245\linewidth]{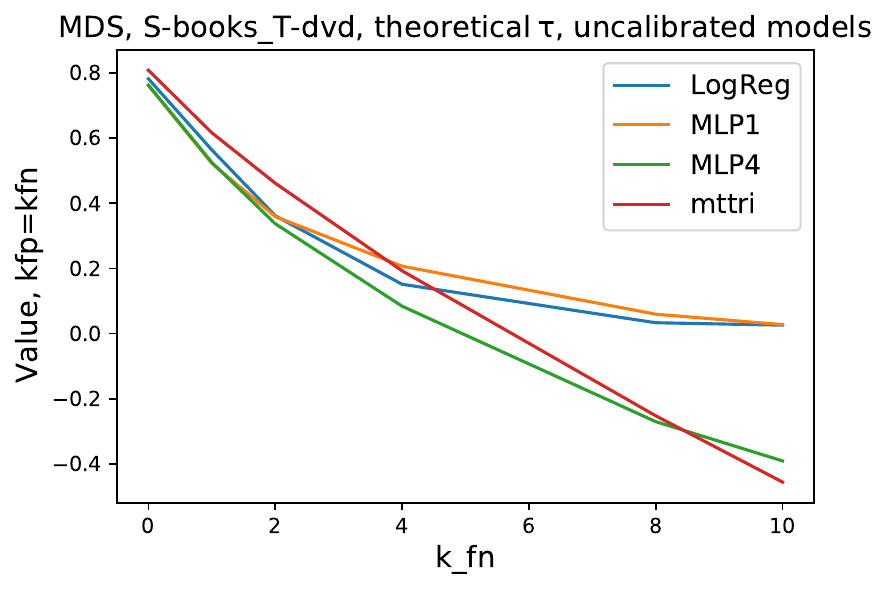} 
    \includegraphics[width=.245\linewidth]{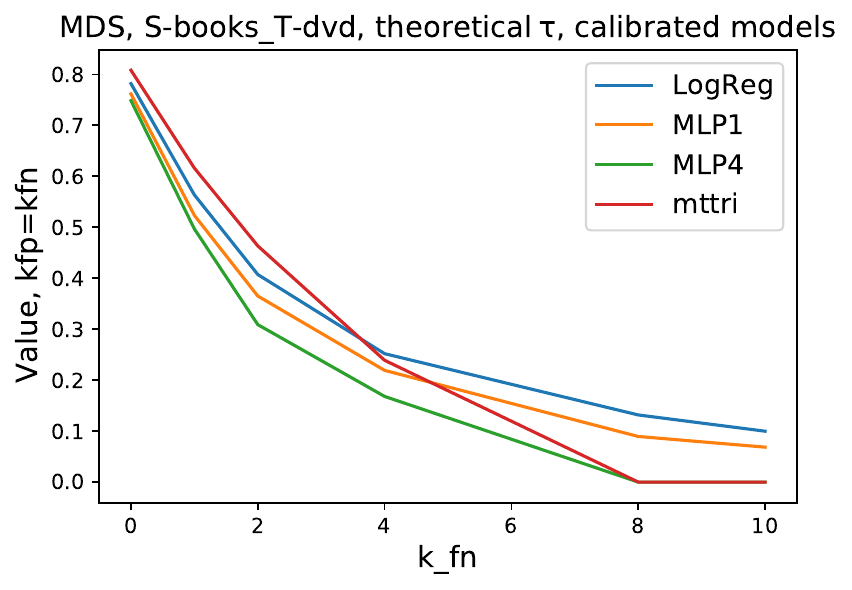}
    \includegraphics[width=.245\linewidth]{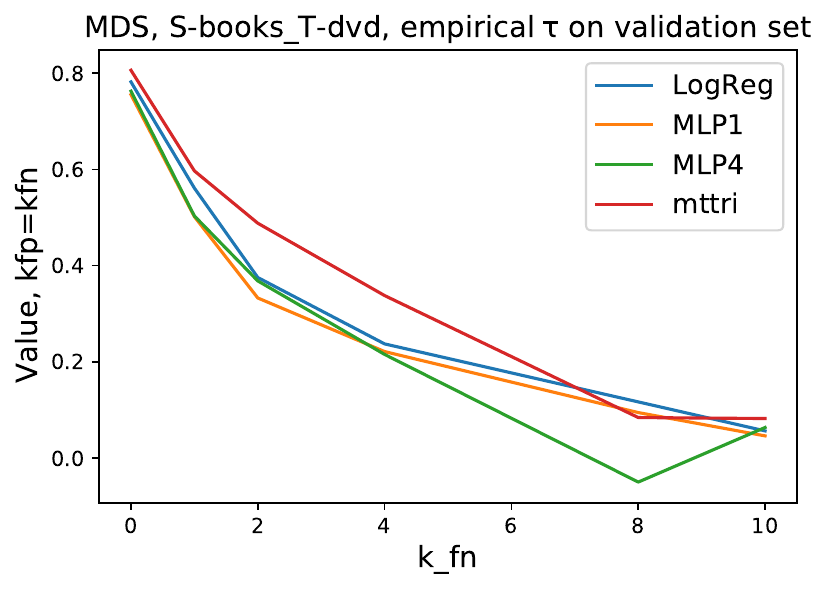}
    \includegraphics[width=.245\linewidth]{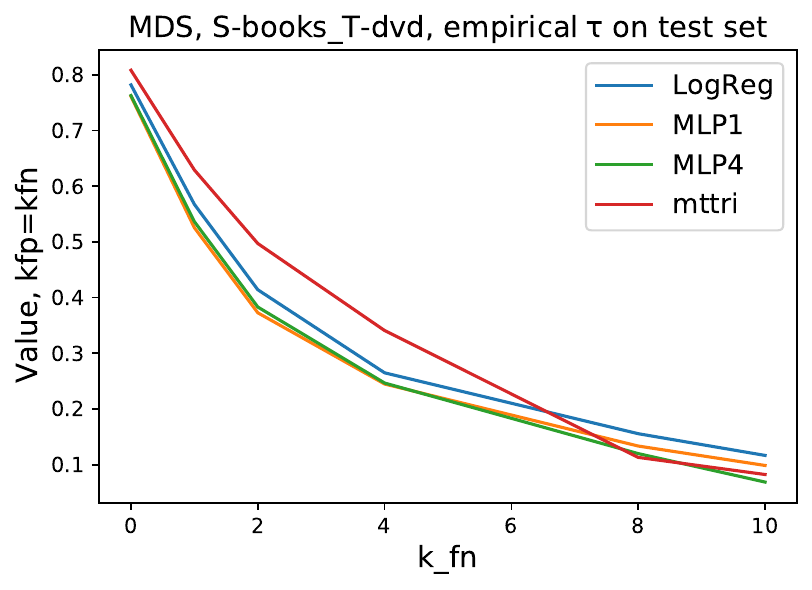}
    
    \includegraphics[width=.245\linewidth]{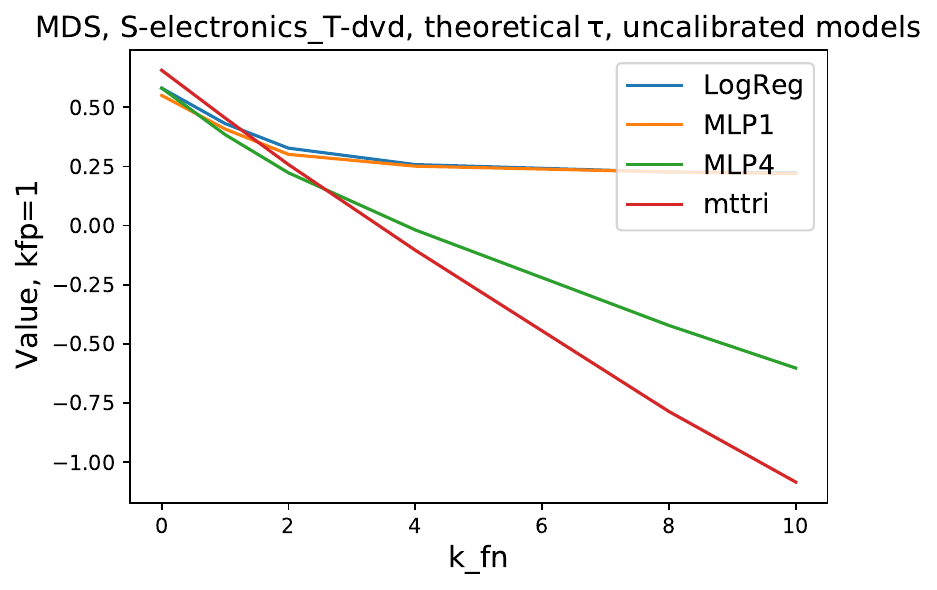} 
    \includegraphics[width=.245\linewidth]{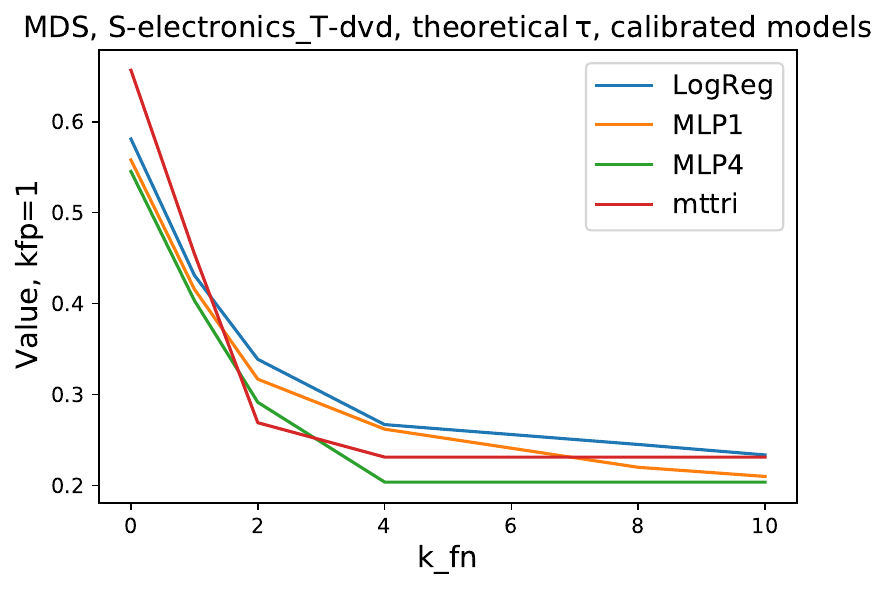}
    \includegraphics[width=.245\linewidth]{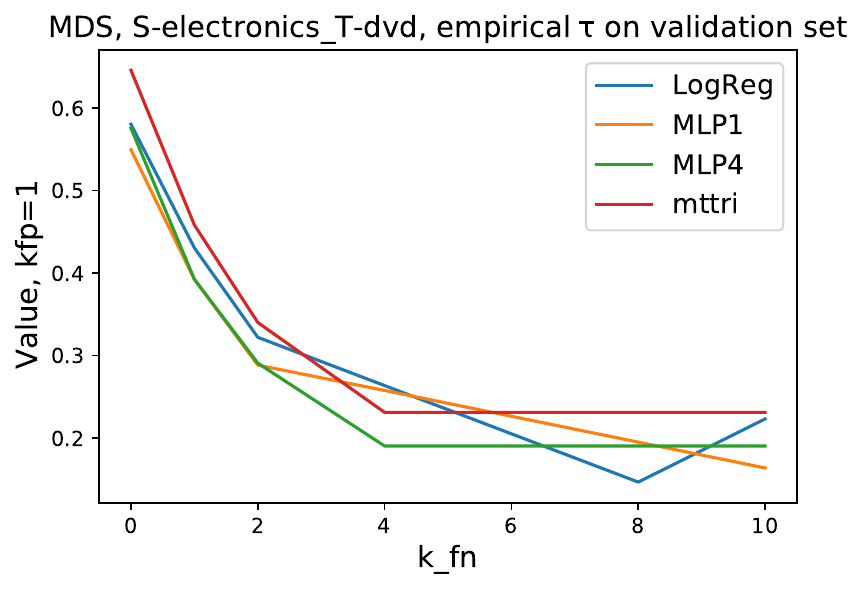}
    \includegraphics[width=.245\linewidth]{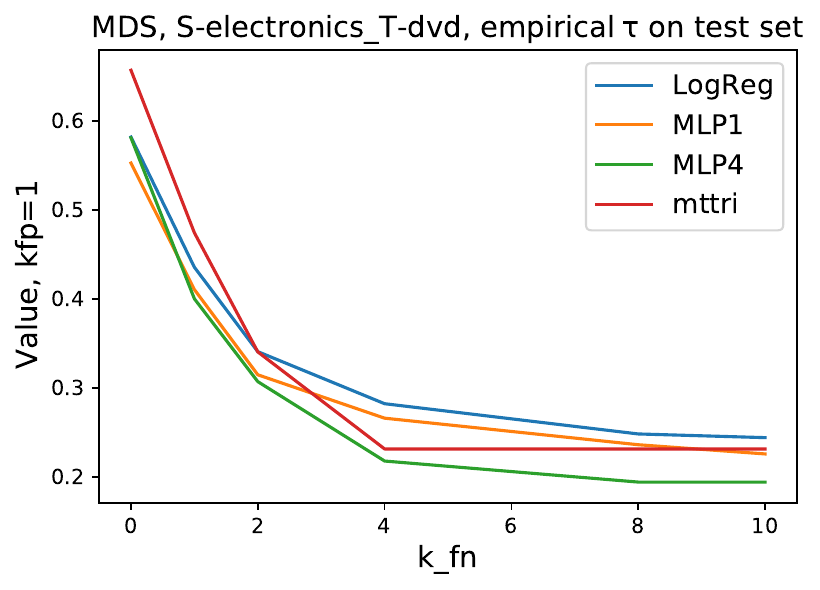}
    \includegraphics[width=.245\linewidth]{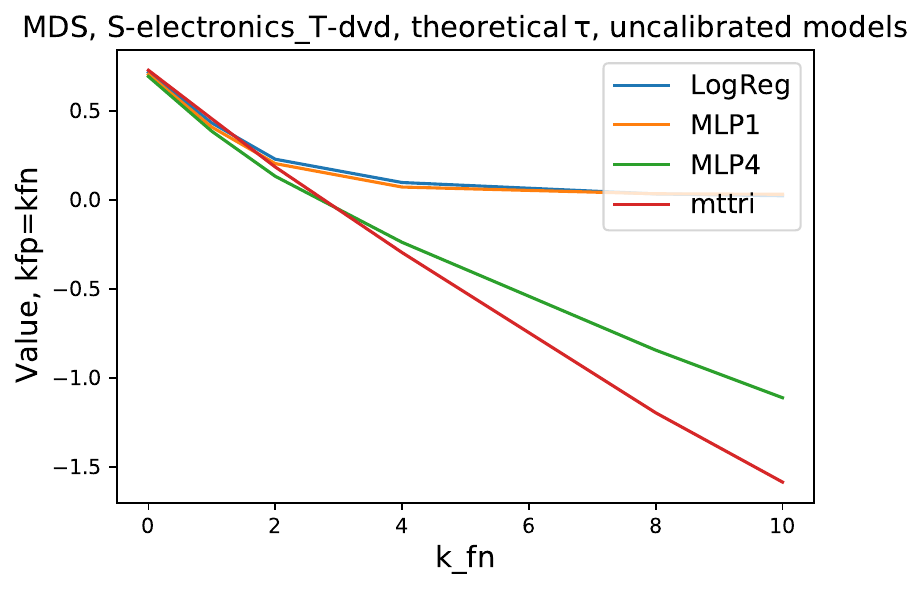} 
    \includegraphics[width=.245\linewidth]{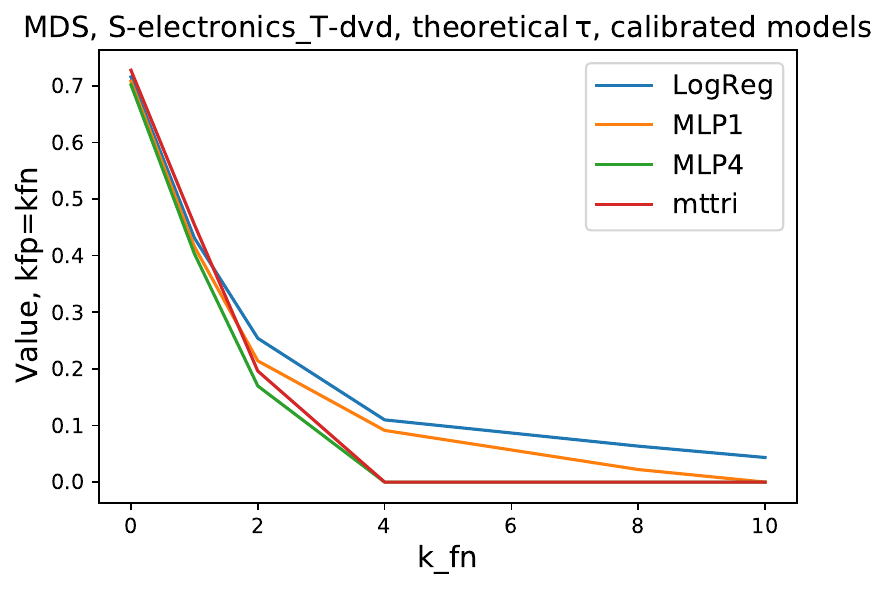}
    \includegraphics[width=.245\linewidth]{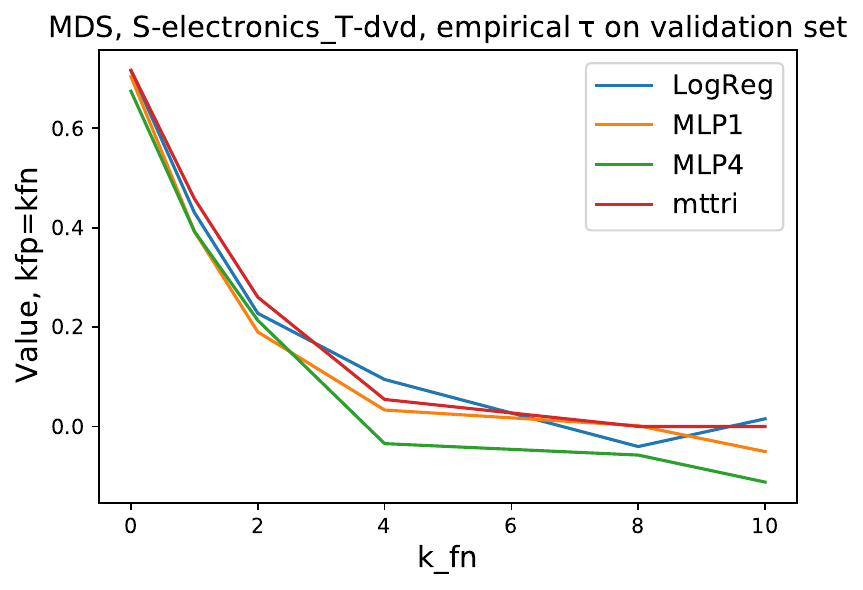}
    \includegraphics[width=.245\linewidth]{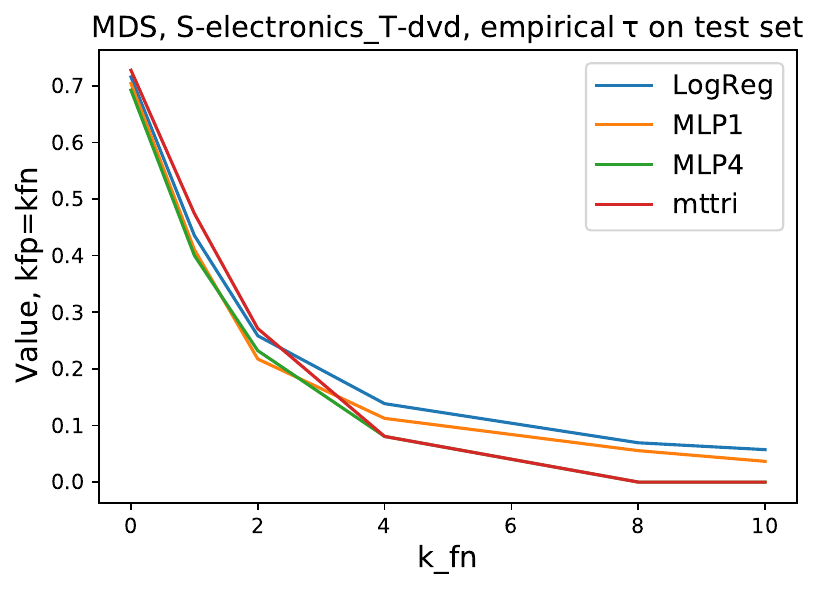}
    
    \includegraphics[width=.245\linewidth]{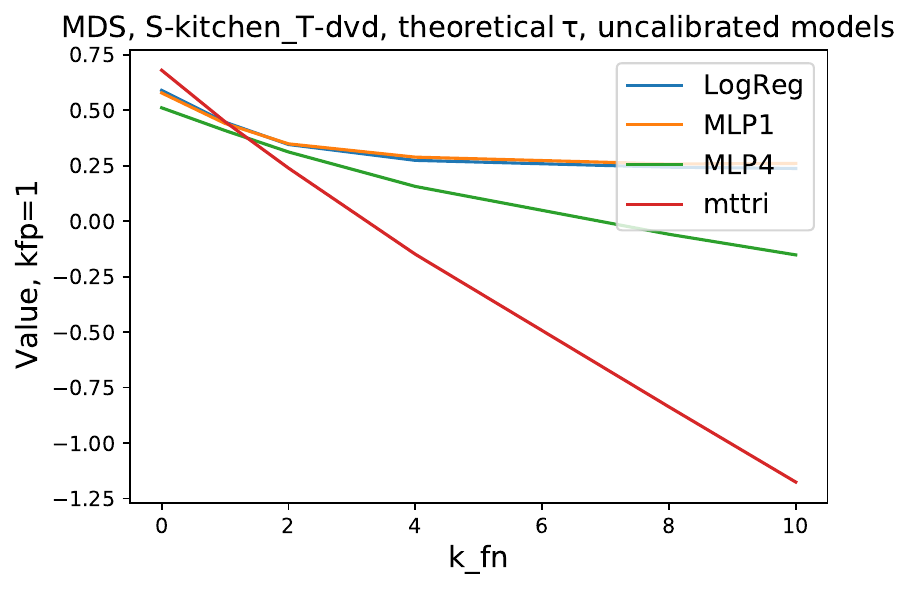} 
    \includegraphics[width=.245\linewidth]{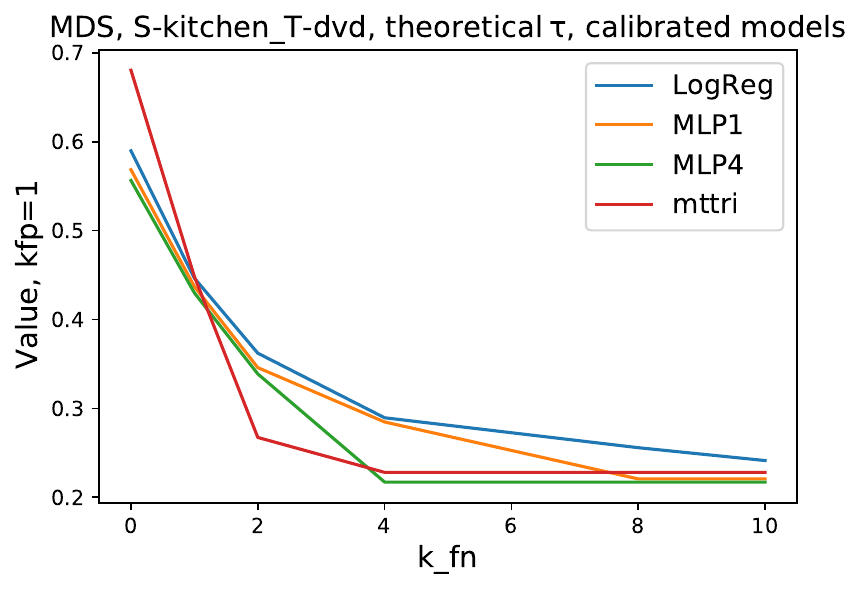}
    \includegraphics[width=.245\linewidth]{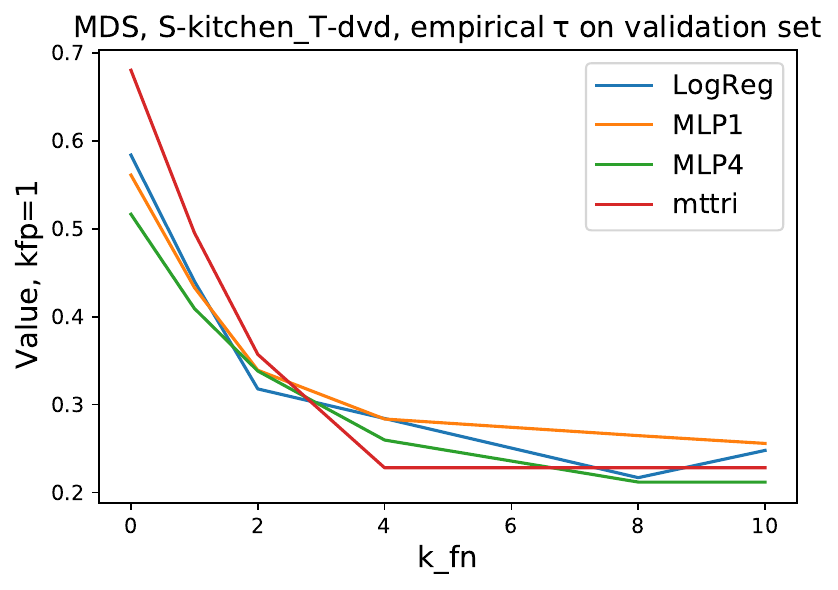}
    \includegraphics[width=.245\linewidth]{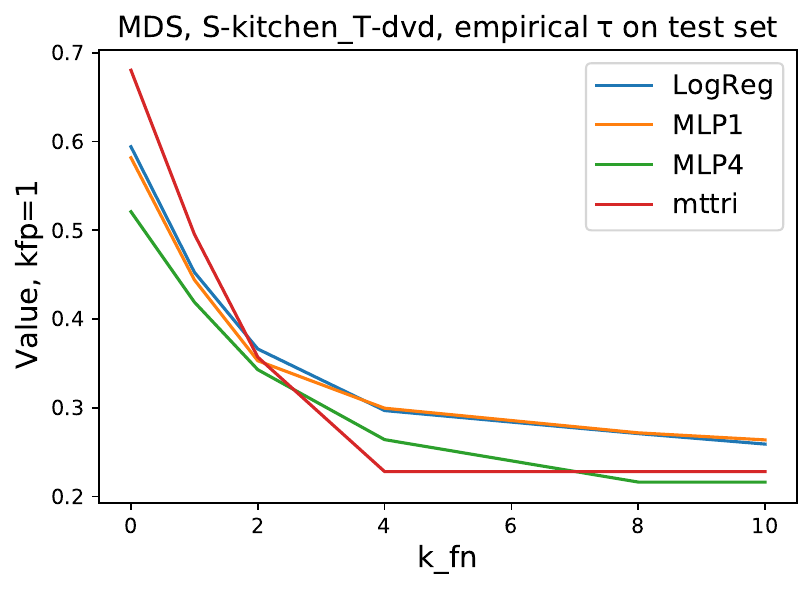}
    \includegraphics[width=.245\linewidth]{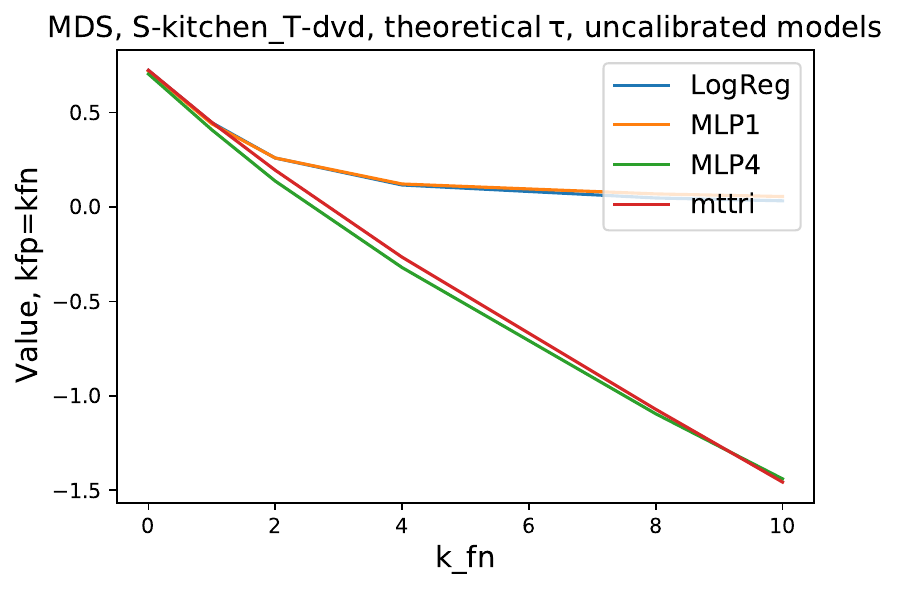} 
    \includegraphics[width=.245\linewidth]{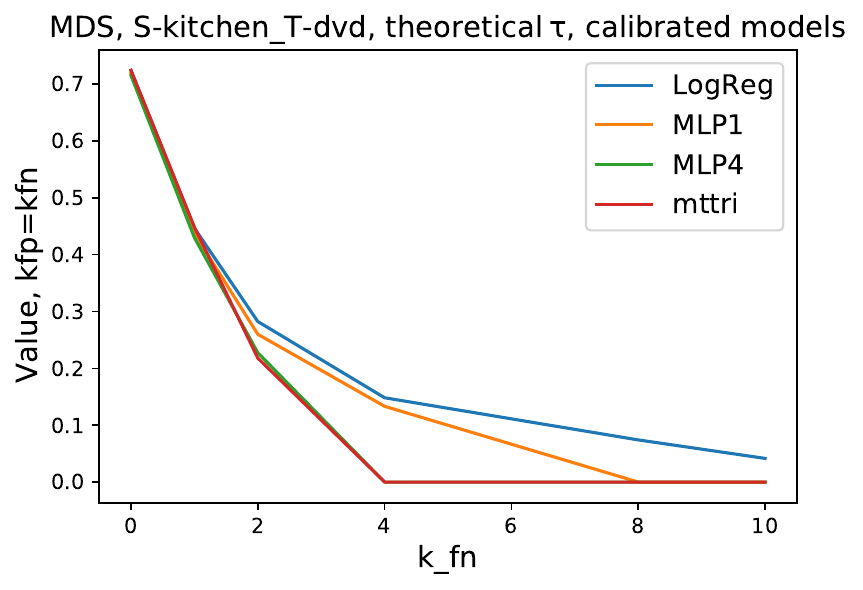}
    \includegraphics[width=.245\linewidth]{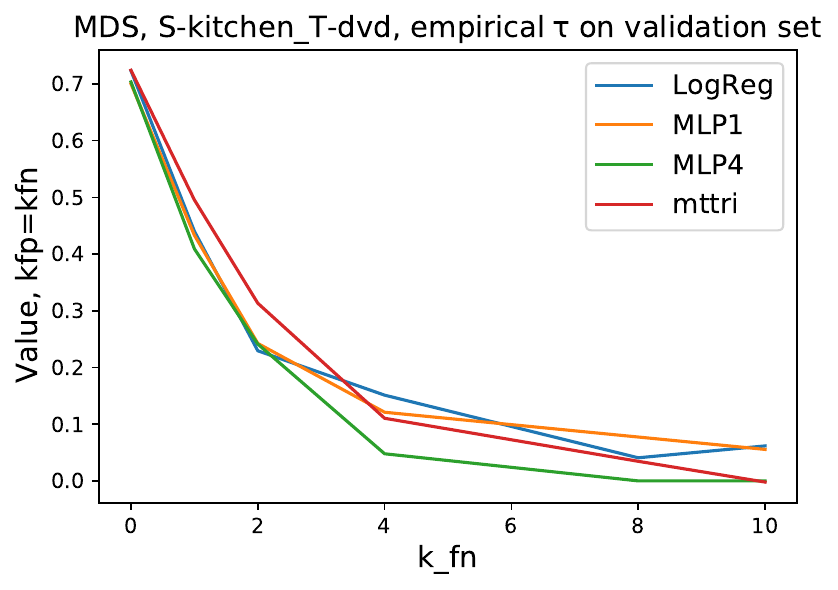}
    \includegraphics[width=.245\linewidth]{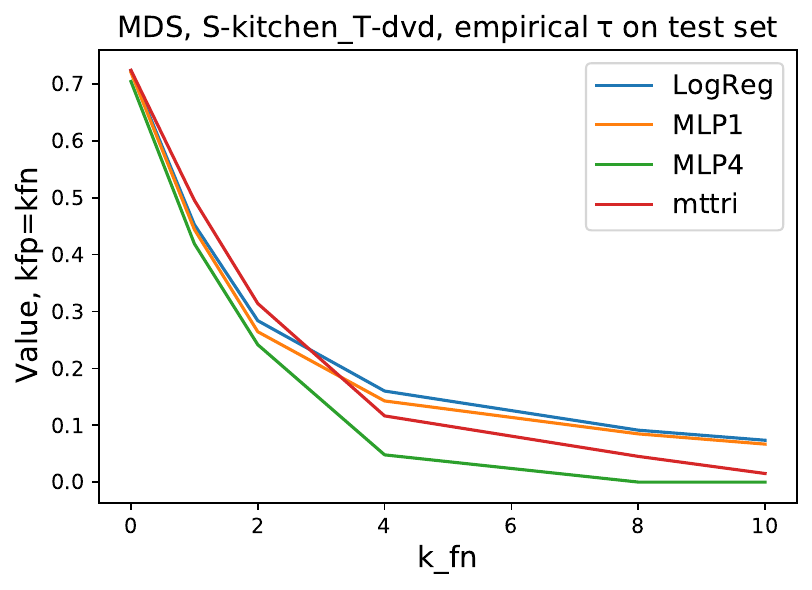}
    
    \caption{\label{fig:MDS_value_dvd}Value curves on Multi Domain Sentiment dataset for increasing $k_{fn}$, TARGET = 'DVD'. We use S-SOURCE\_T-TARGET format in the sub-figure titles, values show the performance of each model trained on a source domain and tested on a target domain.}
\end{figure*}%%

\begin{figure*}[!htbp]
 \centering
    \includegraphics[width=.245\linewidth]{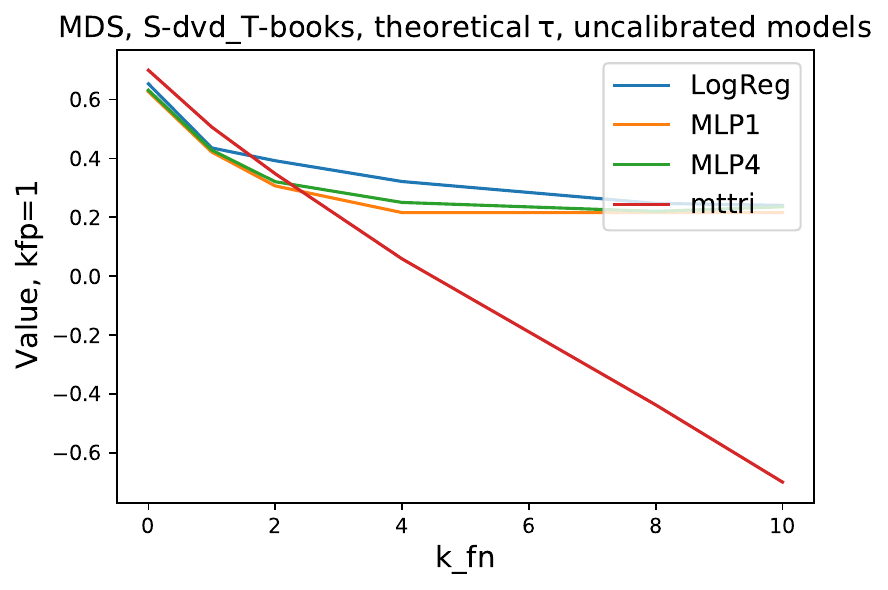} 
    \includegraphics[width=.245\linewidth]{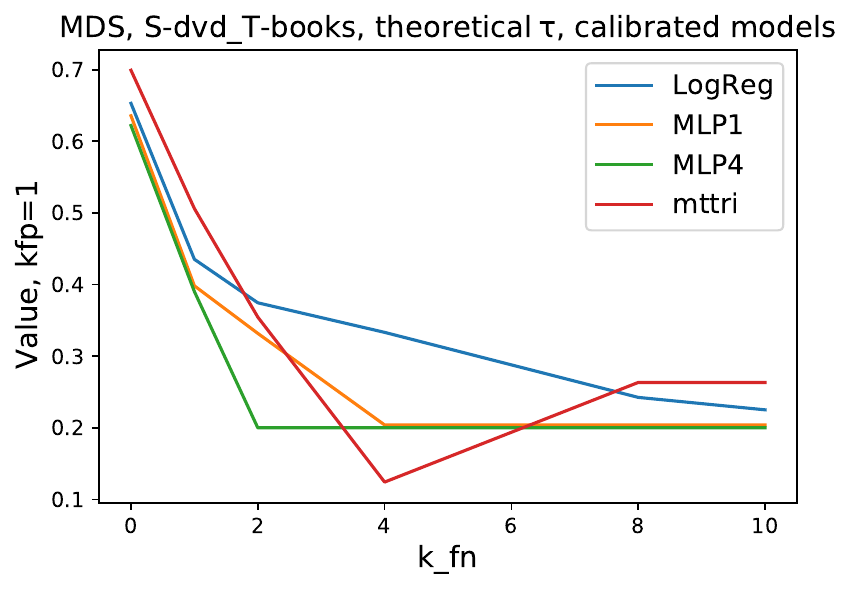}
    \includegraphics[width=.245\linewidth]{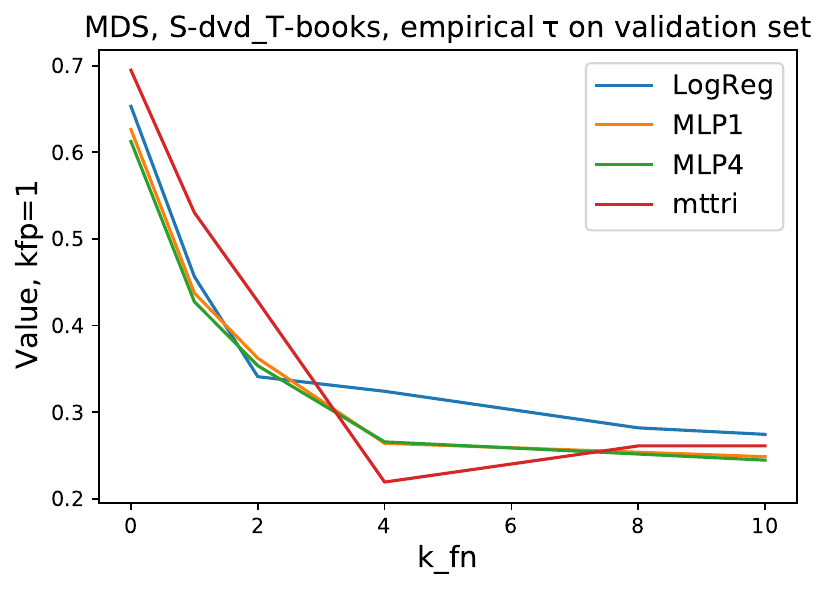}
    \includegraphics[width=.245\linewidth]{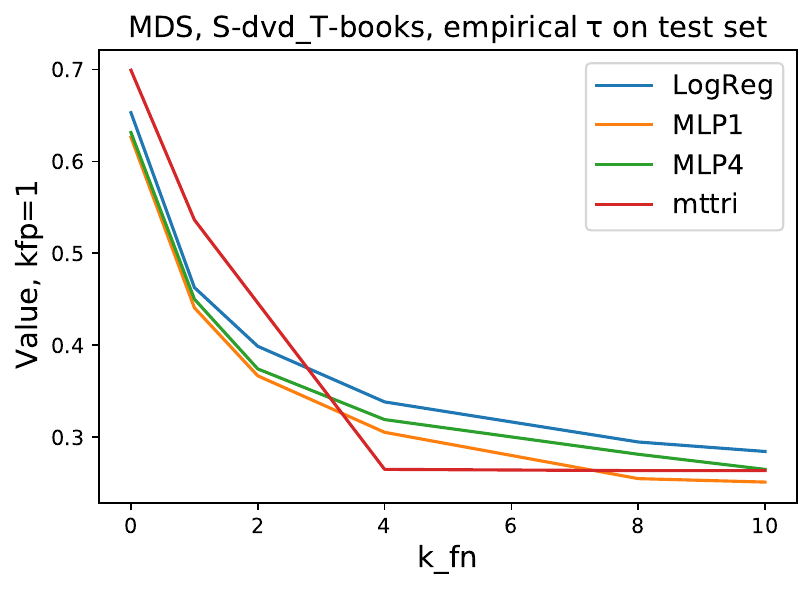}
    \includegraphics[width=.245\linewidth]{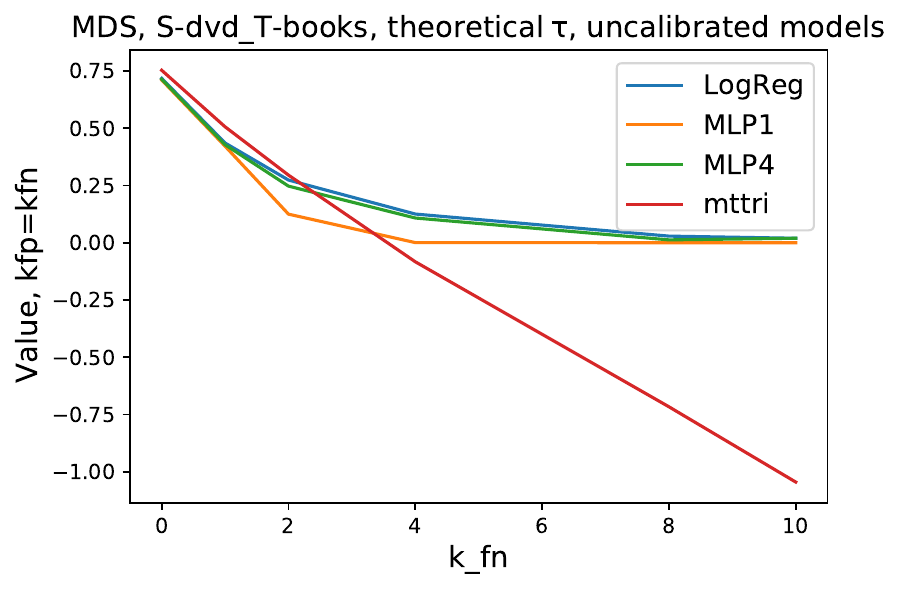} 
    \includegraphics[width=.245\linewidth]{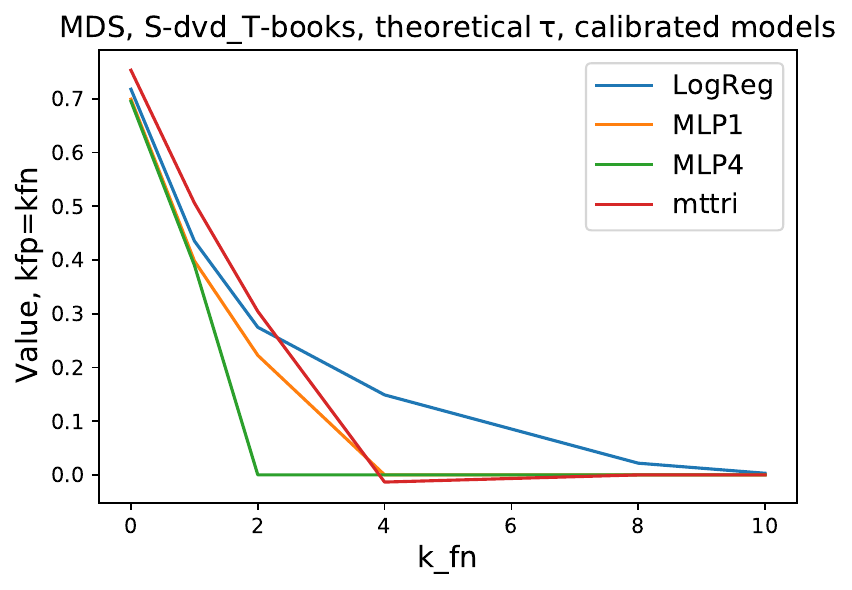}
    \includegraphics[width=.245\linewidth]{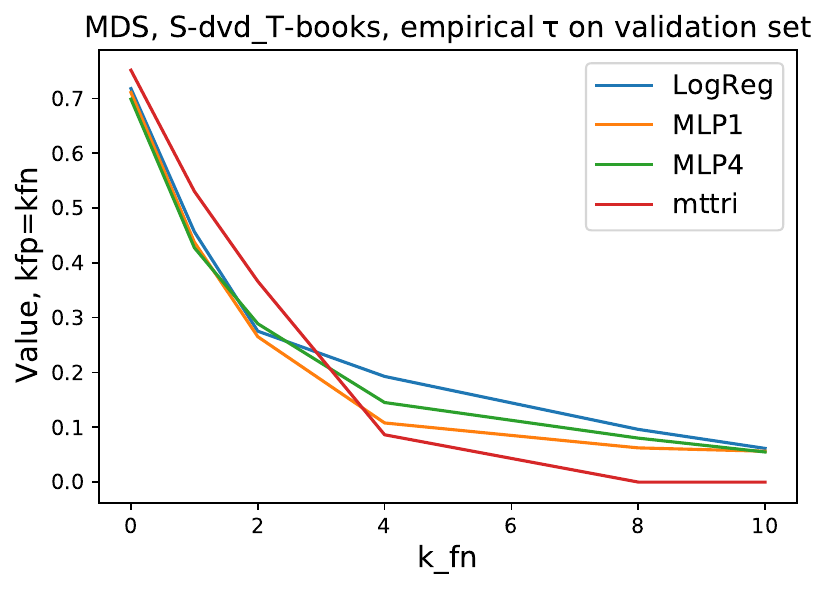}
    \includegraphics[width=.245\linewidth]{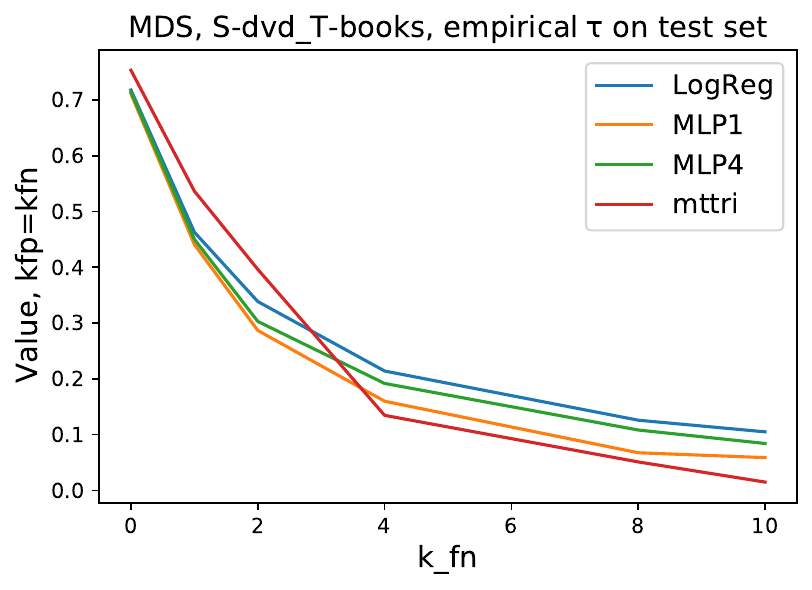}
    
    \includegraphics[width=.245\linewidth]{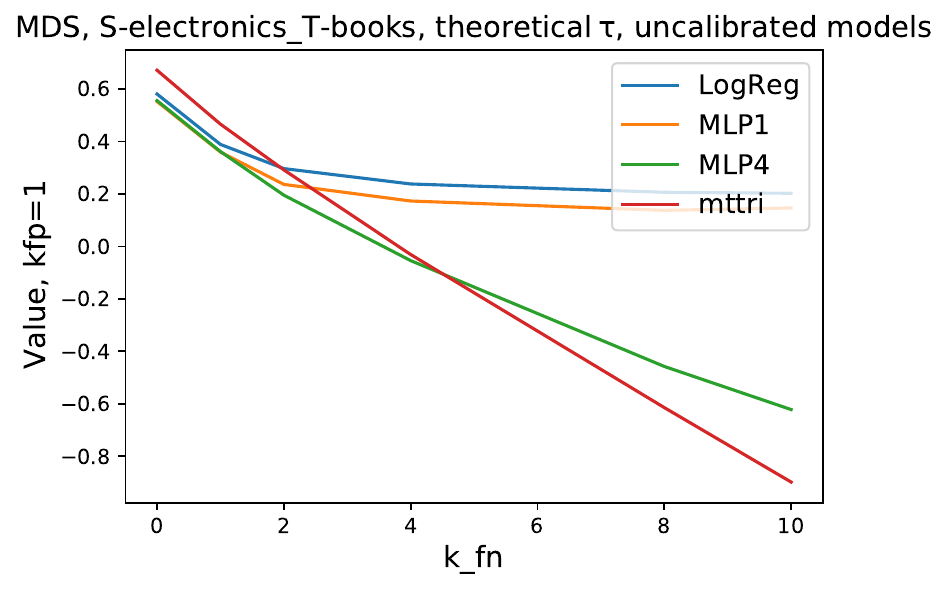} 
    \includegraphics[width=.245\linewidth]{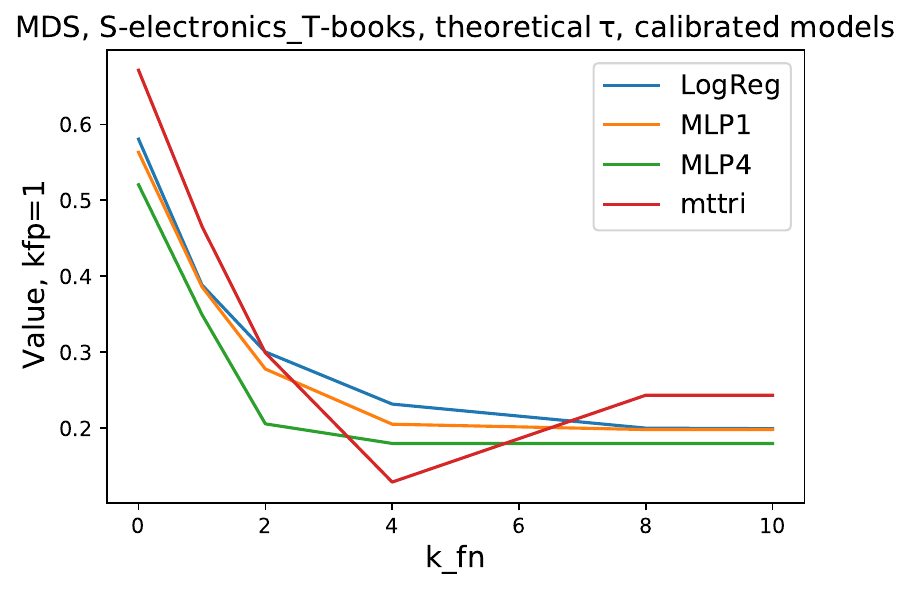}
    \includegraphics[width=.245\linewidth]{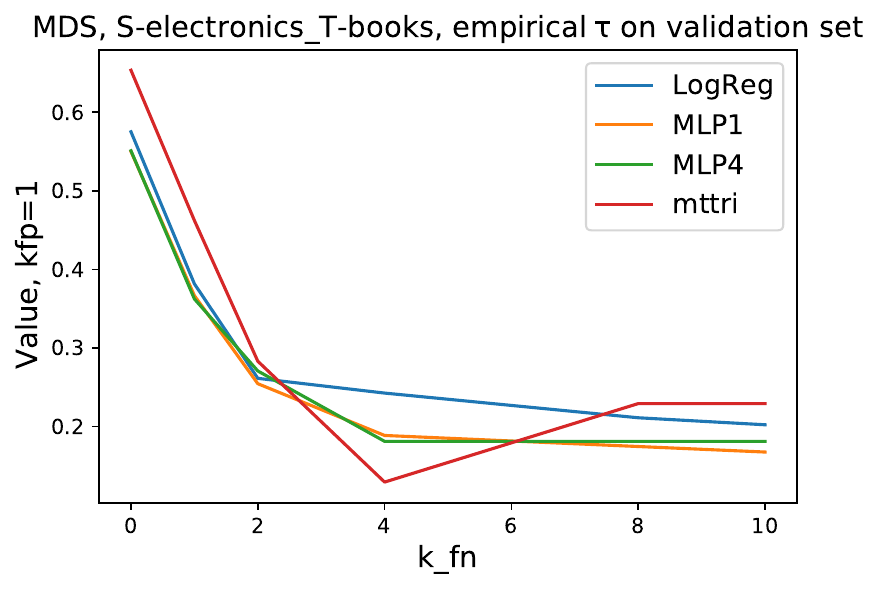}
    \includegraphics[width=.245\linewidth]{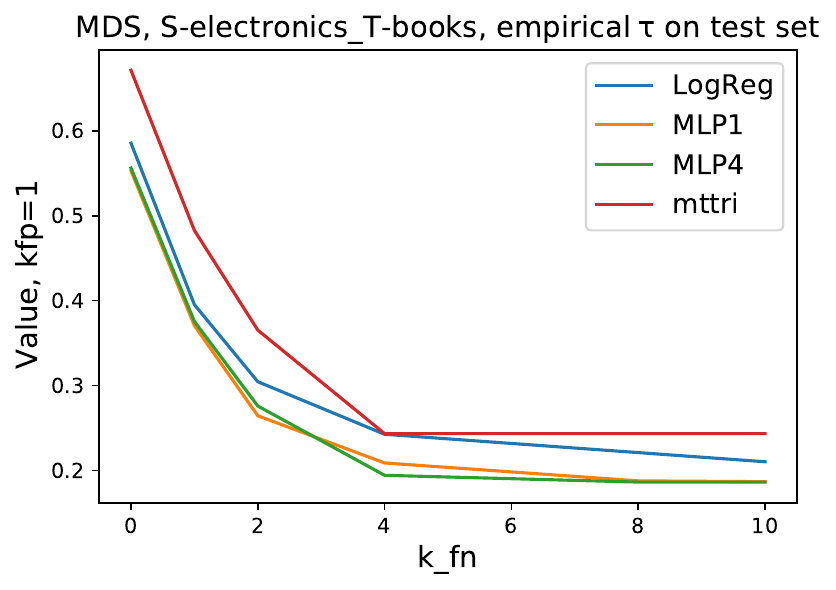}
    \includegraphics[width=.245\linewidth]{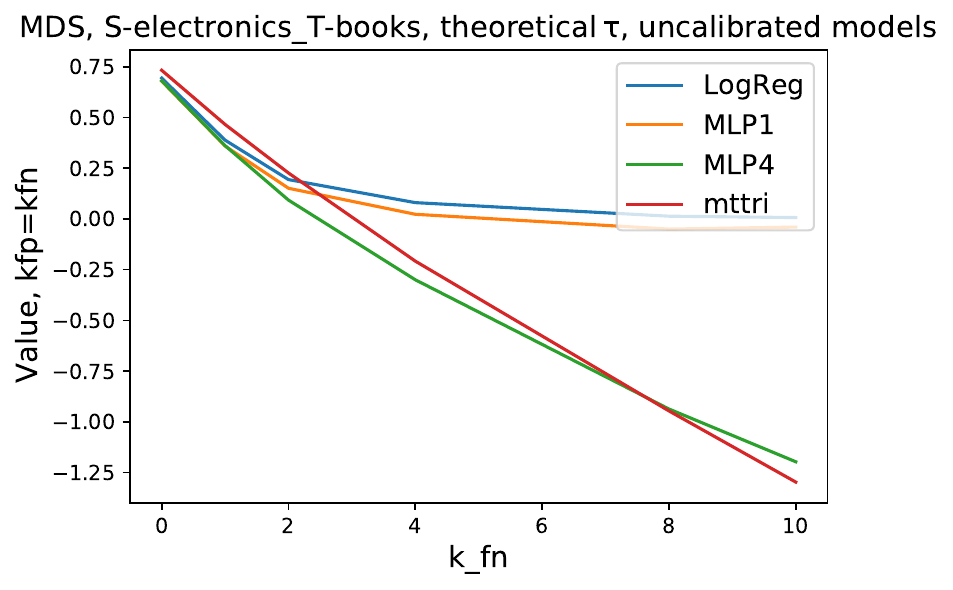} 
    \includegraphics[width=.245\linewidth]{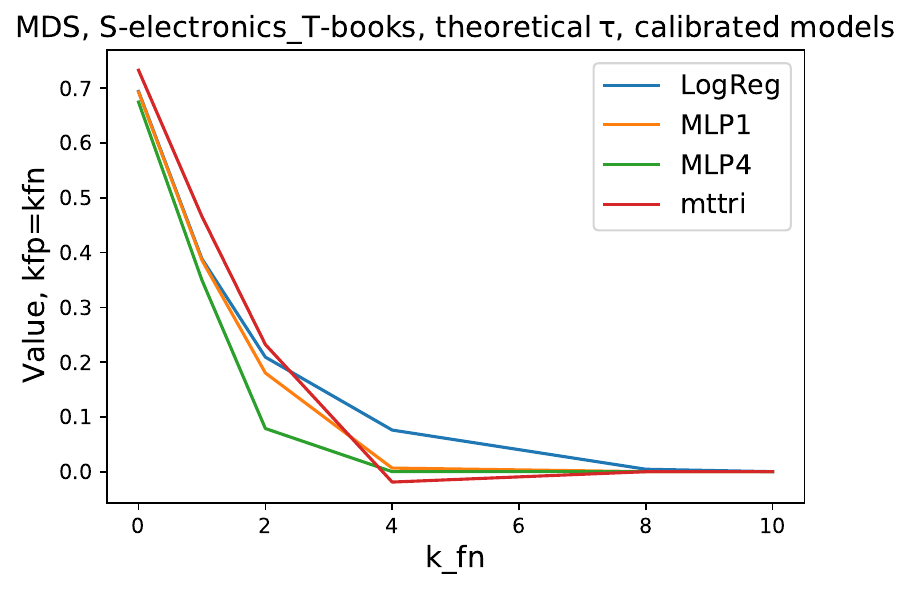}
    \includegraphics[width=.245\linewidth]{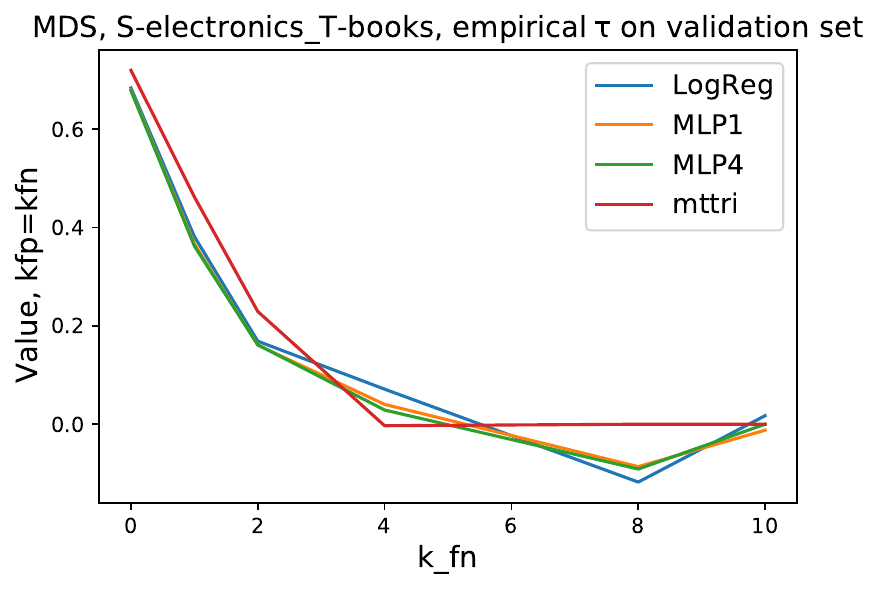}
    \includegraphics[width=.245\linewidth]{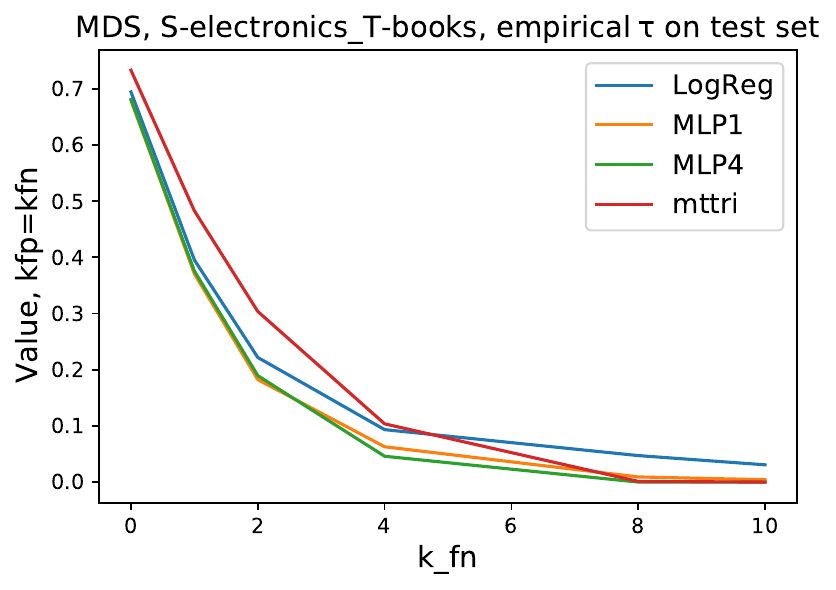}
    
    \includegraphics[width=.245\linewidth]{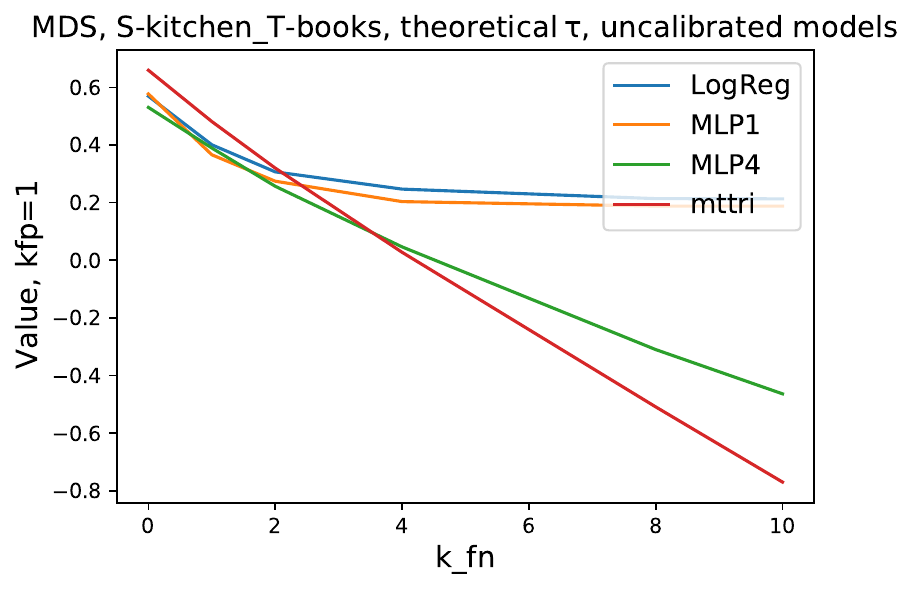} 
    \includegraphics[width=.245\linewidth]{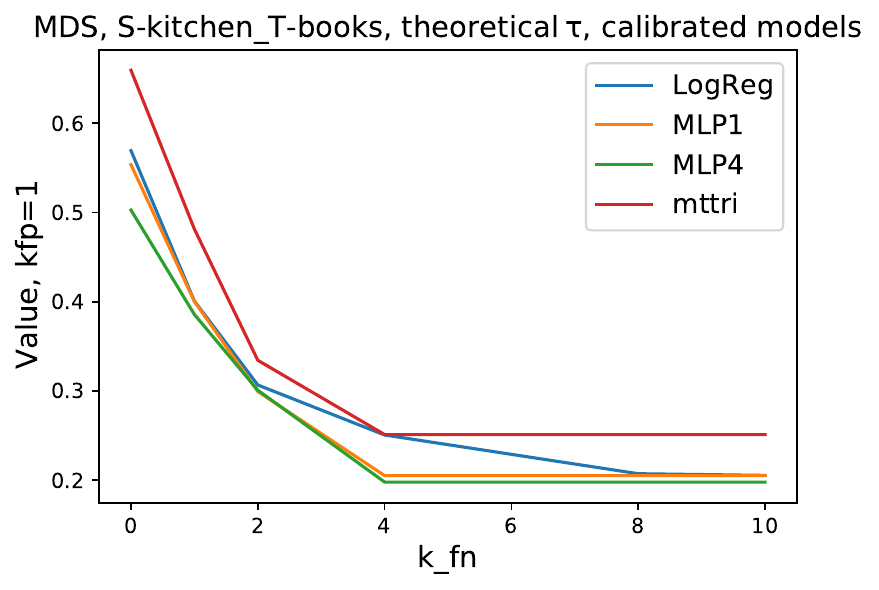}
    \includegraphics[width=.245\linewidth]{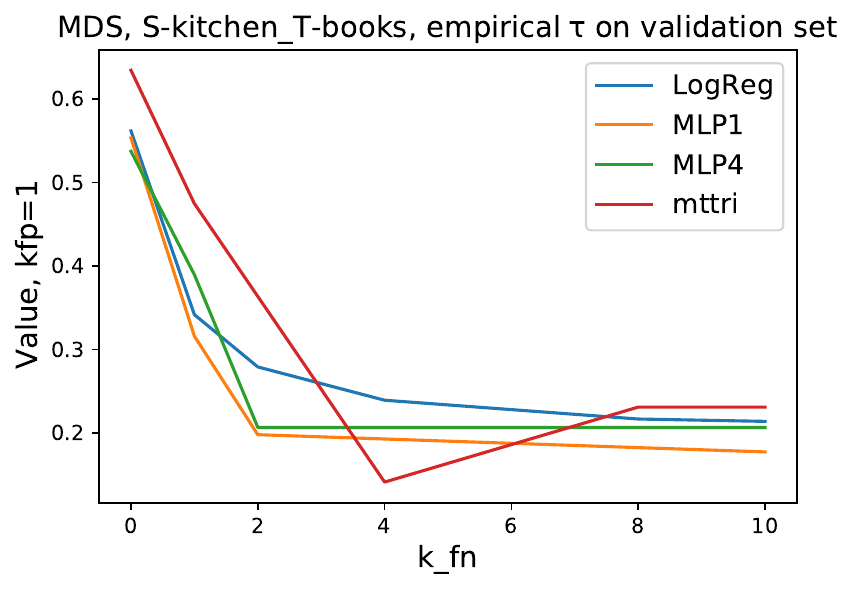}
    \includegraphics[width=.245\linewidth]{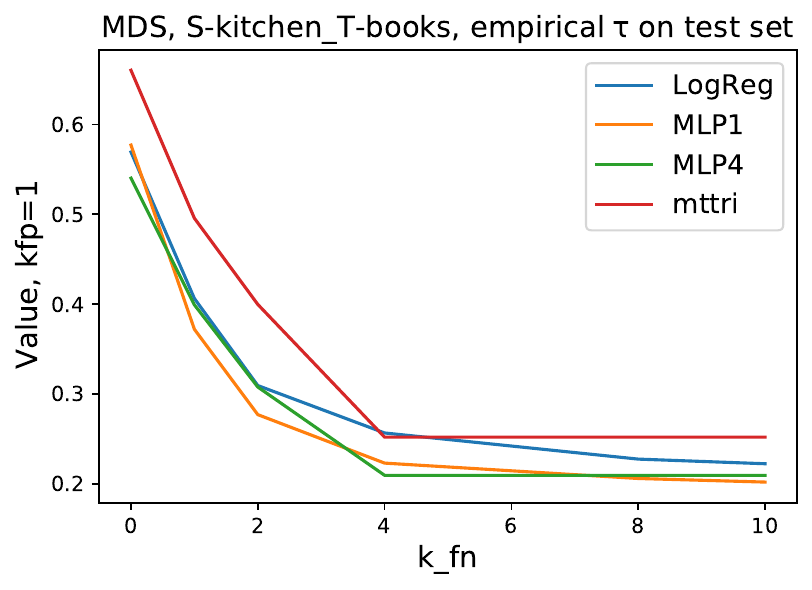}
    \includegraphics[width=.245\linewidth]{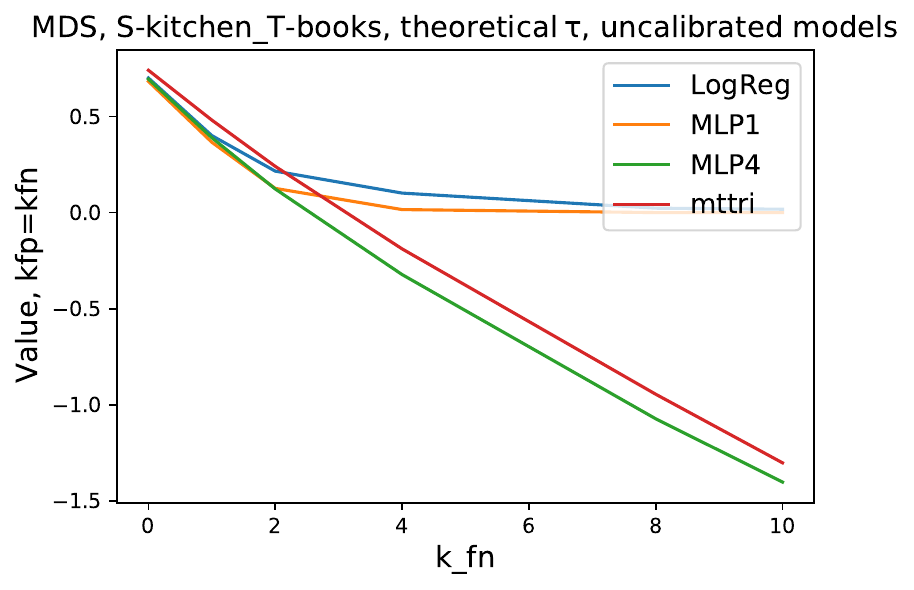} 
    \includegraphics[width=.245\linewidth]{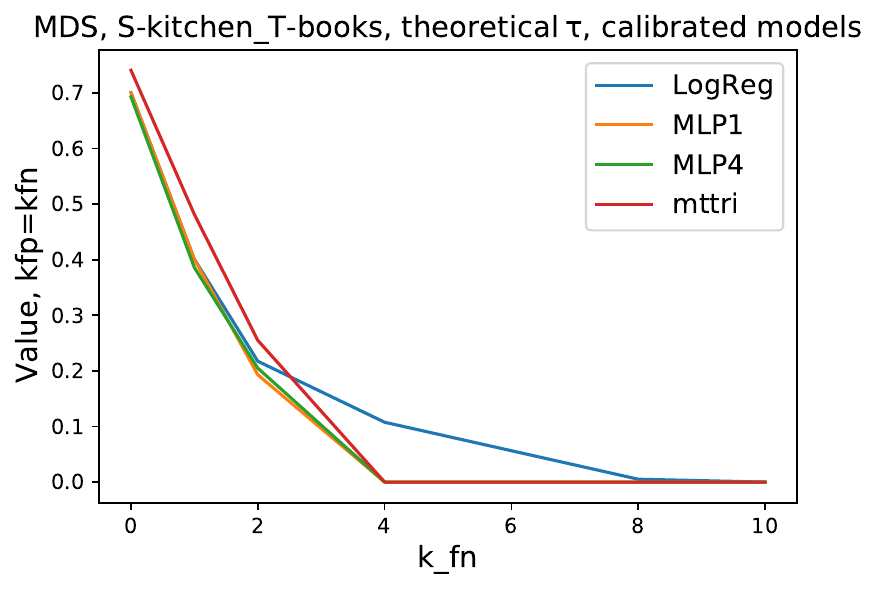}
    \includegraphics[width=.245\linewidth]{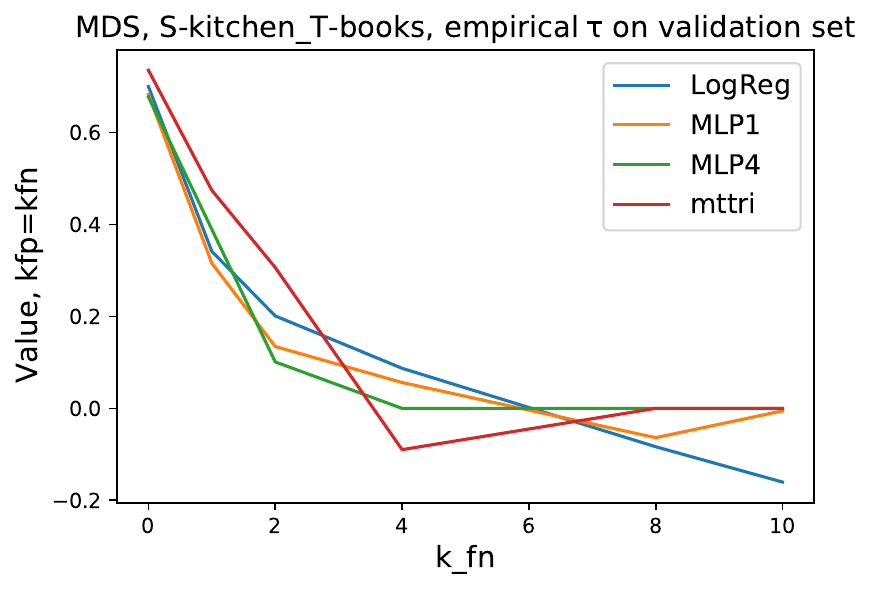}
    \includegraphics[width=.245\linewidth]{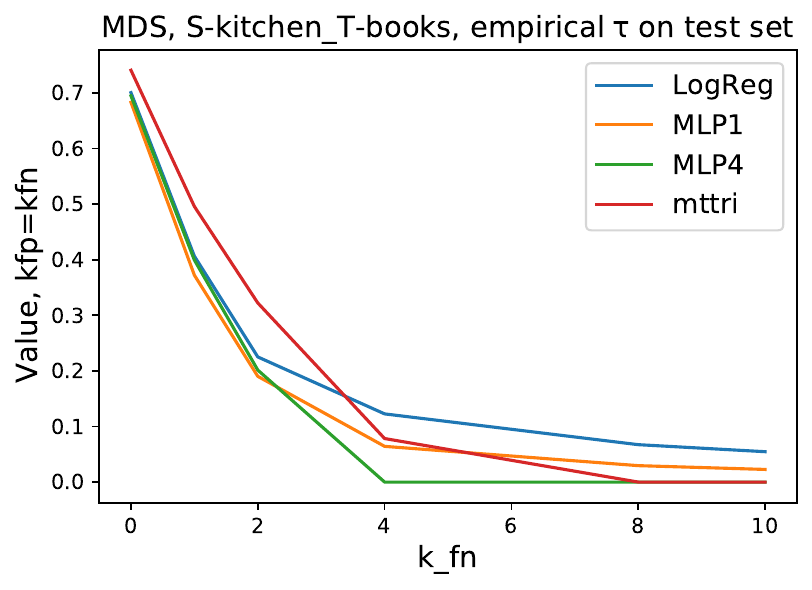}
    
    \caption{\label{fig:MDS_value_books}Value curves on Multi Domain Sentiment dataset for increasing $k_{fn}$, TARGET = 'Books'. We use S-SOURCE\_T-TARGET format in the sub-figure titles, values show the performance of each model trained on a source domain and tested on a target domain.}
\end{figure*}%%

\begin{figure*}[!htbp]
 \centering
    \includegraphics[width=.245\linewidth]{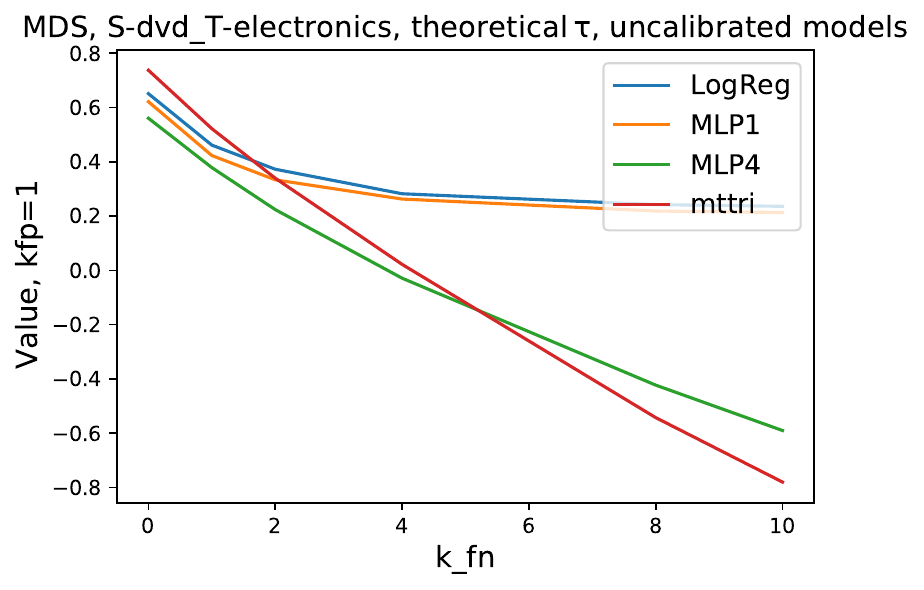} 
    \includegraphics[width=.245\linewidth]{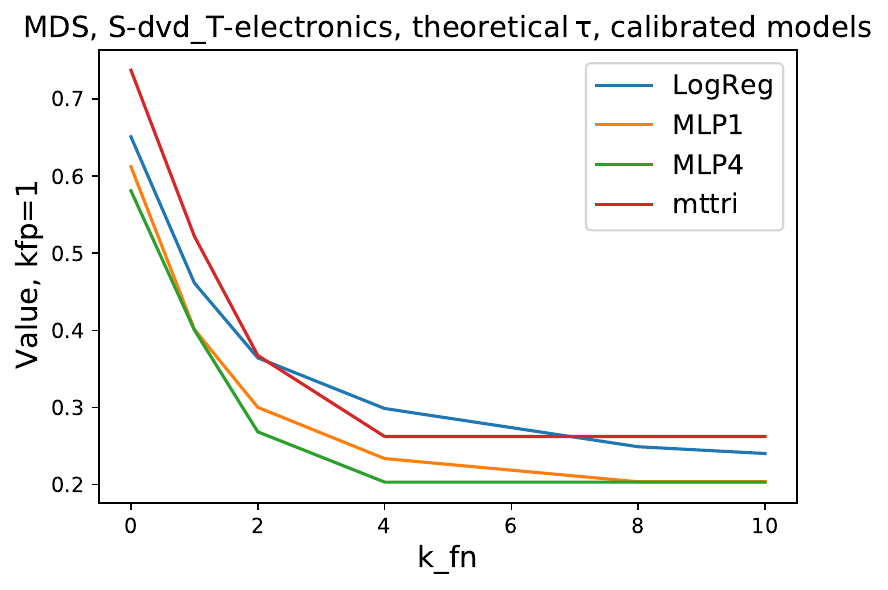}
    \includegraphics[width=.245\linewidth]{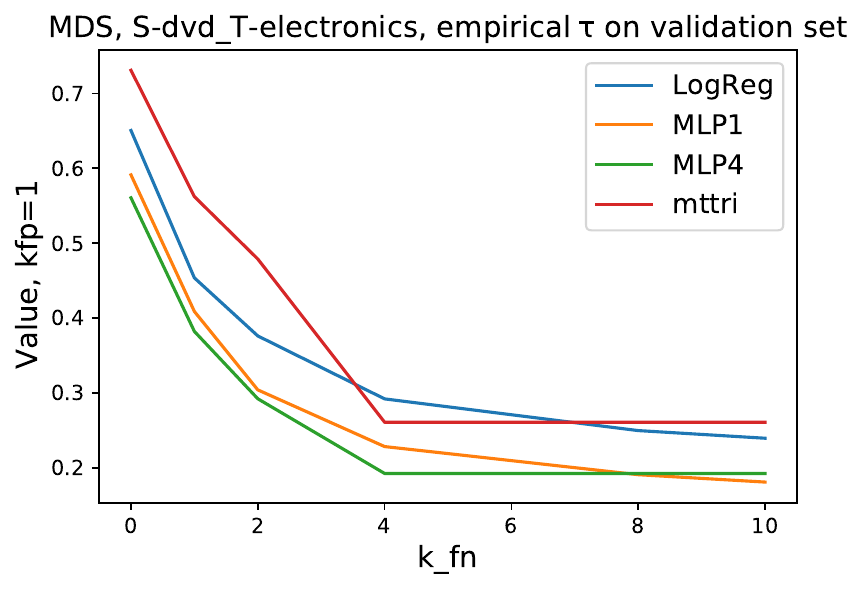}
    \includegraphics[width=.245\linewidth]{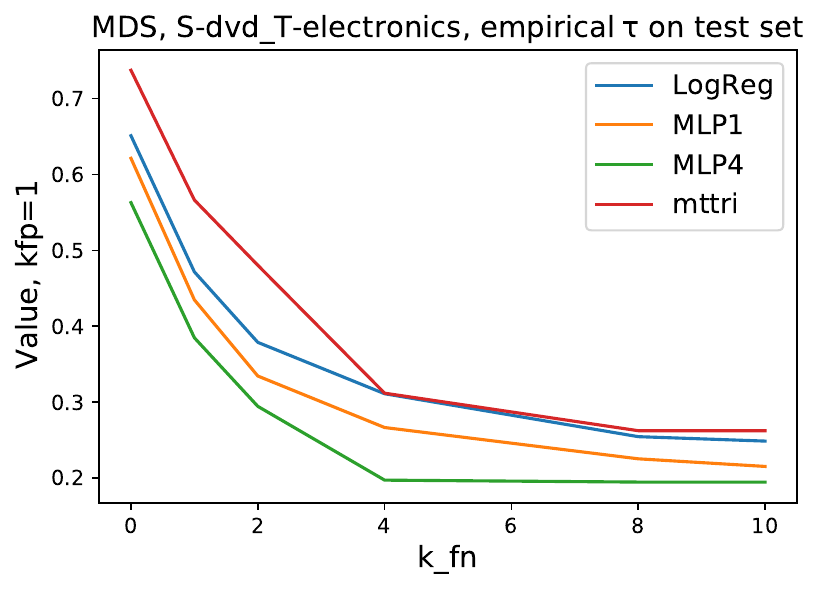}
    \includegraphics[width=.245\linewidth]{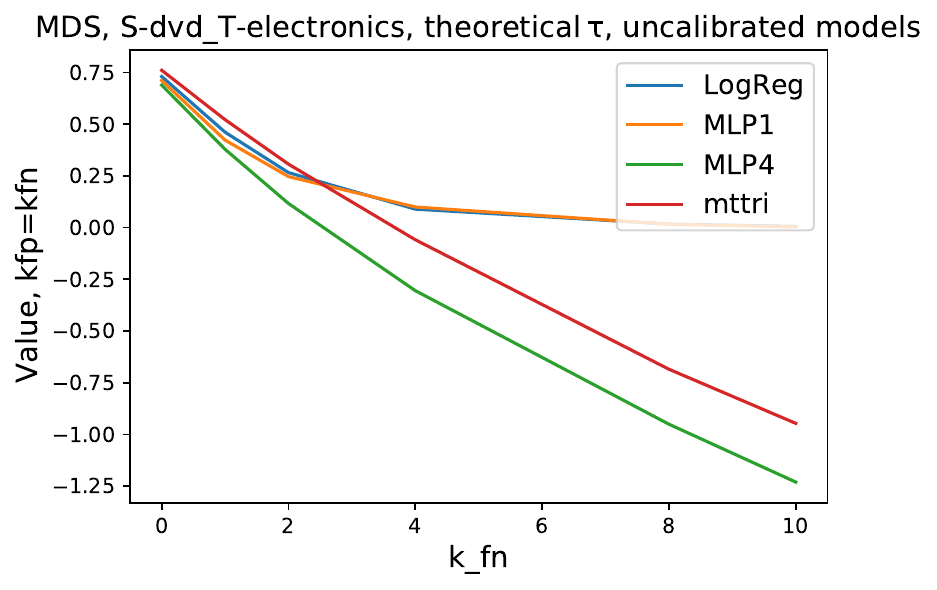} 
    \includegraphics[width=.245\linewidth]{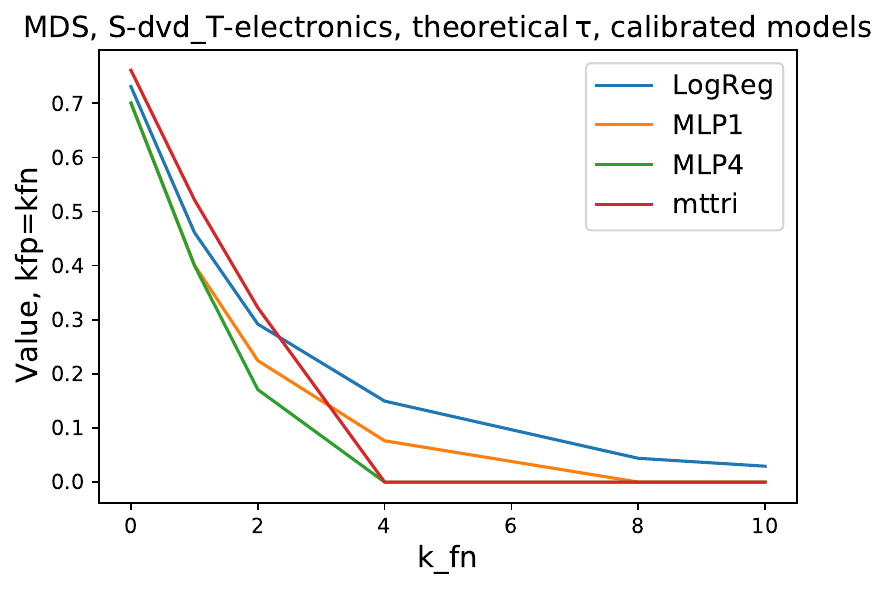}
    \includegraphics[width=.245\linewidth]{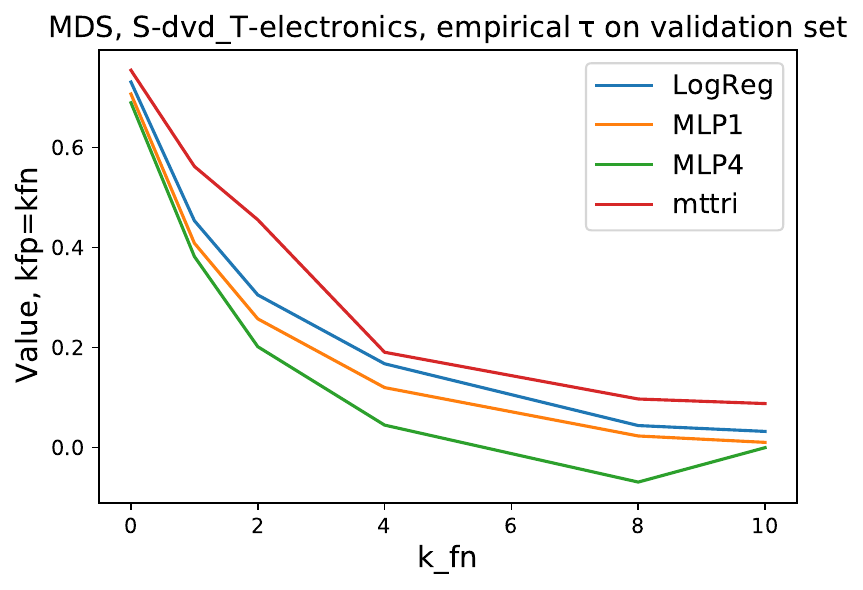}
    \includegraphics[width=.245\linewidth]{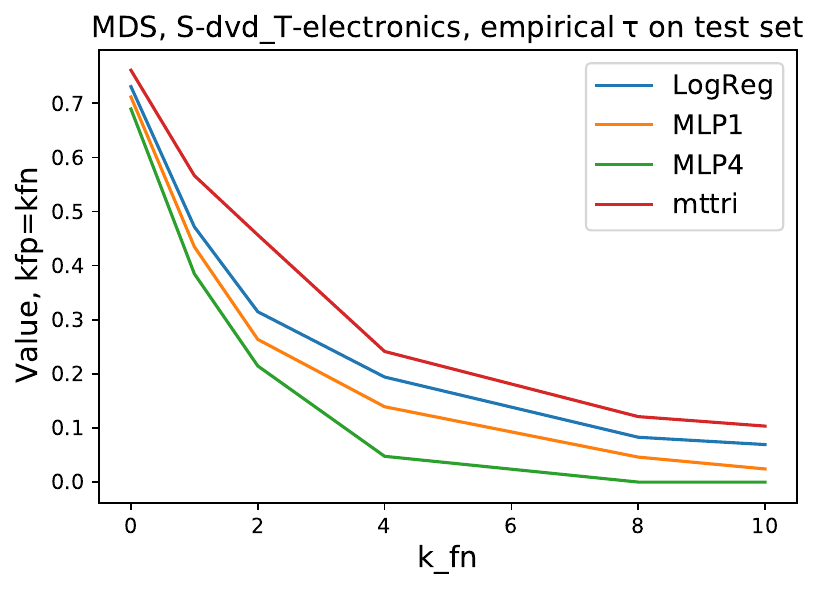}
    
    \includegraphics[width=.245\linewidth]{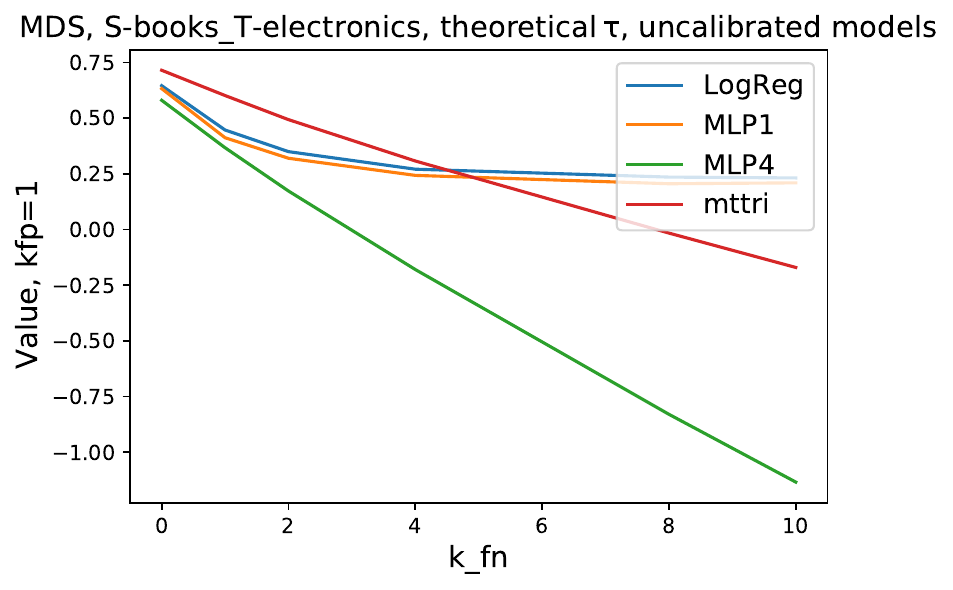} 
    \includegraphics[width=.245\linewidth]{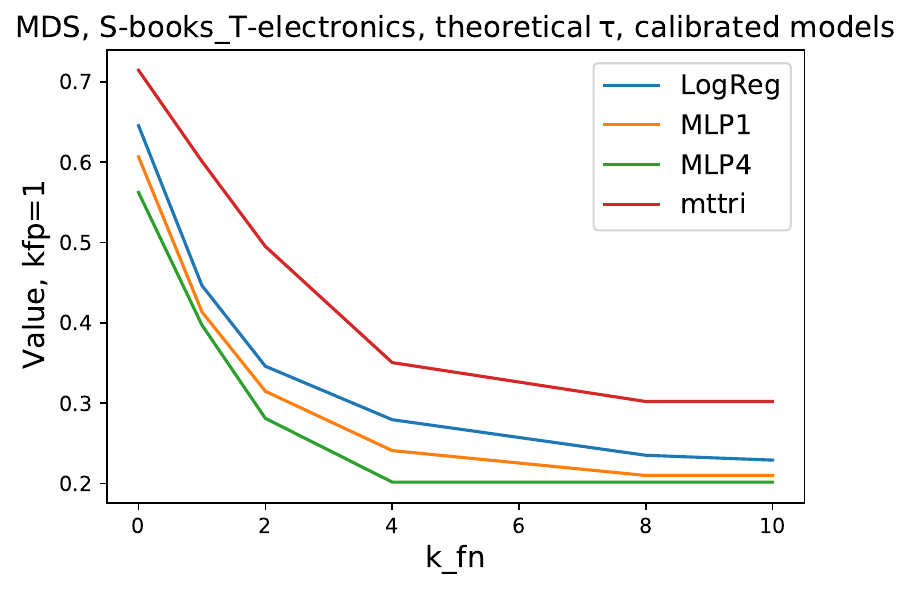}
    \includegraphics[width=.245\linewidth]{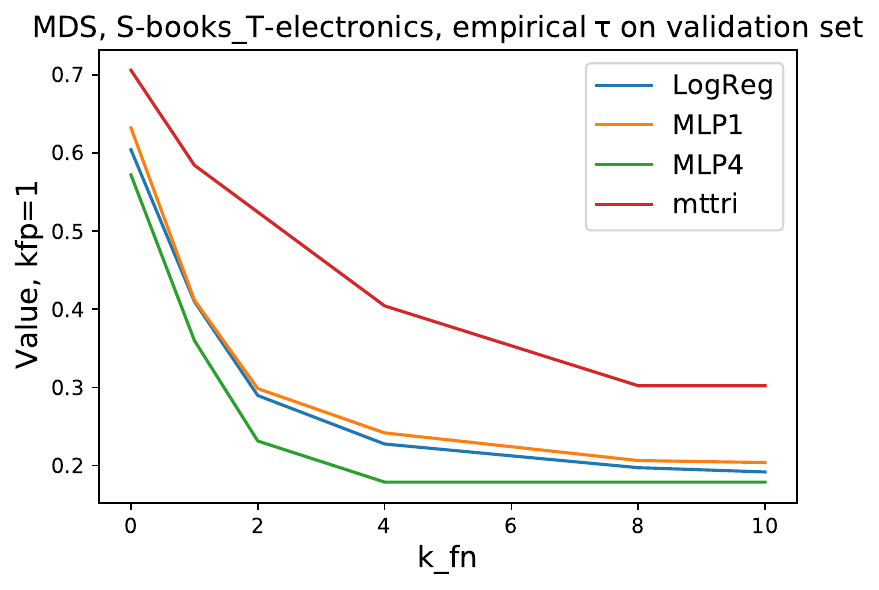}
    \includegraphics[width=.245\linewidth]{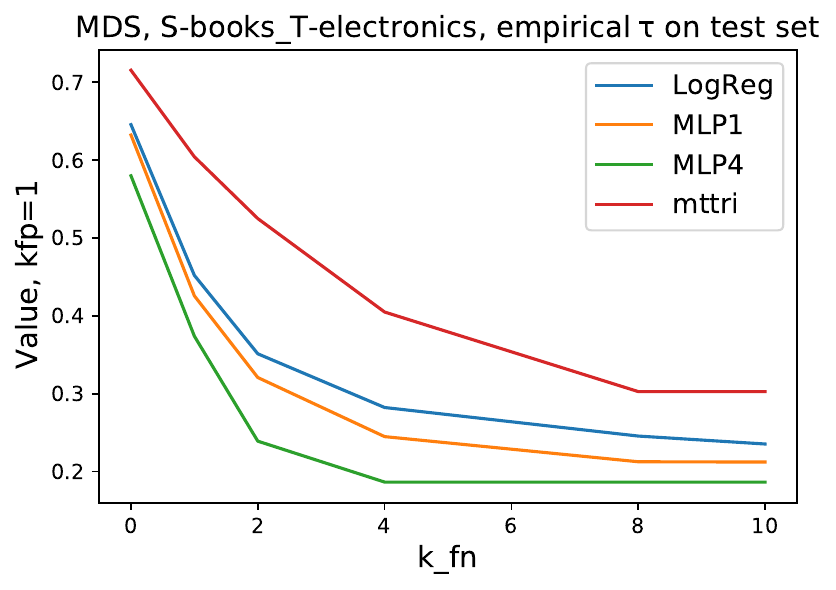}
    \includegraphics[width=.245\linewidth]{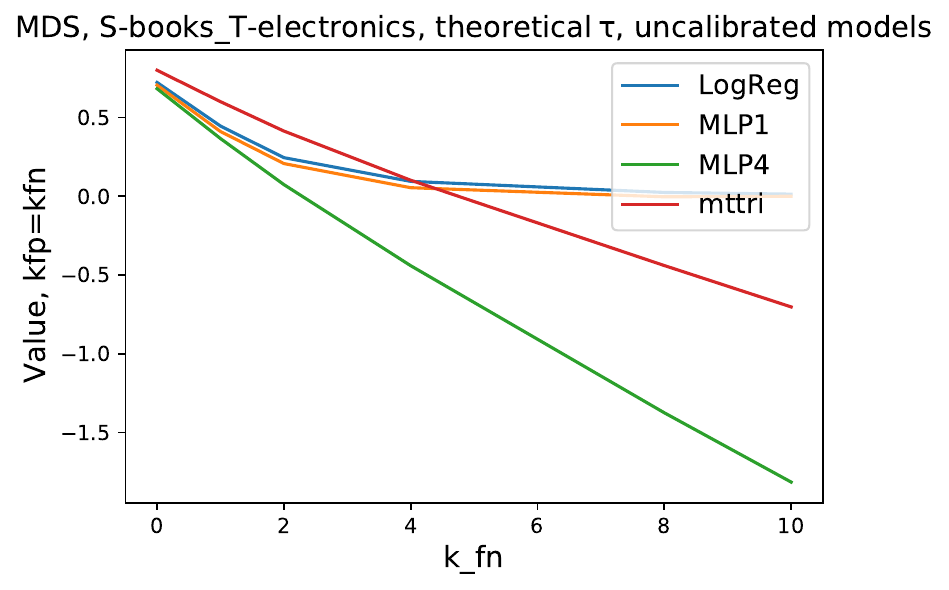} 
    \includegraphics[width=.245\linewidth]{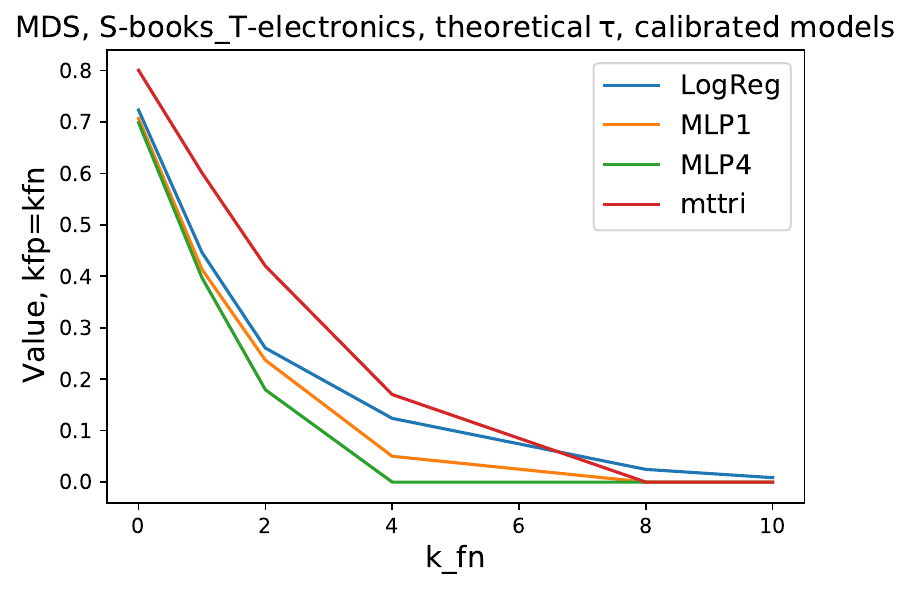}
    \includegraphics[width=.245\linewidth]{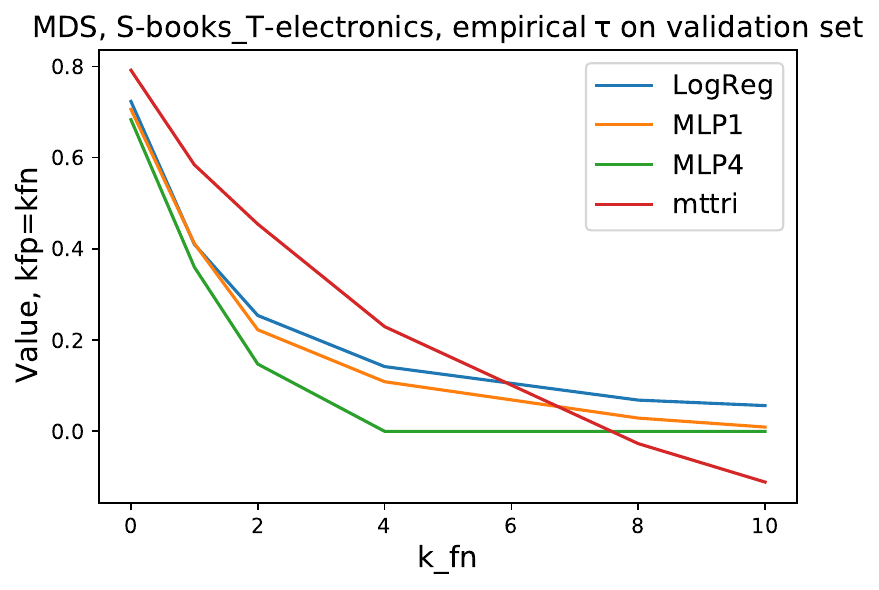}
    \includegraphics[width=.245\linewidth]{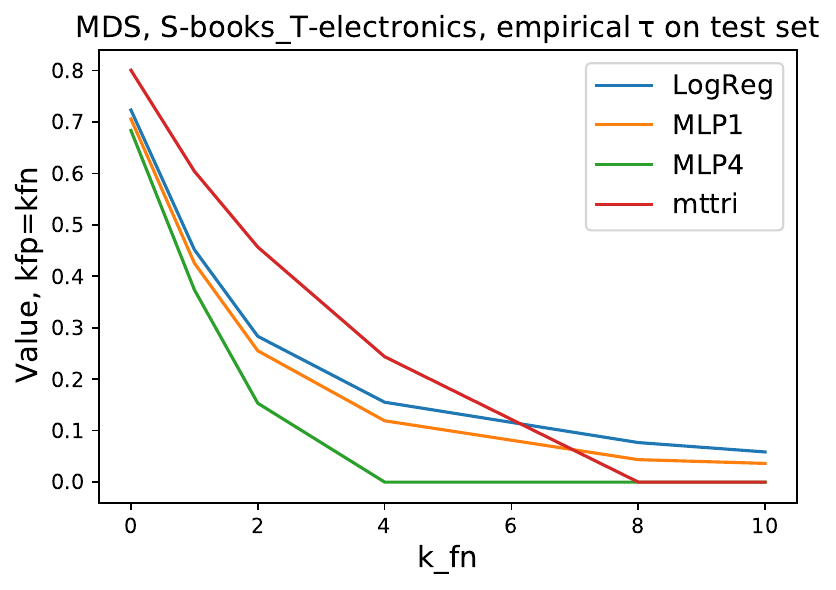}
    
    \includegraphics[width=.245\linewidth]{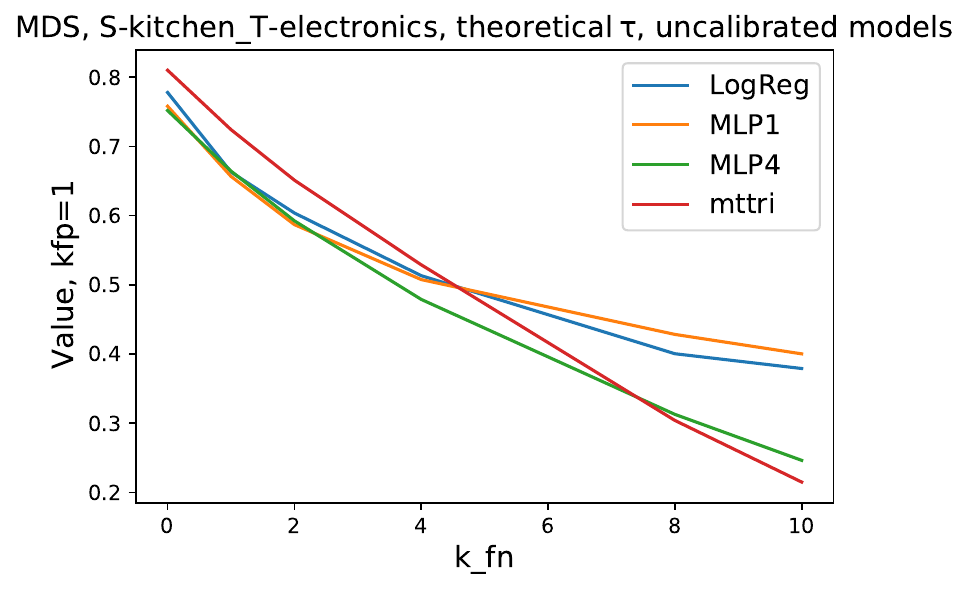} 
    \includegraphics[width=.245\linewidth]{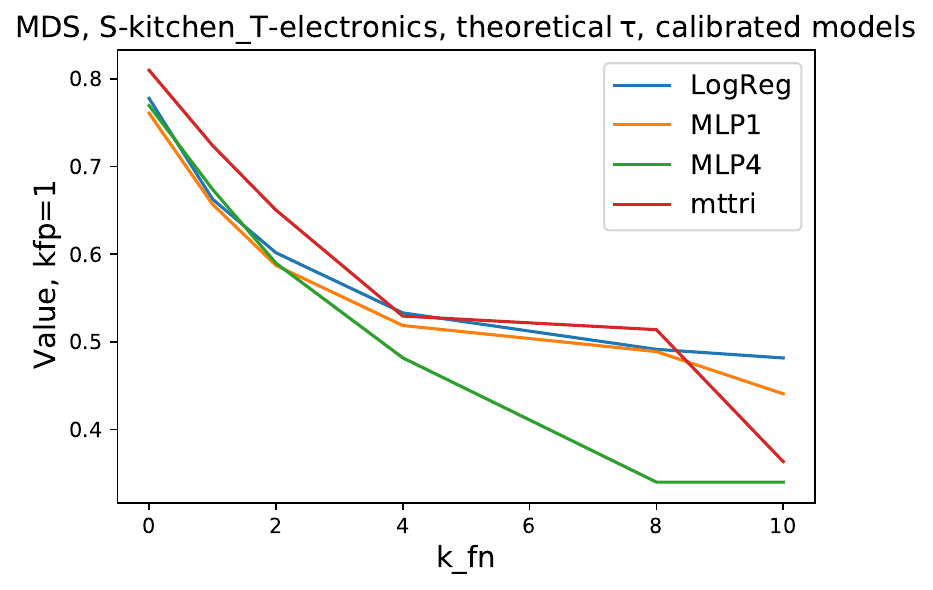}
    \includegraphics[width=.245\linewidth]{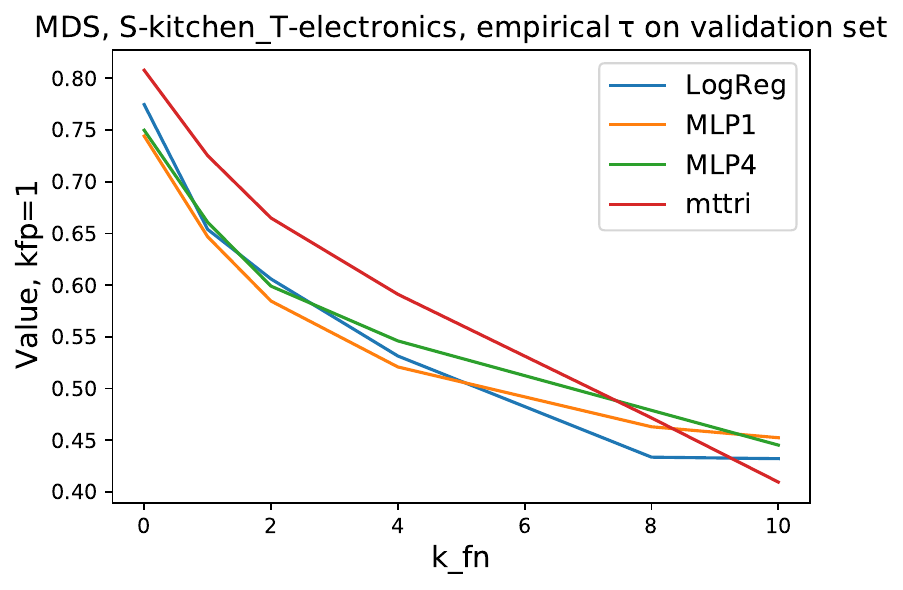}
    \includegraphics[width=.245\linewidth]{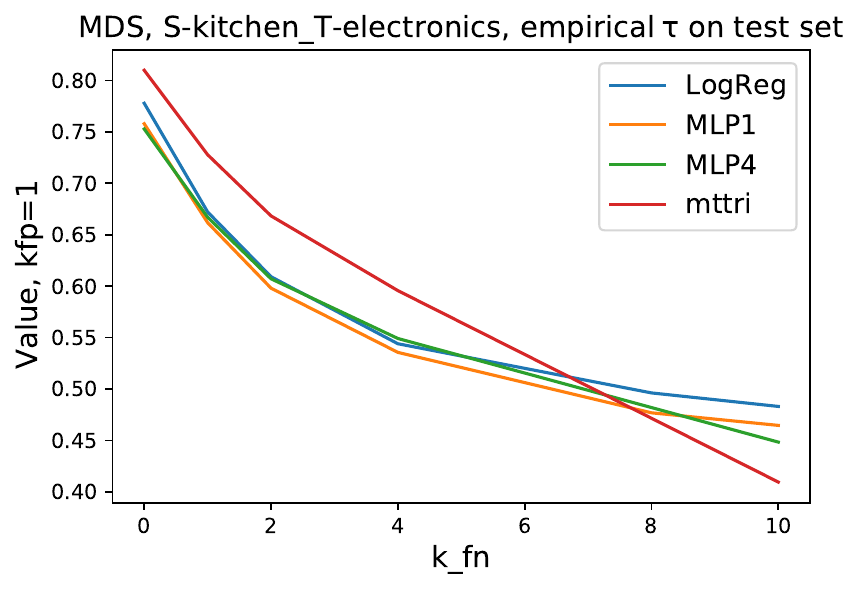}
    \includegraphics[width=.245\linewidth]{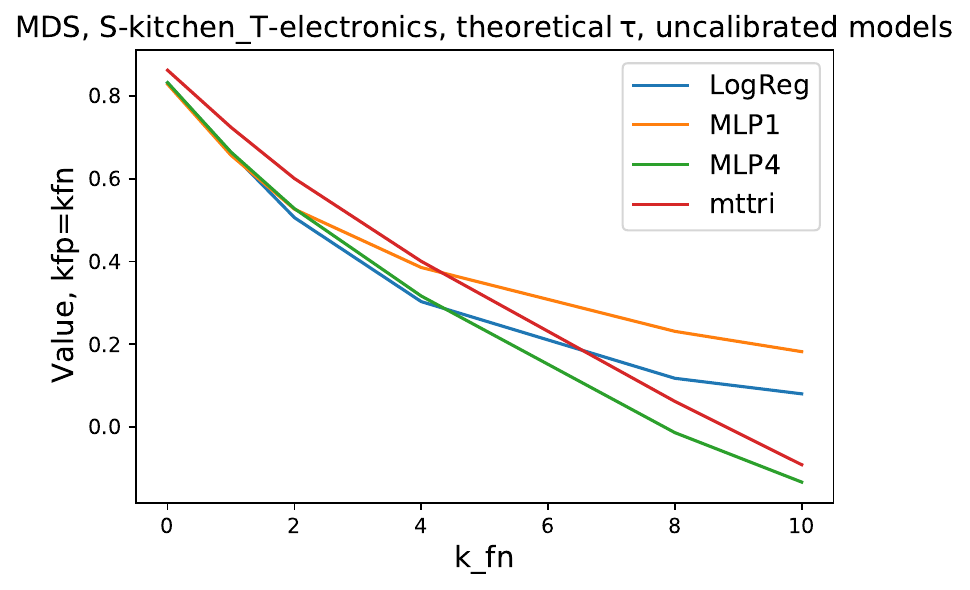} 
    \includegraphics[width=.245\linewidth]{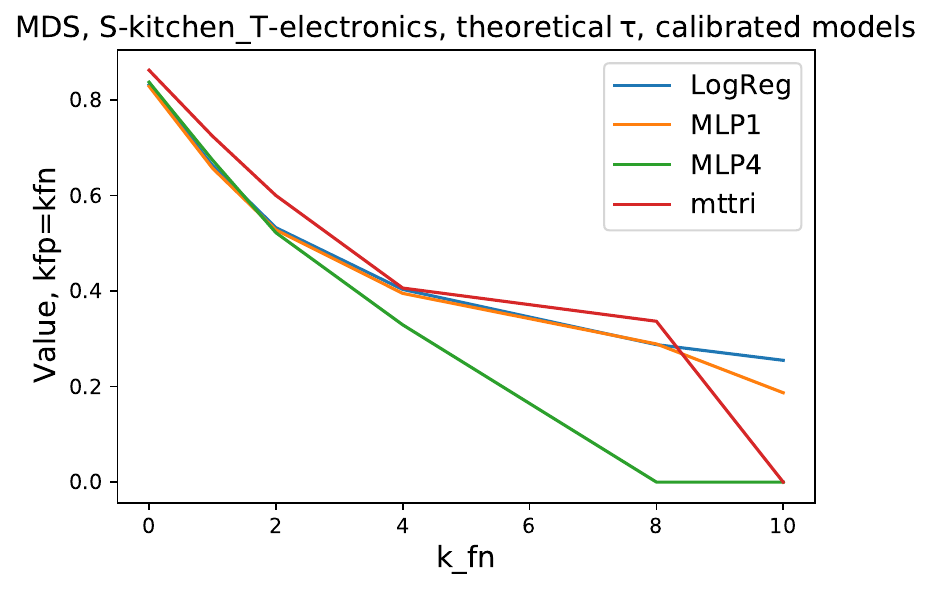}
    \includegraphics[width=.245\linewidth]{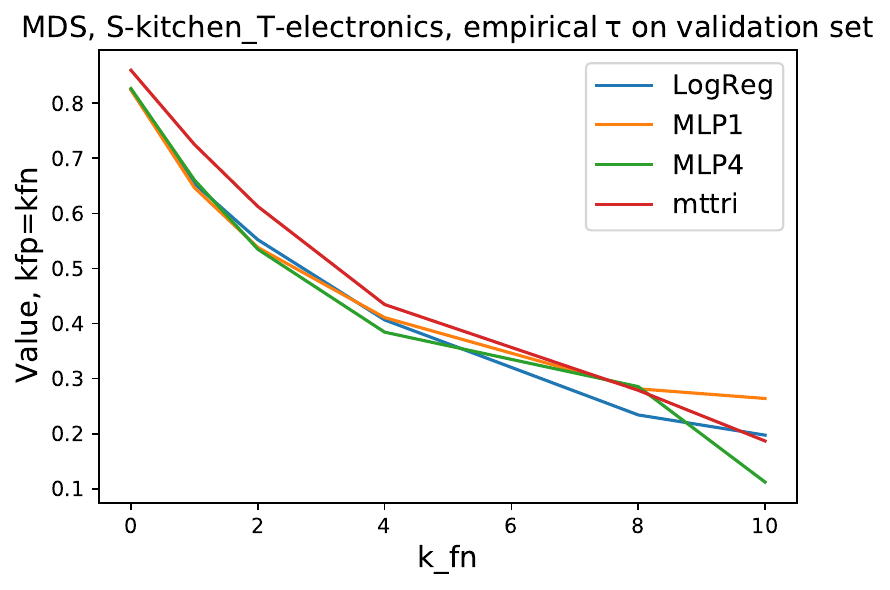}
    \includegraphics[width=.245\linewidth]{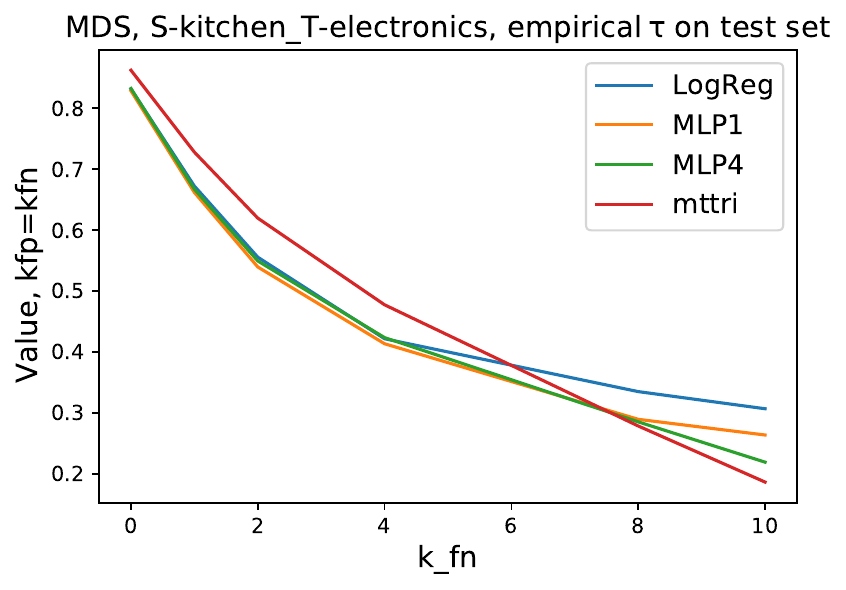}
    
    \caption{\label{fig:MDS_value_electronics}Value curves on Multi Domain Sentiment dataset for increasing $k_{fn}$, TARGET = 'Electronics'. We use S-SOURCE\_T-TARGET format in the sub-figure titles, values show the performance of each model trained on a source domain and tested on a target domain.}
\end{figure*}%%

\begin{figure*}[!htbp]
 \centering
    \includegraphics[width=.245\linewidth]{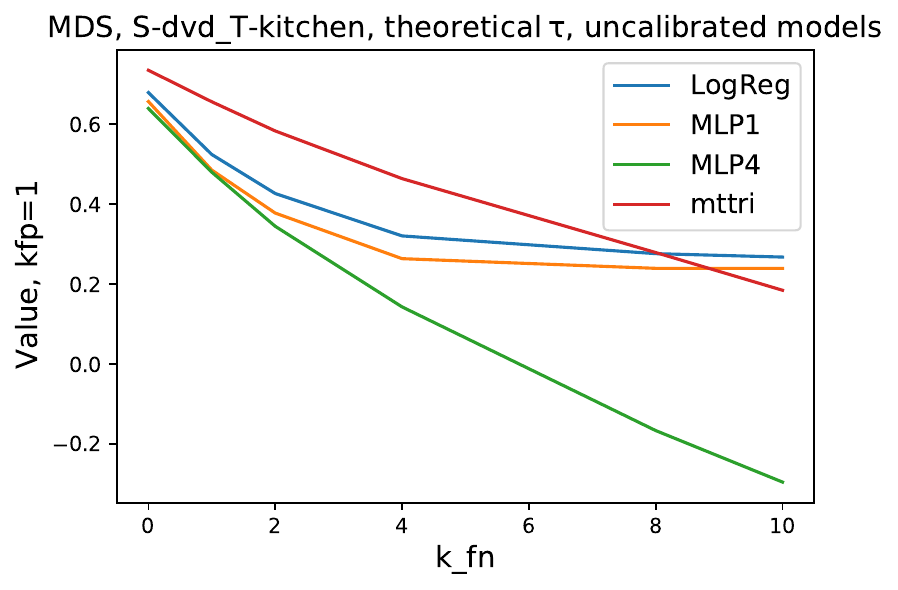} 
    \includegraphics[width=.245\linewidth]{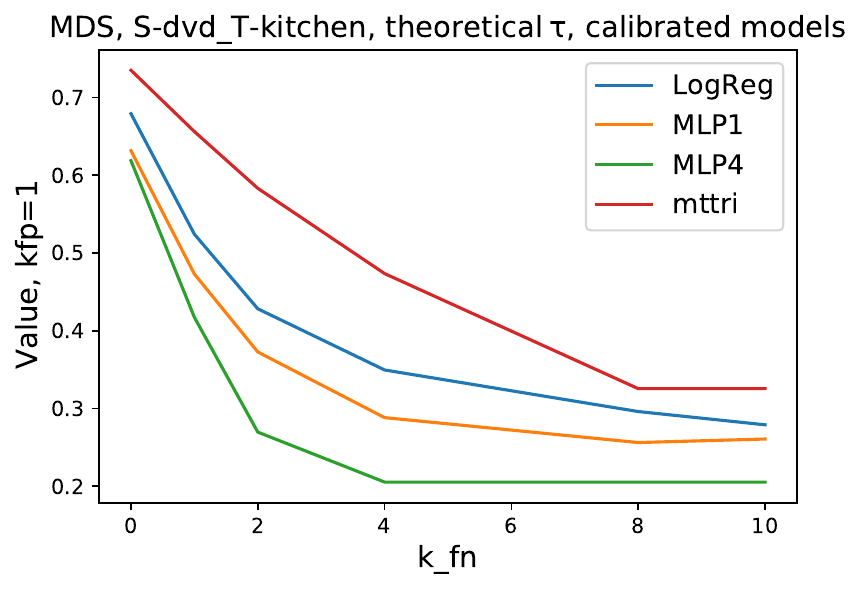}
    \includegraphics[width=.245\linewidth]{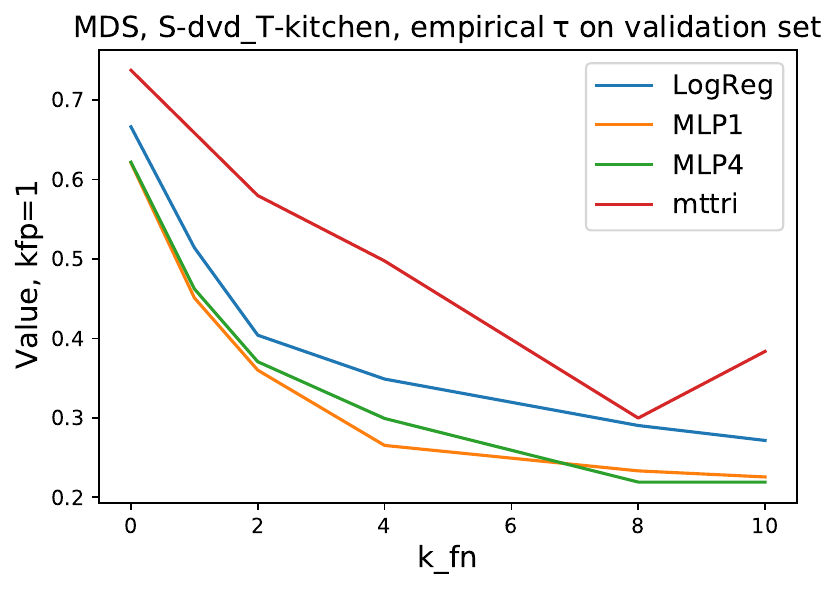}
    \includegraphics[width=.245\linewidth]{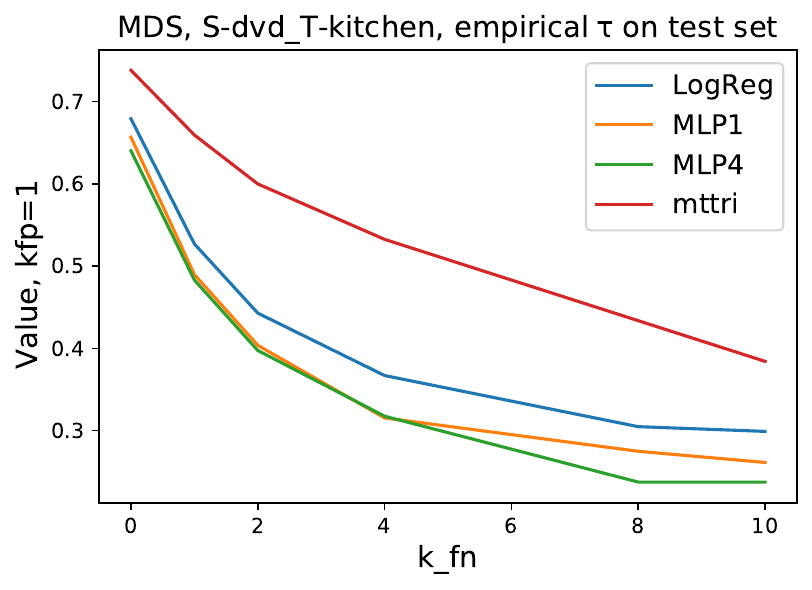}
    \includegraphics[width=.245\linewidth]{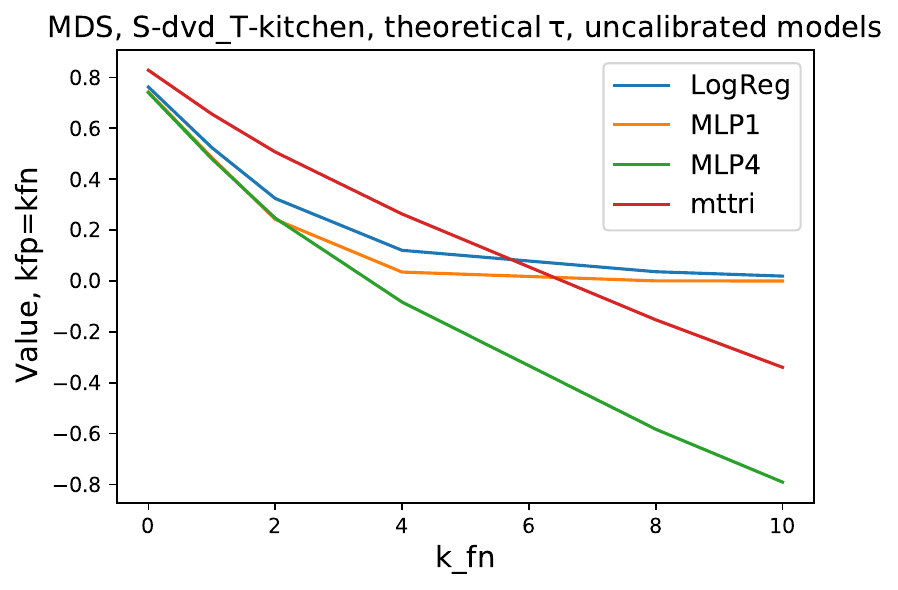} 
    \includegraphics[width=.245\linewidth]{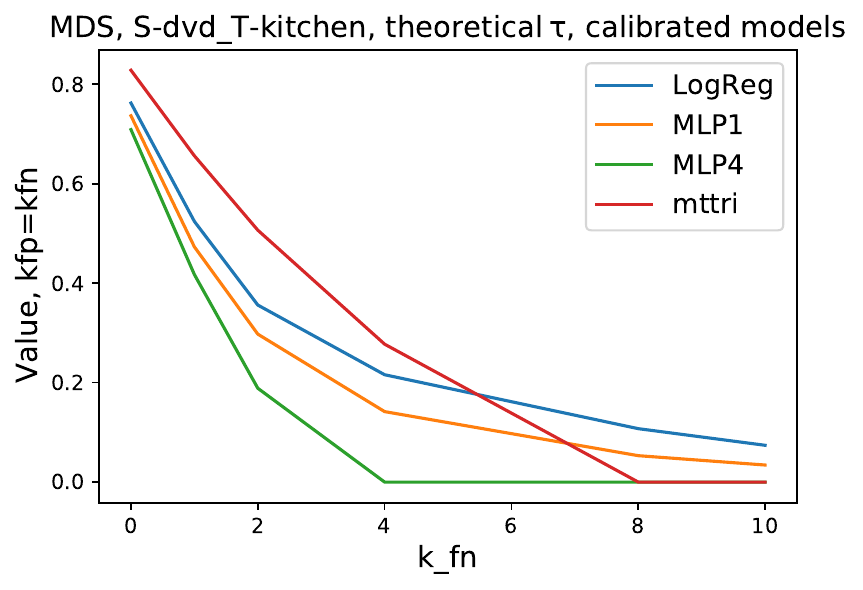}
    \includegraphics[width=.245\linewidth]{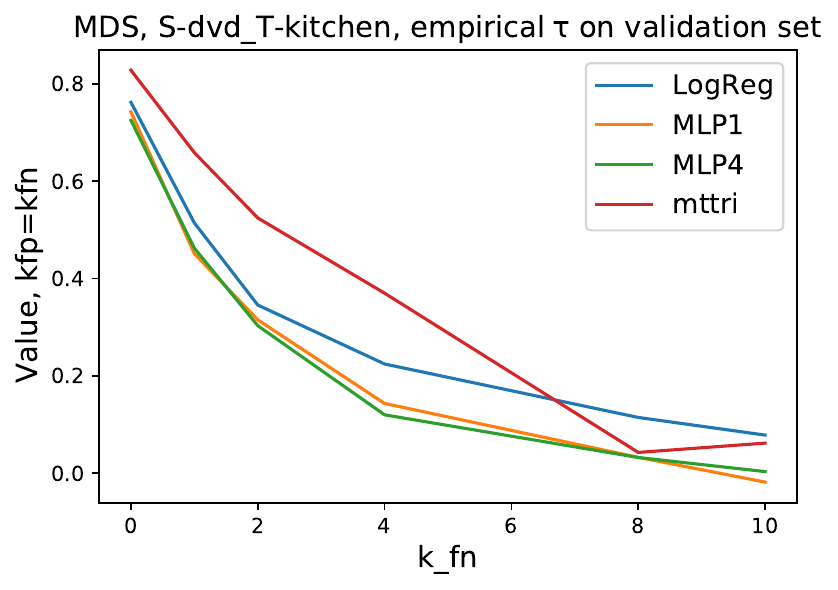}
    \includegraphics[width=.245\linewidth]{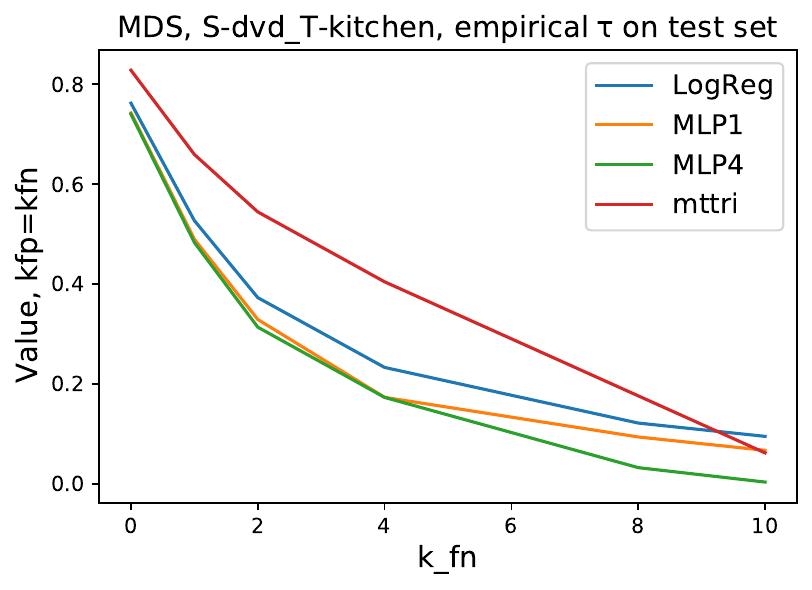}
    
    \includegraphics[width=.245\linewidth]{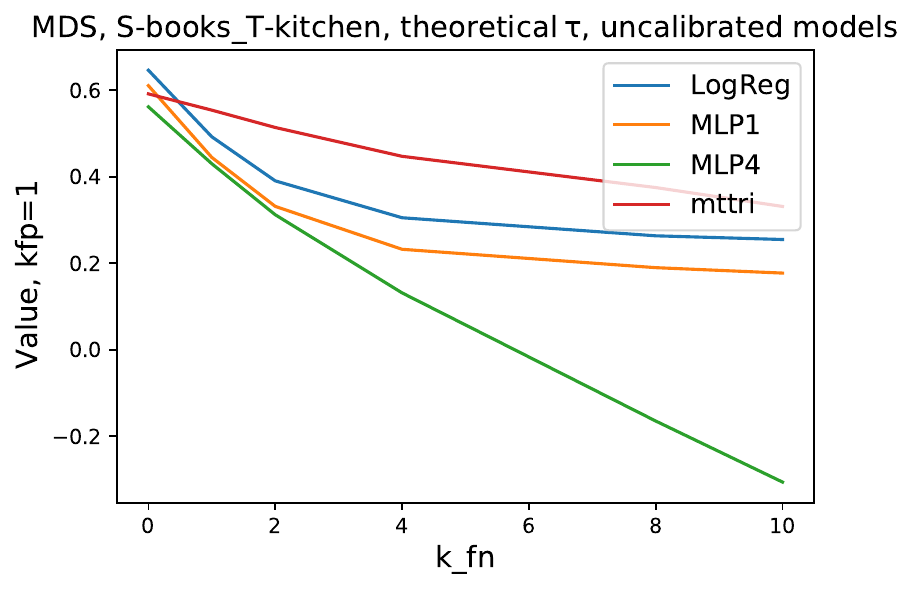} 
    \includegraphics[width=.245\linewidth]{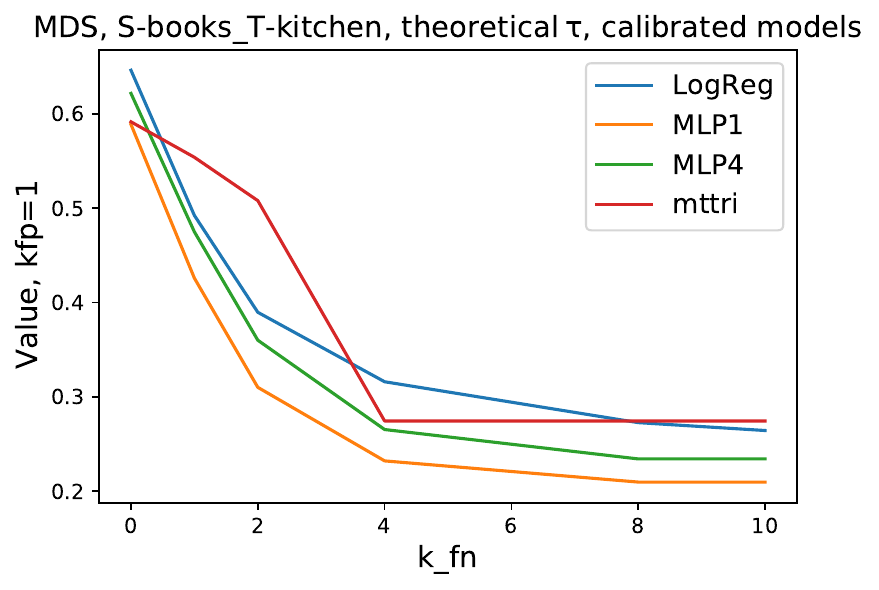}
    \includegraphics[width=.245\linewidth]{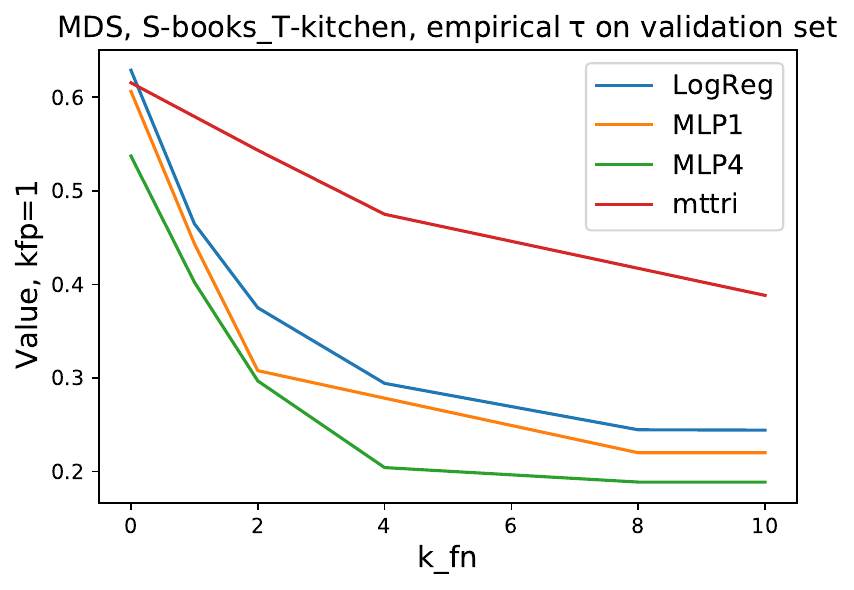}
    \includegraphics[width=.245\linewidth]{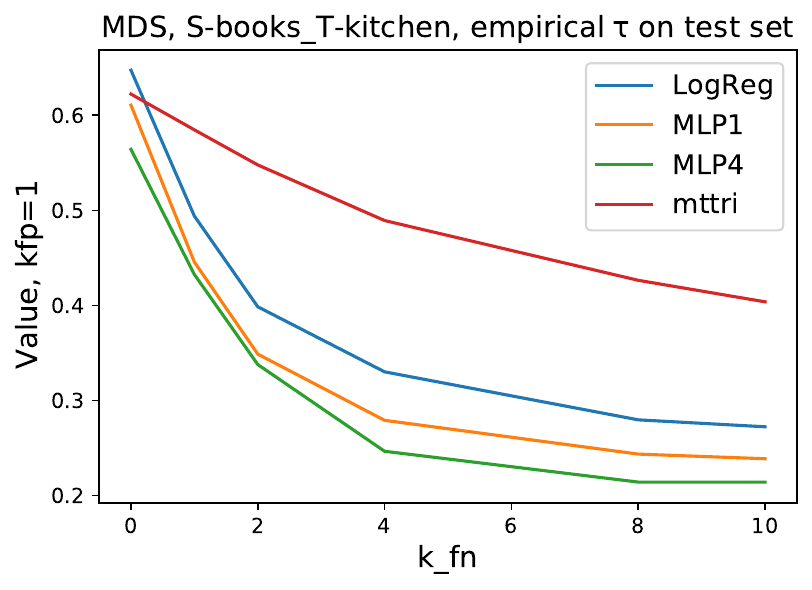}
    \includegraphics[width=.245\linewidth]{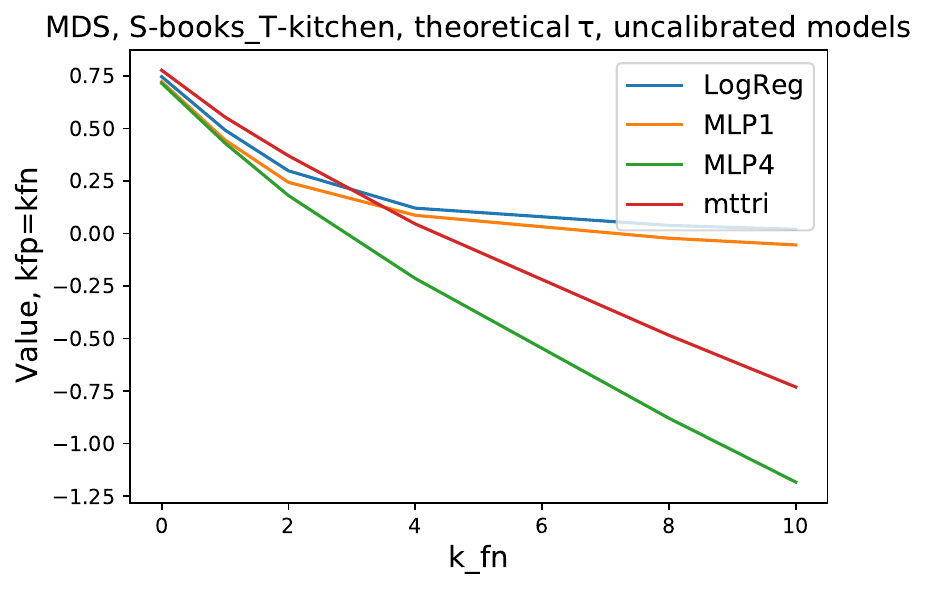} 
    \includegraphics[width=.245\linewidth]{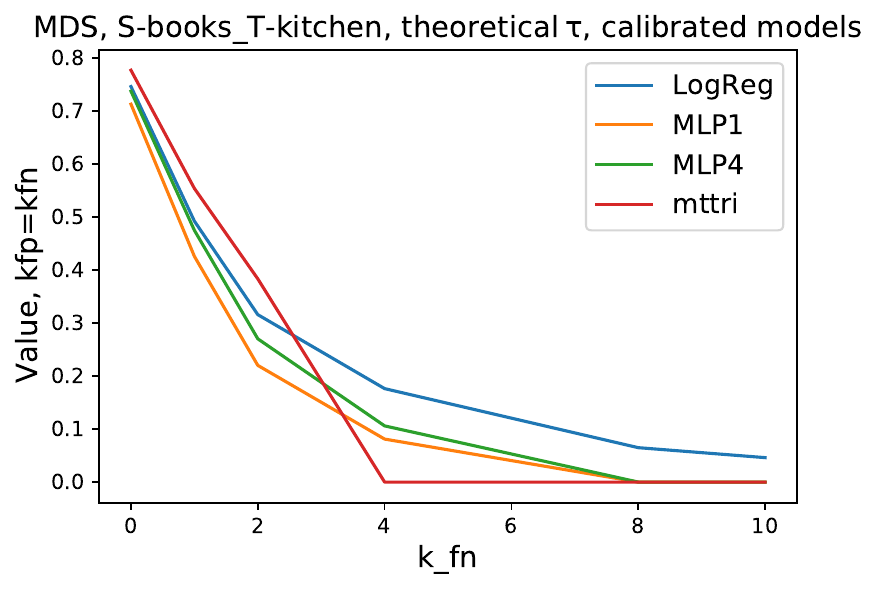}
    \includegraphics[width=.245\linewidth]{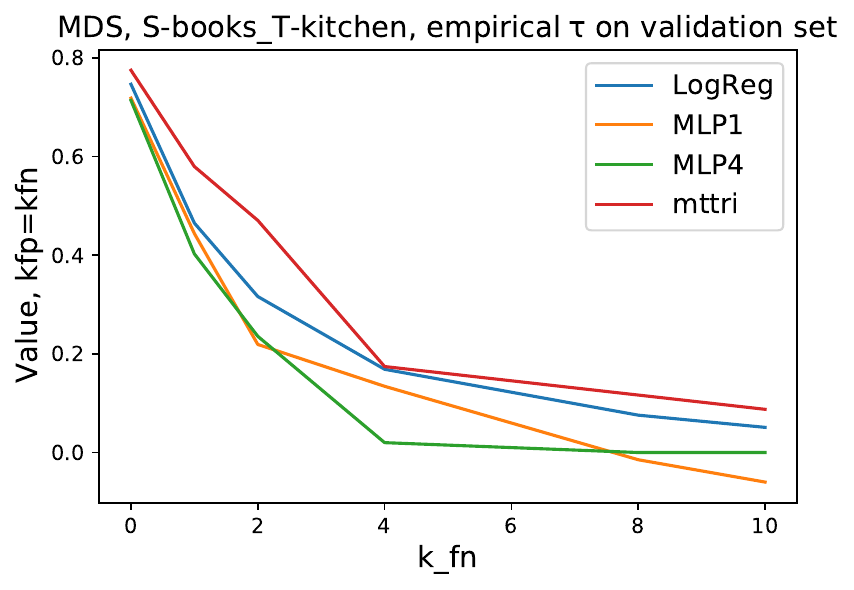}
    \includegraphics[width=.245\linewidth]{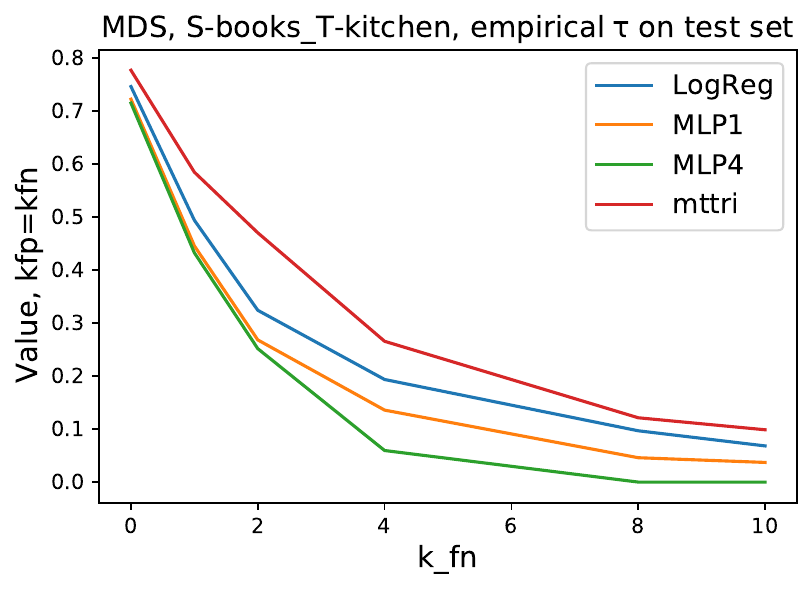}
    
    \includegraphics[width=.245\linewidth]{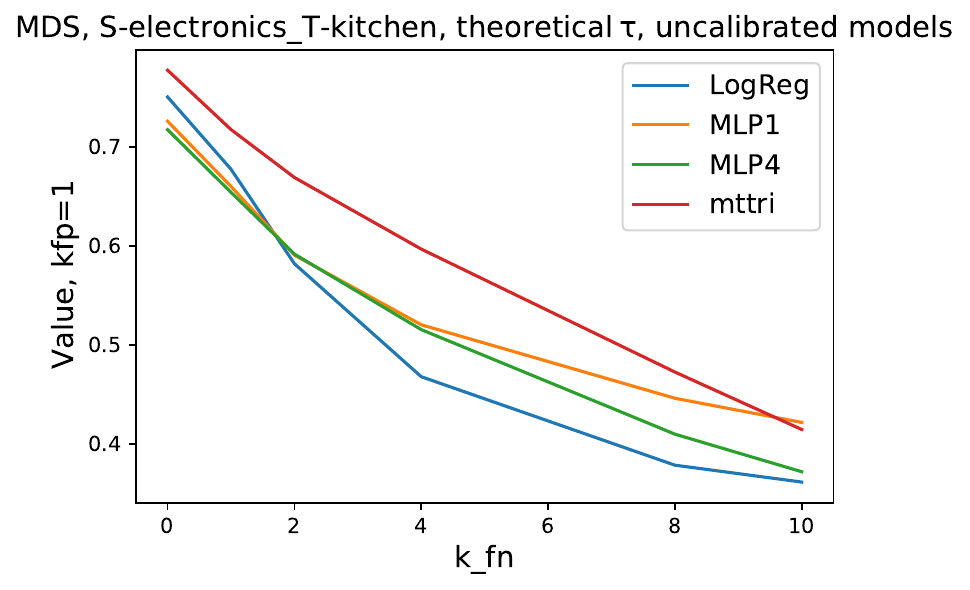} 
    \includegraphics[width=.245\linewidth]{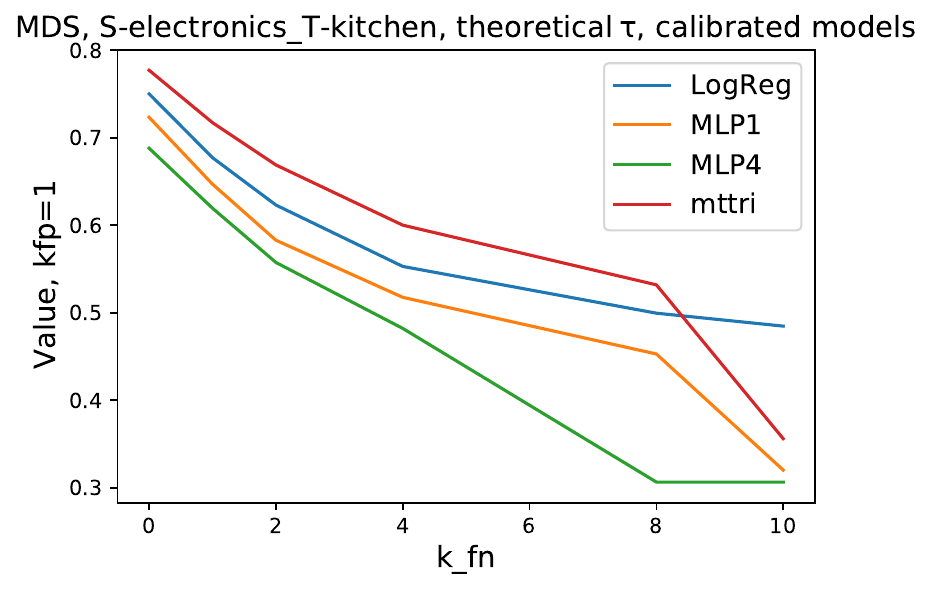}
    \includegraphics[width=.245\linewidth]{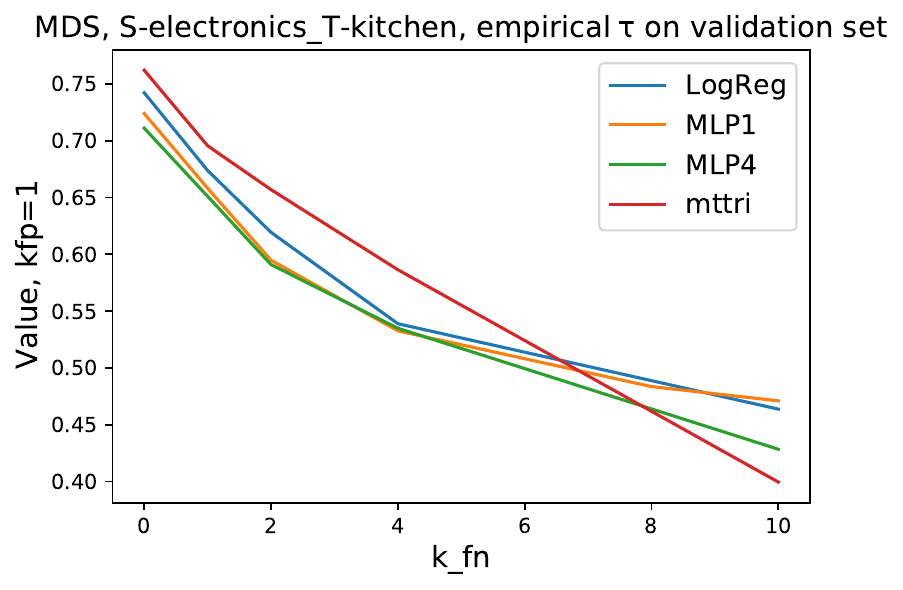}
    \includegraphics[width=.245\linewidth]{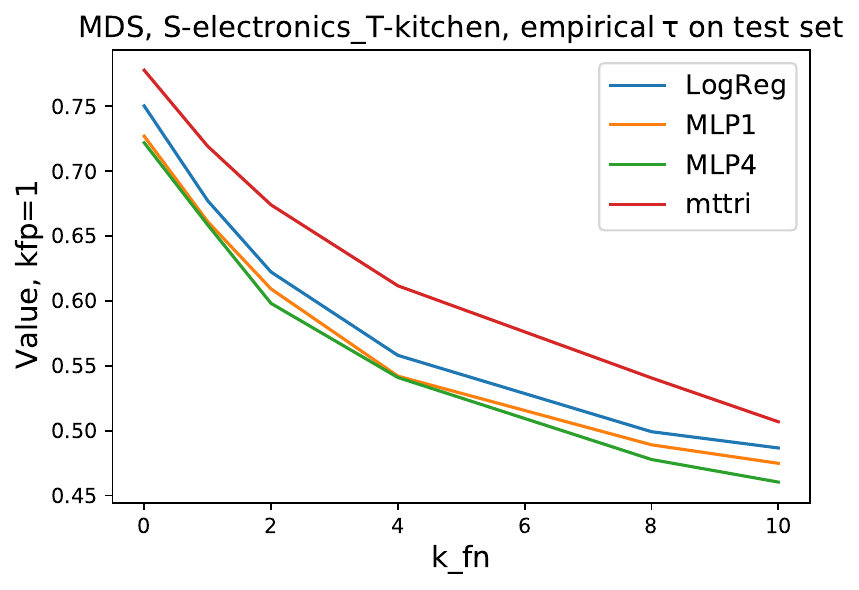}
    \includegraphics[width=.245\linewidth]{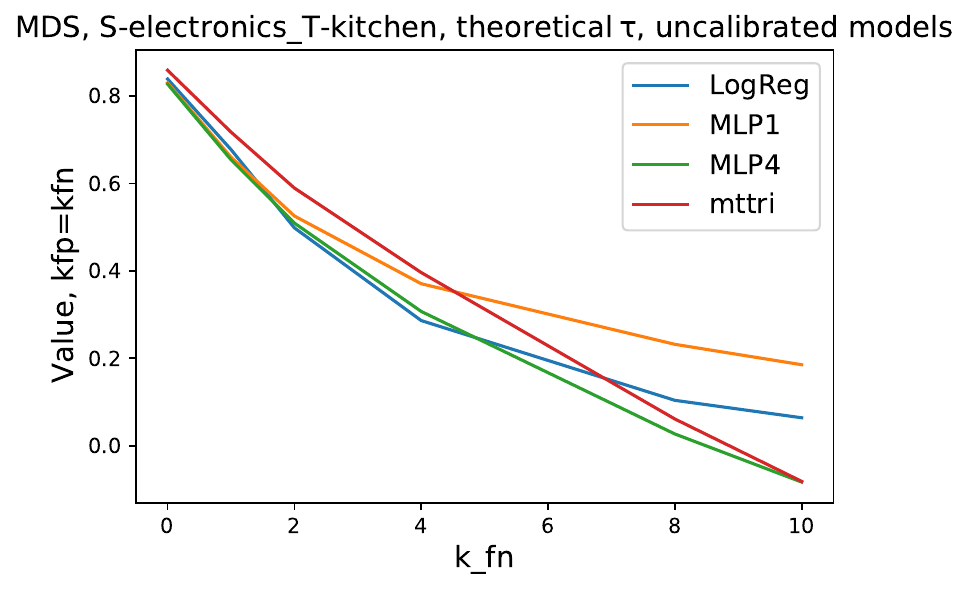} 
    \includegraphics[width=.245\linewidth]{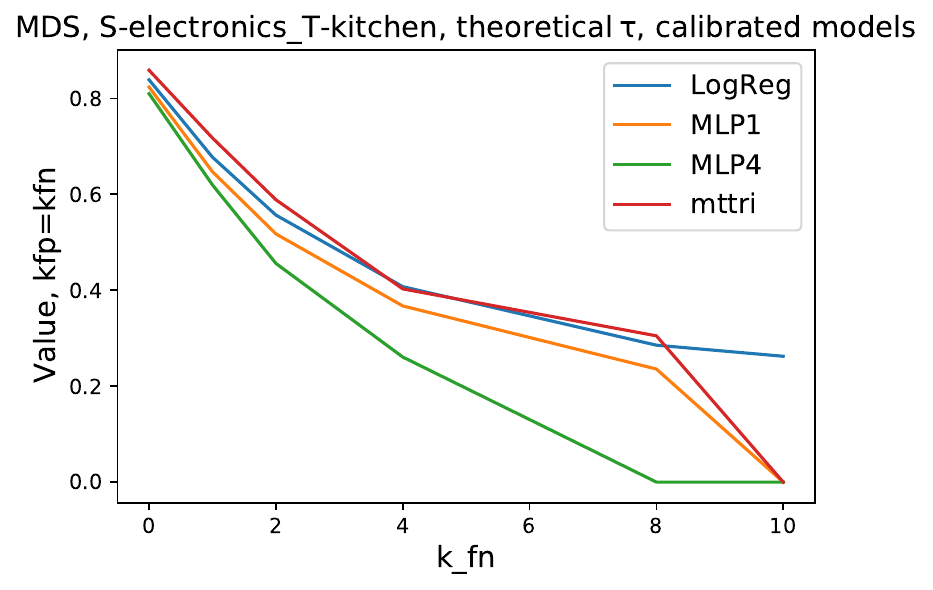}
    \includegraphics[width=.245\linewidth]{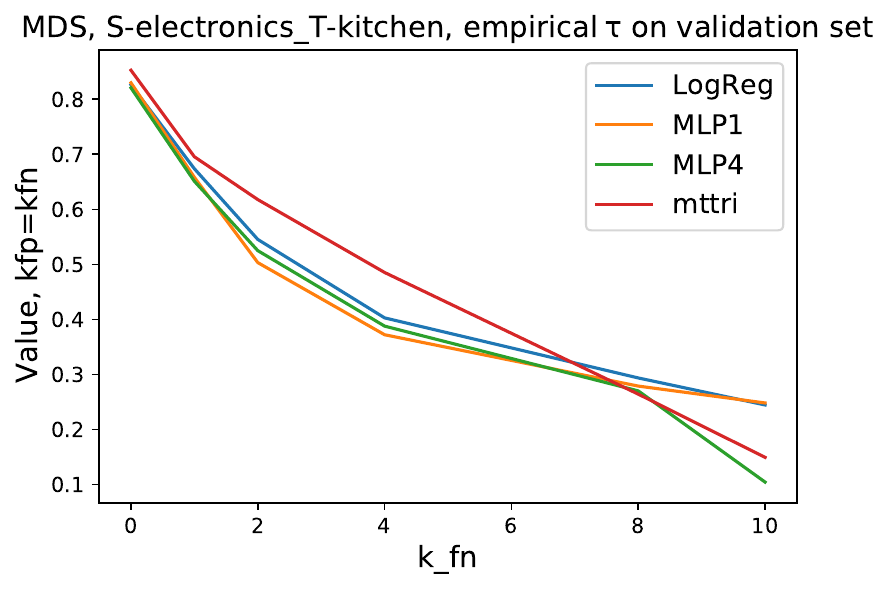}
    \includegraphics[width=.245\linewidth]{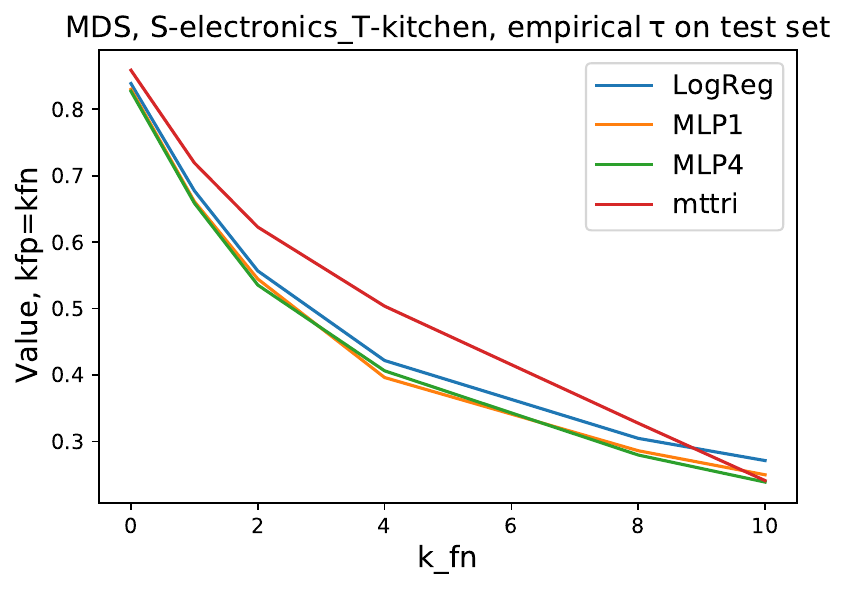}
    
    \caption{\label{fig:MDS_value_kitchen}Value curves on Multi Domain Sentiment dataset for increasing $k_{fn}$, TARGET = 'Kitchen'. We use S-SOURCE\_T-TARGET format in the sub-figure titles, values show the performance of each model trained on a source domain and tested on a target domain.}
\end{figure*}%%
\newpage
\subsubsection{Multi-class datasets - Supplementary Results}

\begin{figure*}[!htbp]
 \centering
    
    \includegraphics[width=.245\linewidth]{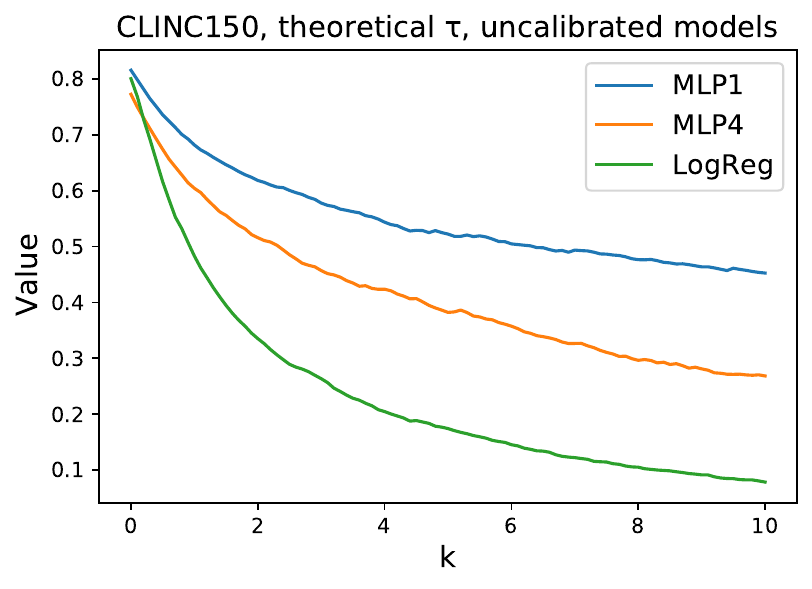}
    \includegraphics[width=.245\linewidth]{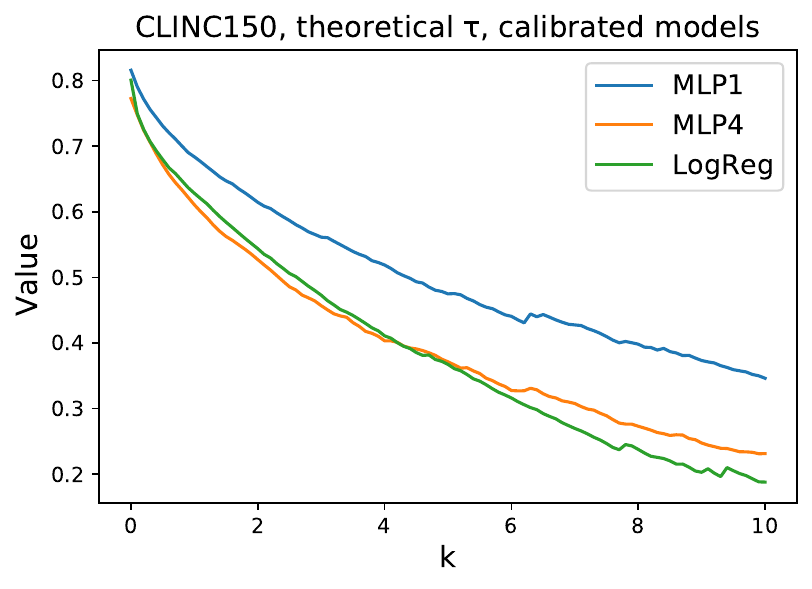}
    \includegraphics[width=.245\linewidth]{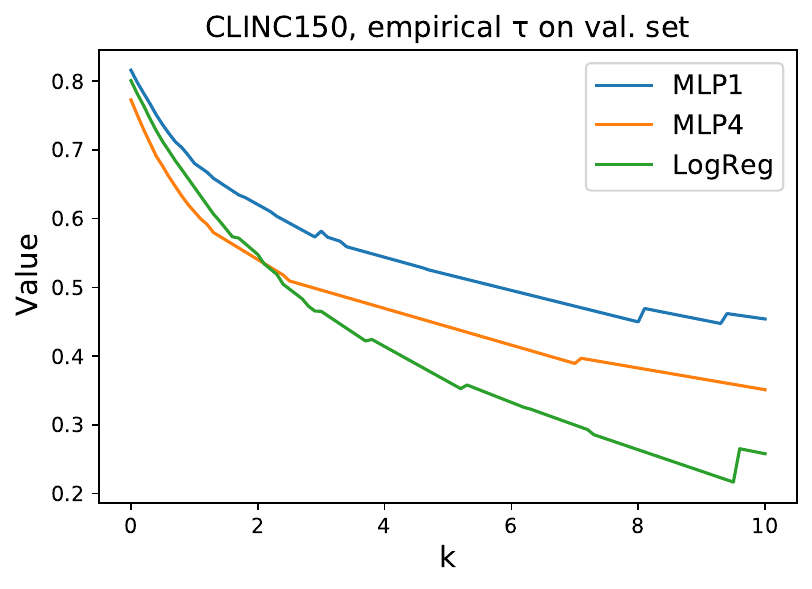}
    \includegraphics[width=.245\linewidth]{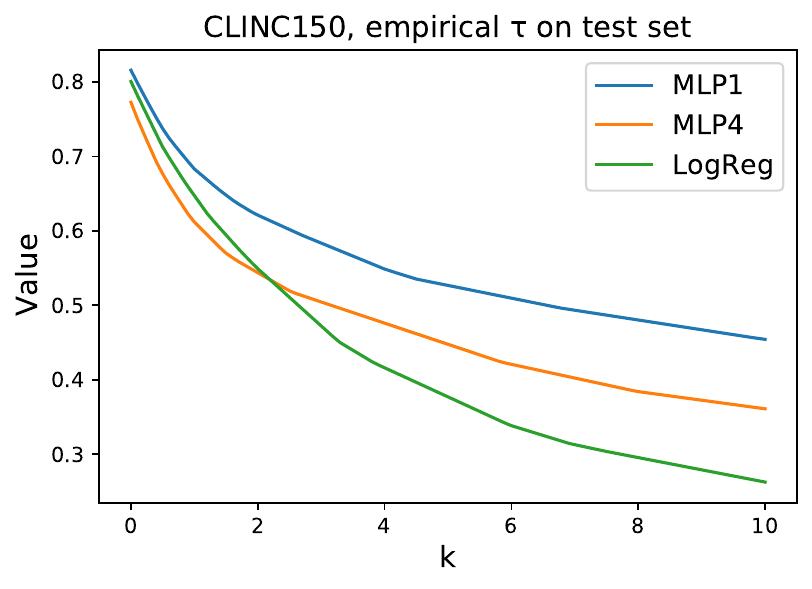}
    \includegraphics[width=.245\linewidth]{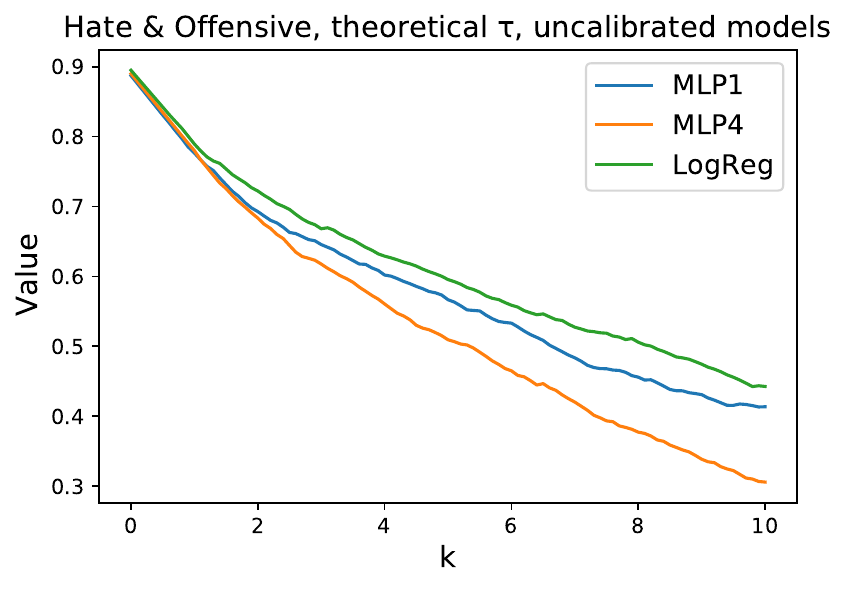}
    \includegraphics[width=.245\linewidth]{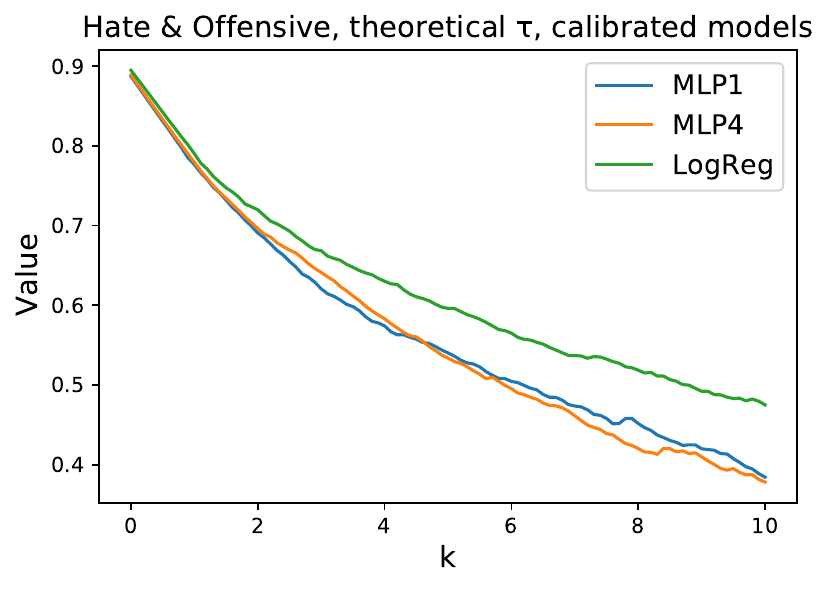}
    \includegraphics[width=.245\linewidth]{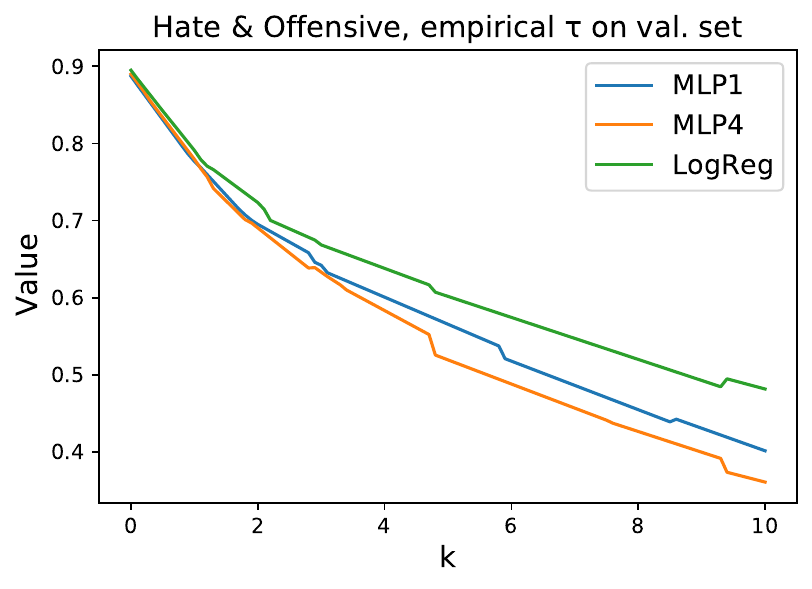}
    \includegraphics[width=.245\linewidth]{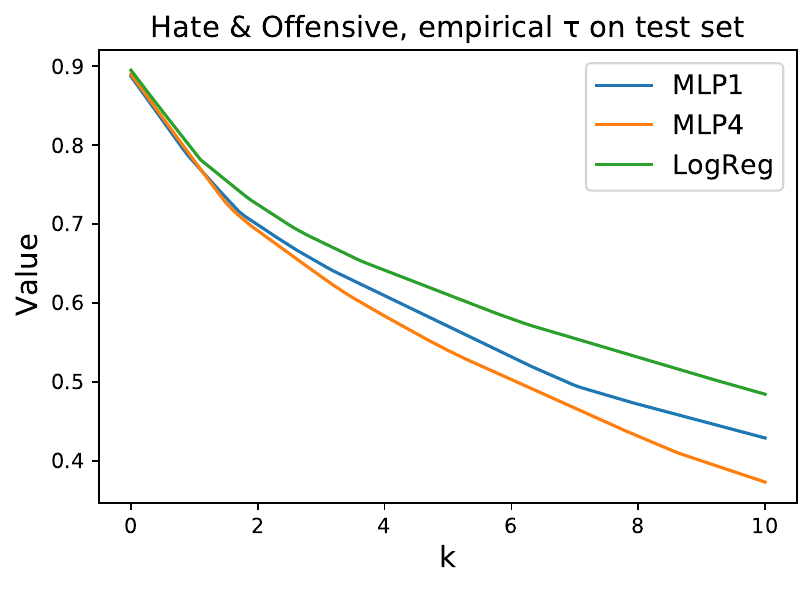}
    \includegraphics[width=.245\linewidth]{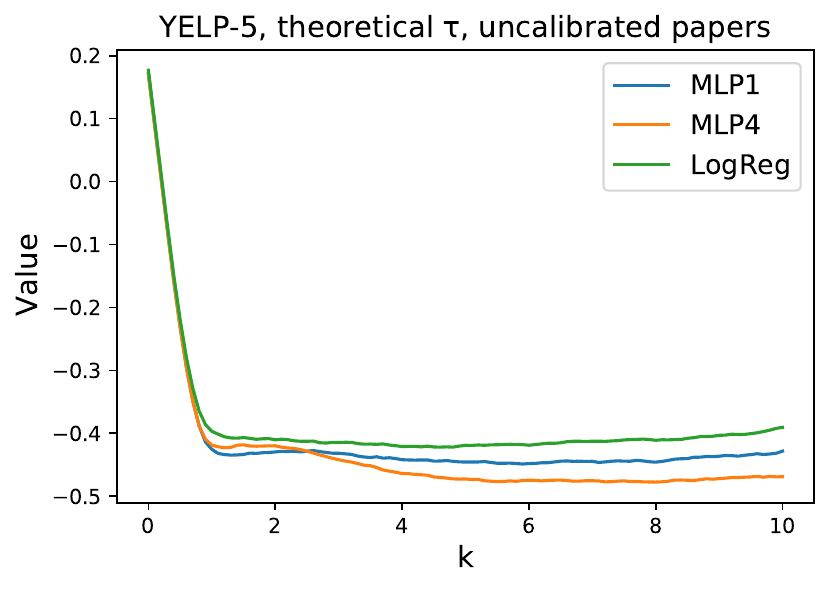}
    \includegraphics[width=.245\linewidth]{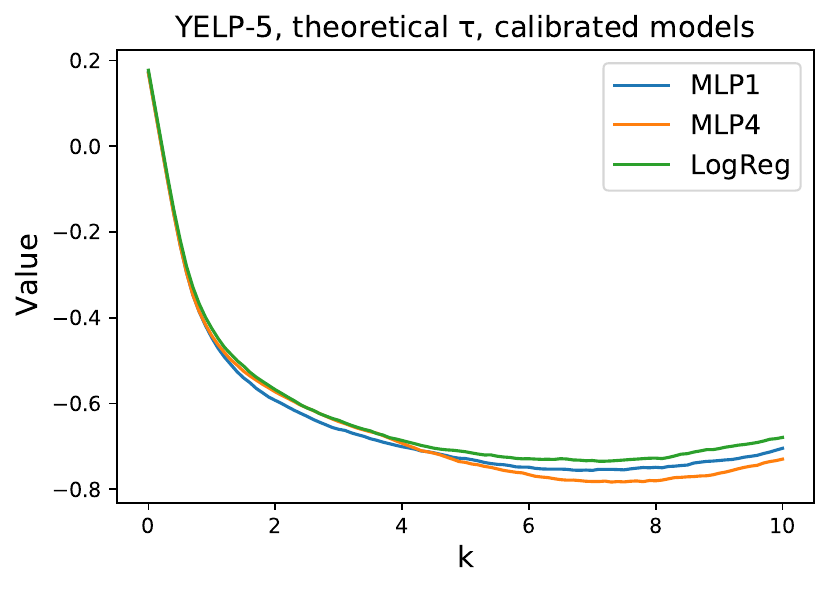}
    \includegraphics[width=.245\linewidth]{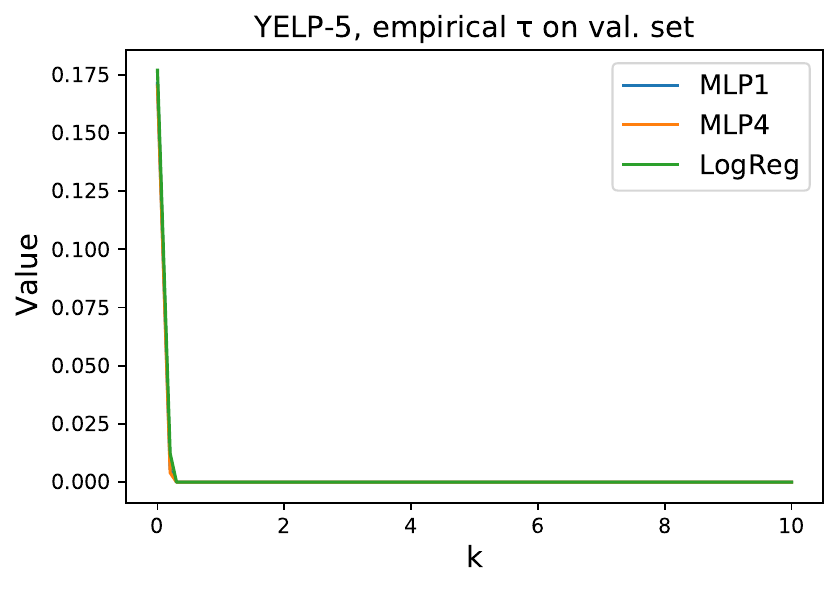}
    \includegraphics[width=.245\linewidth]{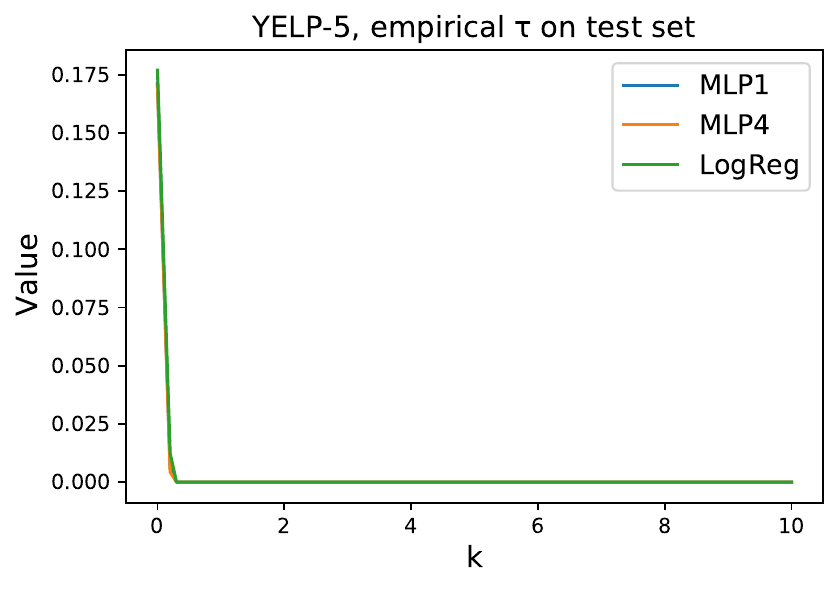}
    \includegraphics[width=.245\linewidth]{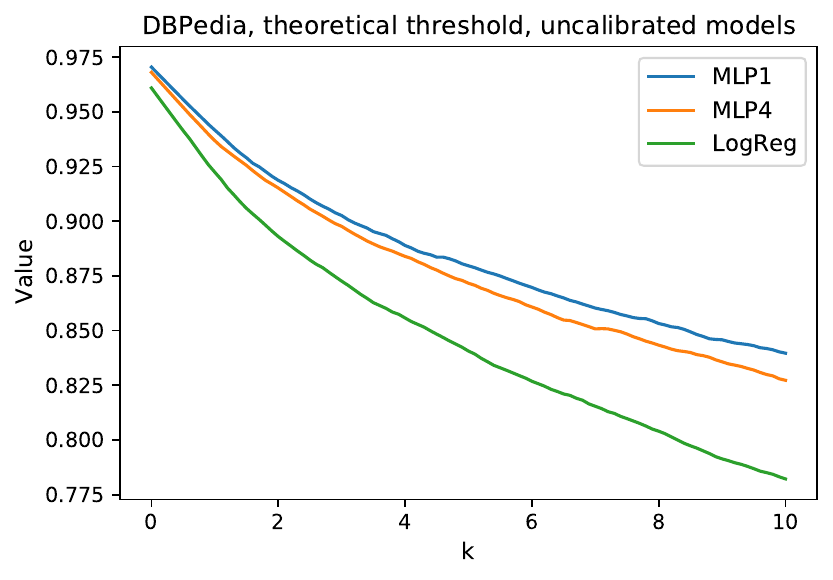}
    \includegraphics[width=.245\linewidth]{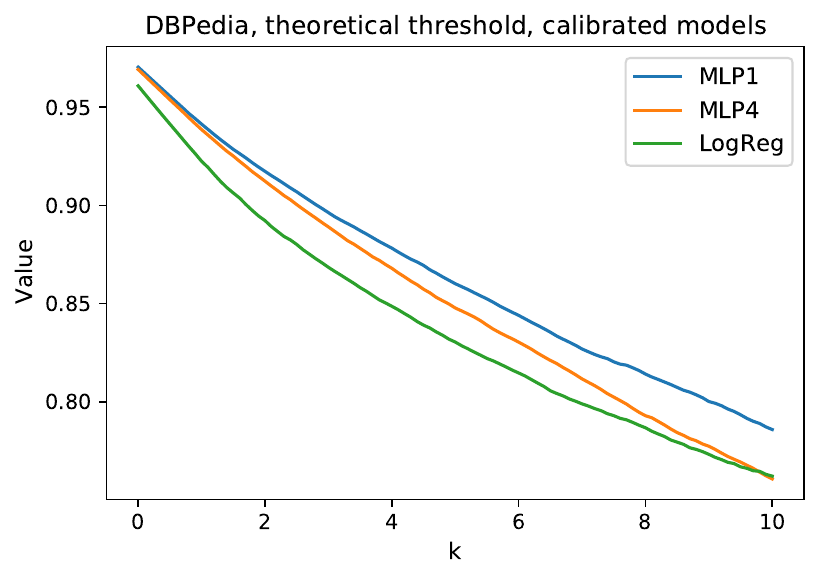}
    \includegraphics[width=.245\linewidth]{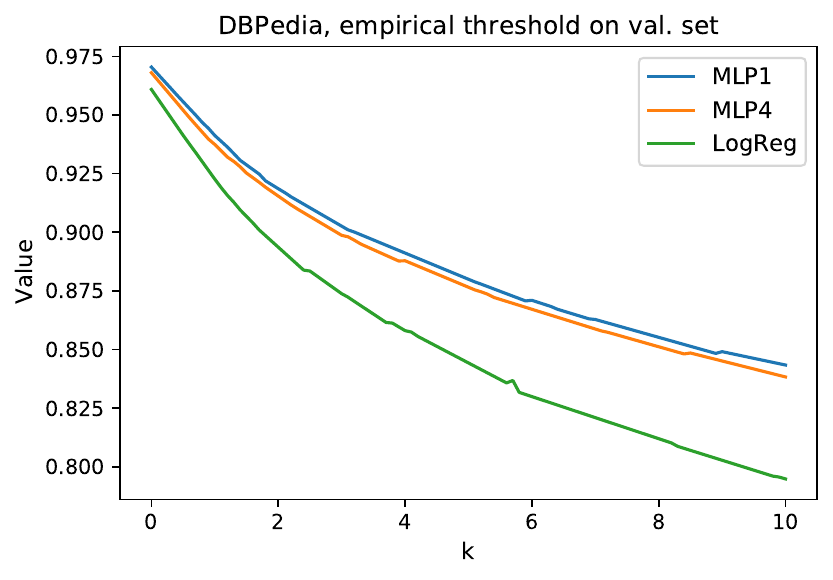}
    \includegraphics[width=.245\linewidth]{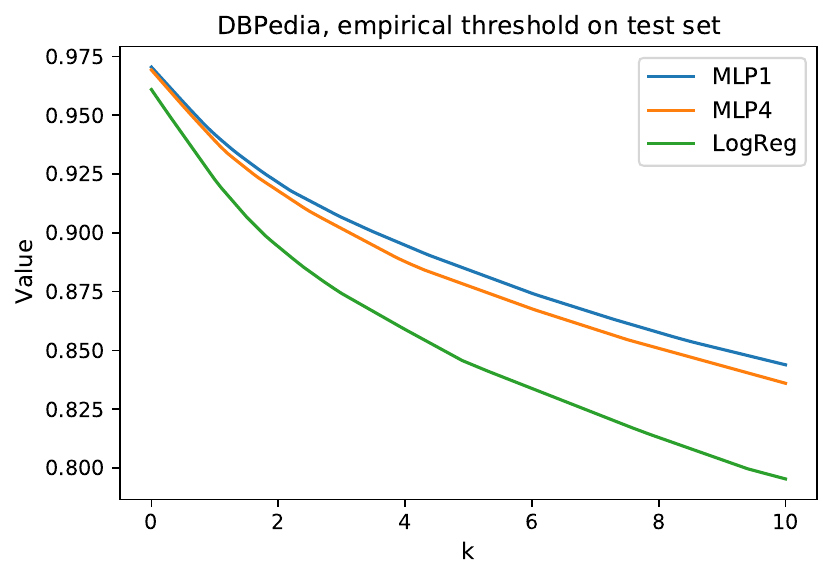}
    
    \caption{\label{fig:value_curve_mclass}Value curves of multi-class datasets for increasing $k$.}
      \vspace{-0.15in}
\end{figure*}%%

\begin{figure*}[!htbp]
 \centering
    \includegraphics[width=.32\linewidth]{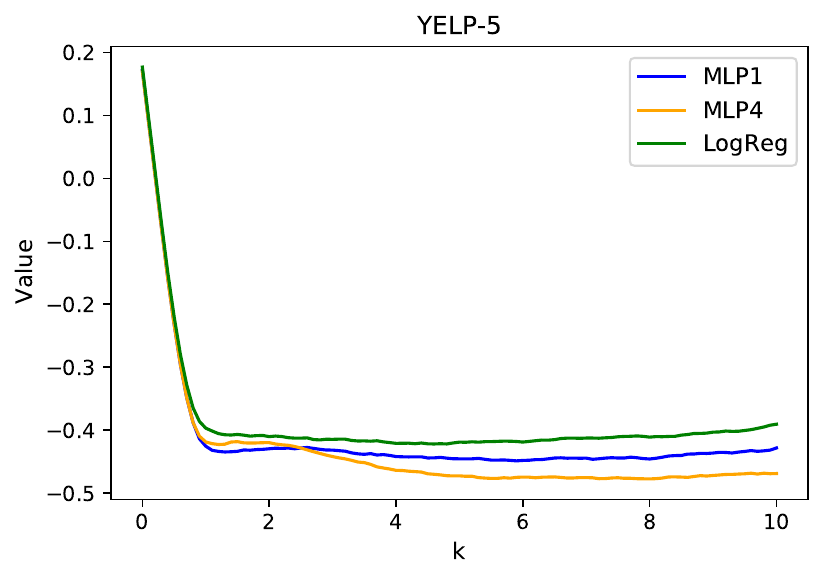} 
    \includegraphics[width=.32\linewidth]{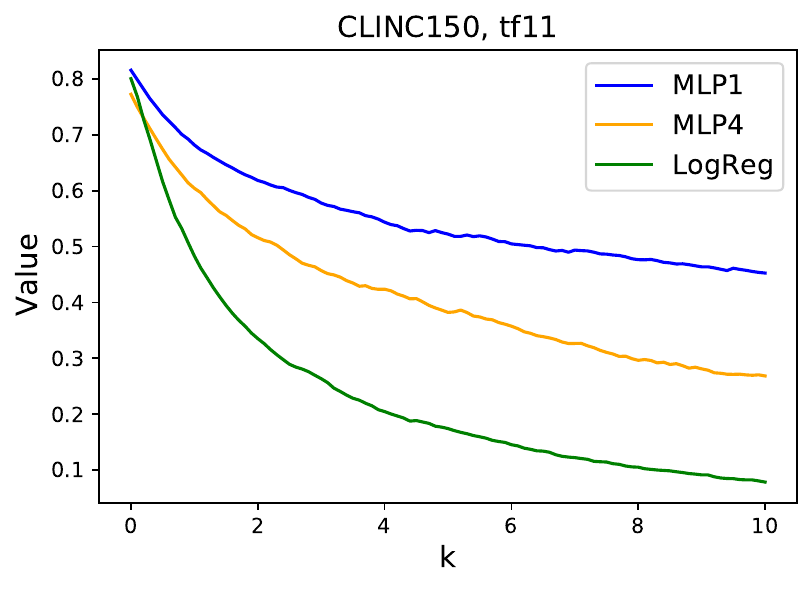}
    \includegraphics[width=.32\linewidth]{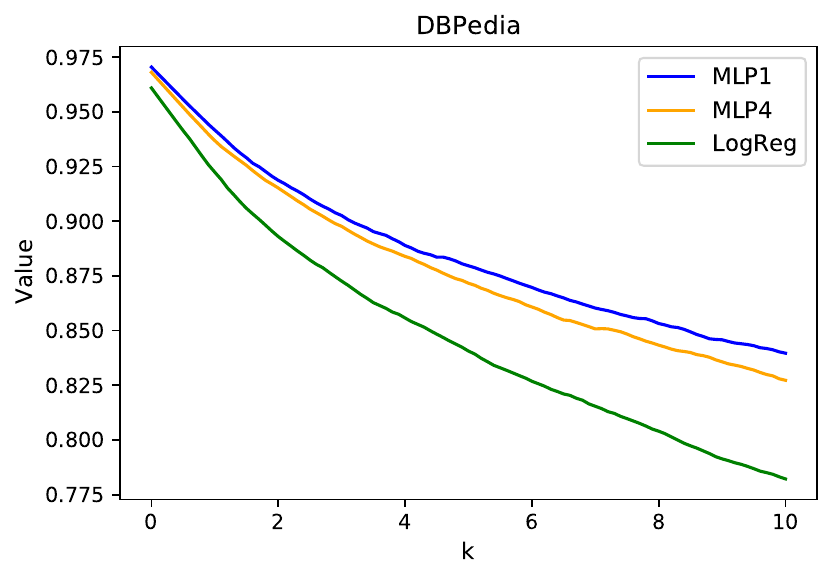}
    \includegraphics[width=.32\linewidth]{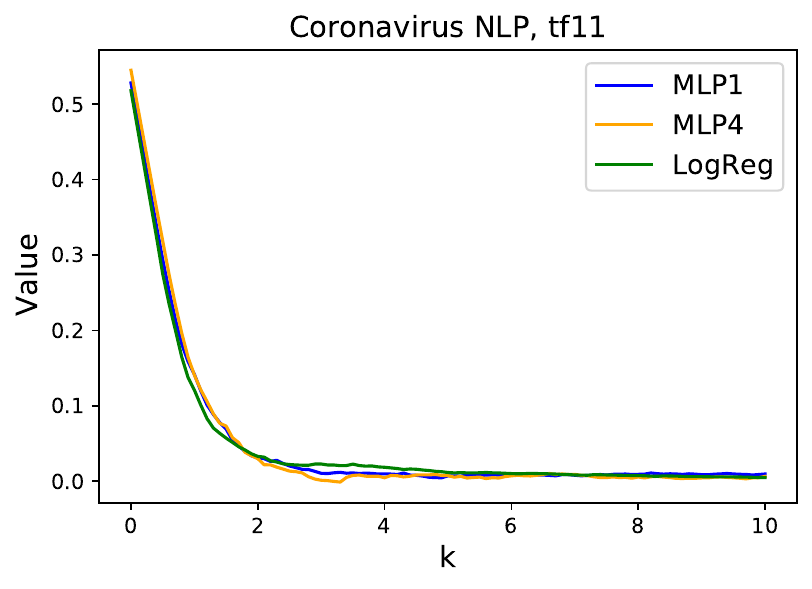} 
    \includegraphics[width=.32\linewidth]{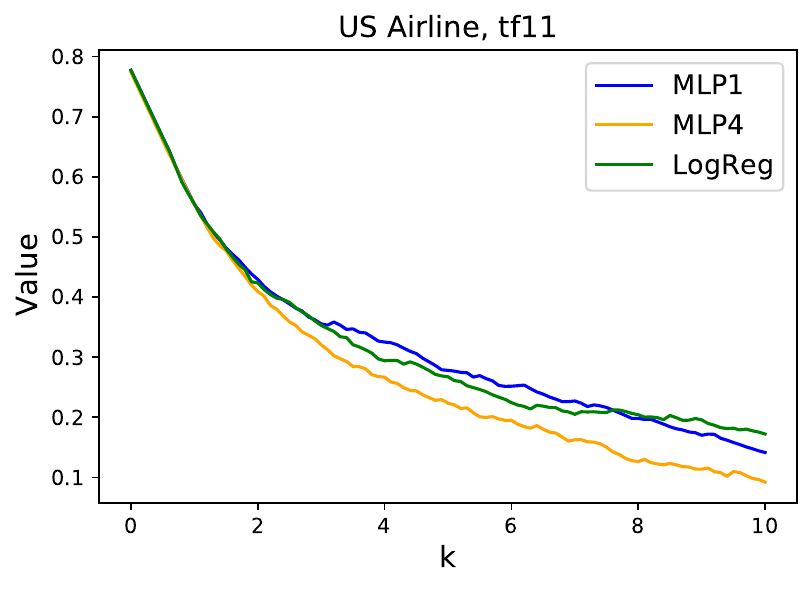}
    \includegraphics[width=.32\linewidth]{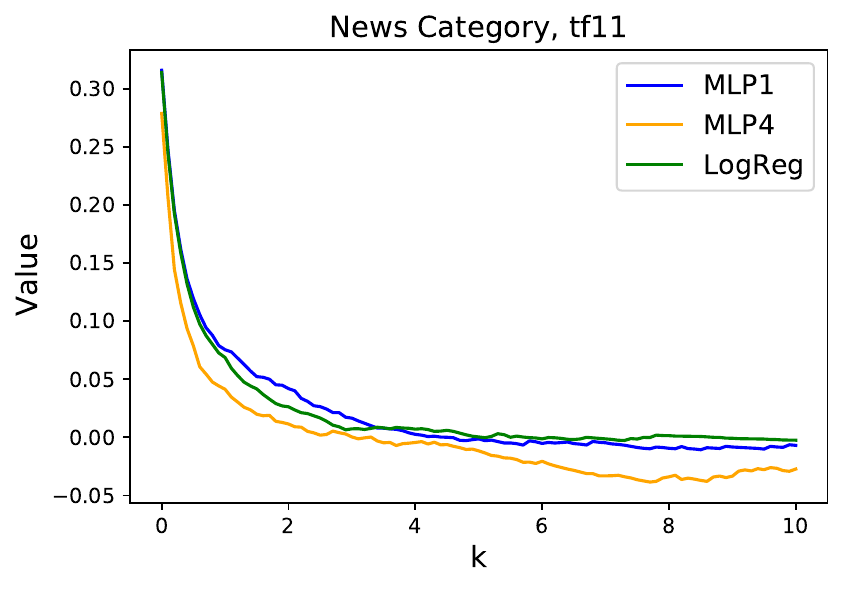}
    \includegraphics[width=.32\linewidth]{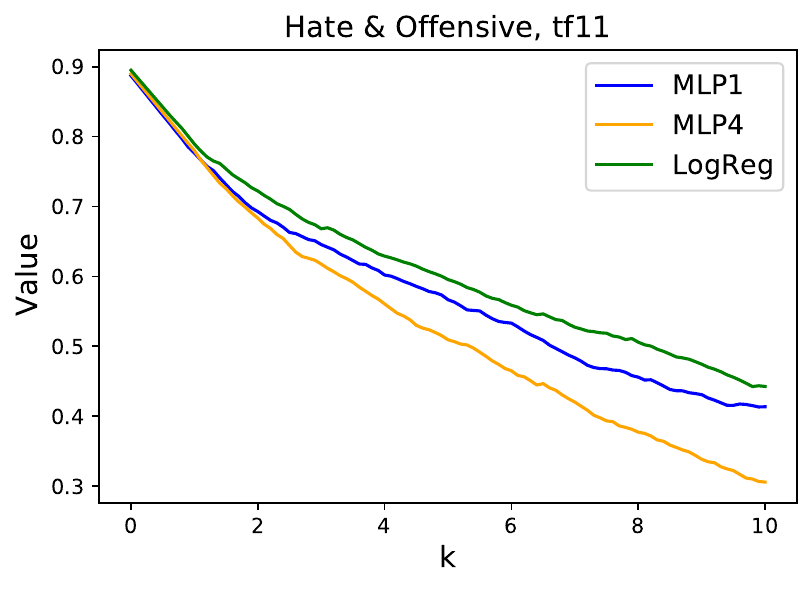}
    \caption{\label{fig:value_multiClass_Theo}Value curves with theoretical
      threshold for increasing $k$.}
      \vspace{-0.15in}
\end{figure*}%%

\begin{figure*}
 \centering
    \includegraphics[width=.3\linewidth]{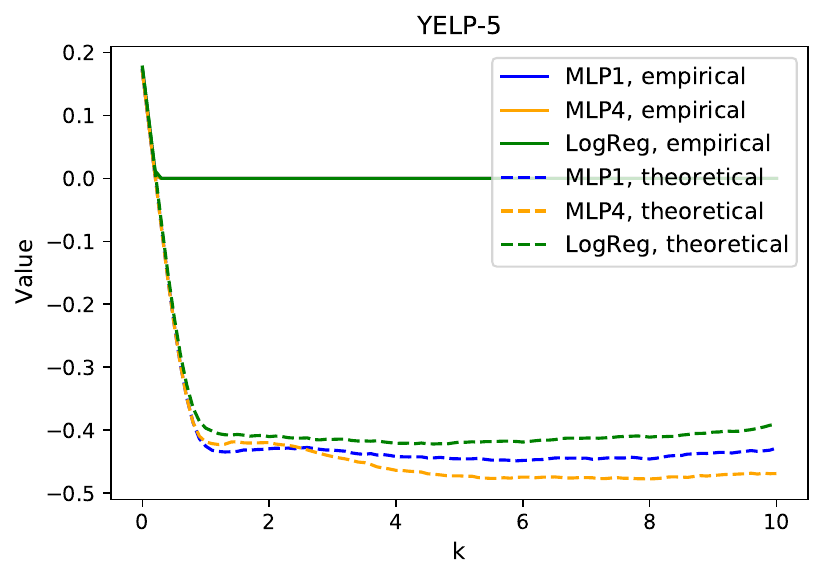} 
    \includegraphics[width=.3\linewidth]{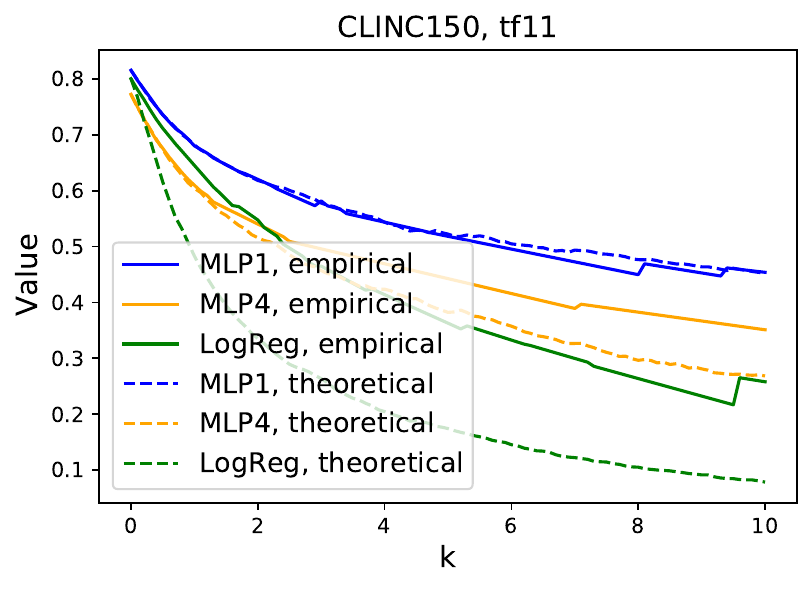}
    \includegraphics[width=.3\linewidth]{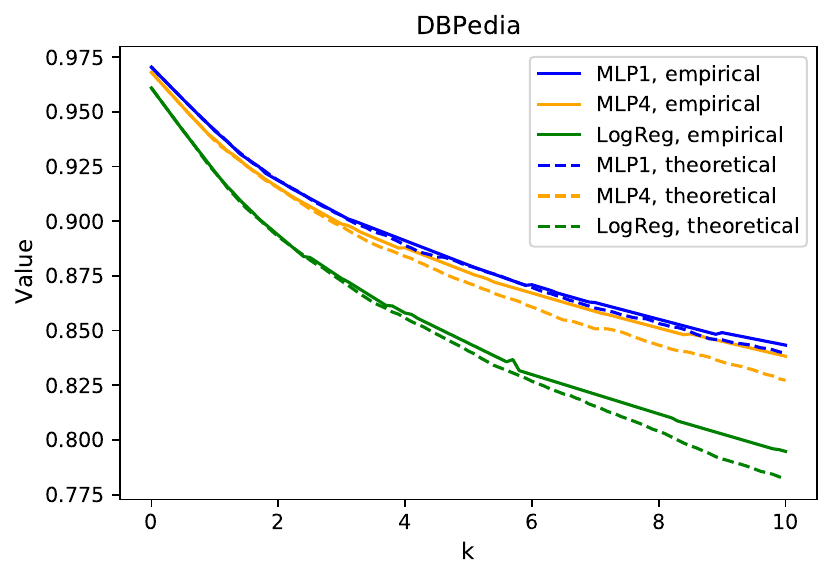} 
    
    \includegraphics[width=.3\linewidth]{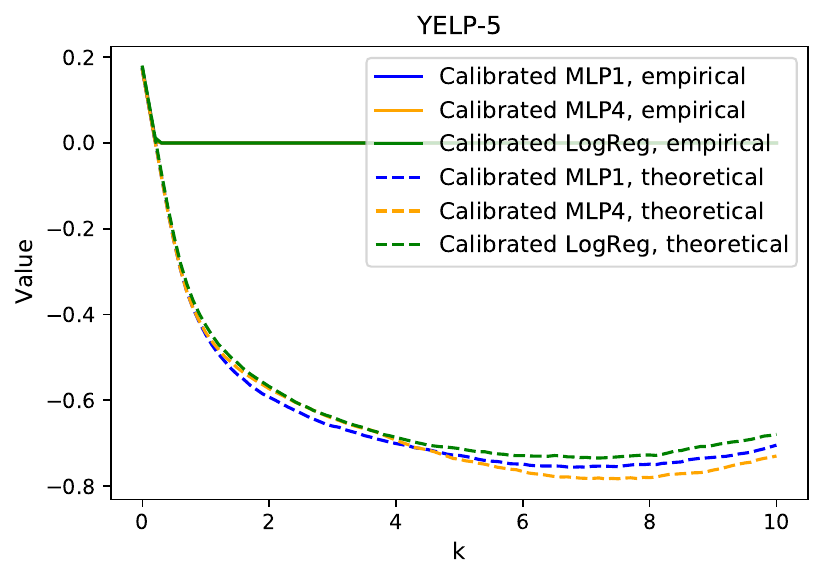} 
    \includegraphics[width=.3\linewidth]{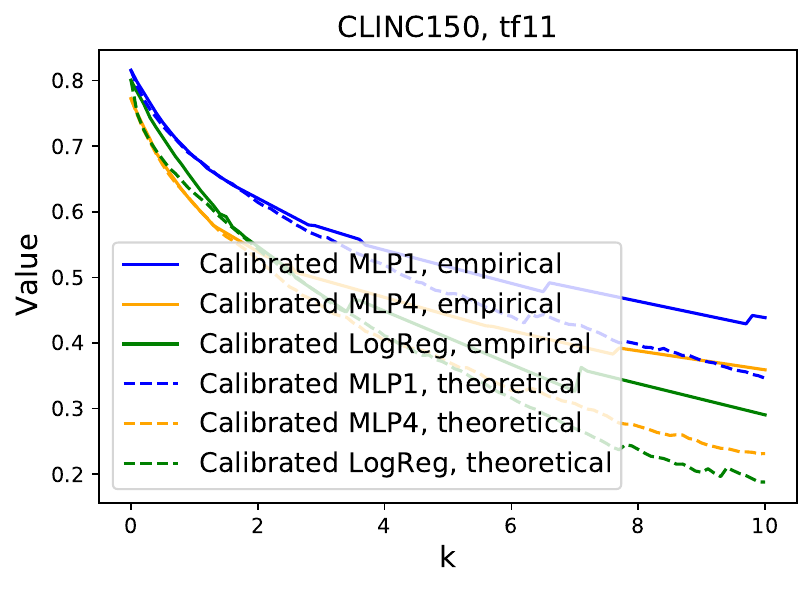}
    \includegraphics[width=.3\linewidth]{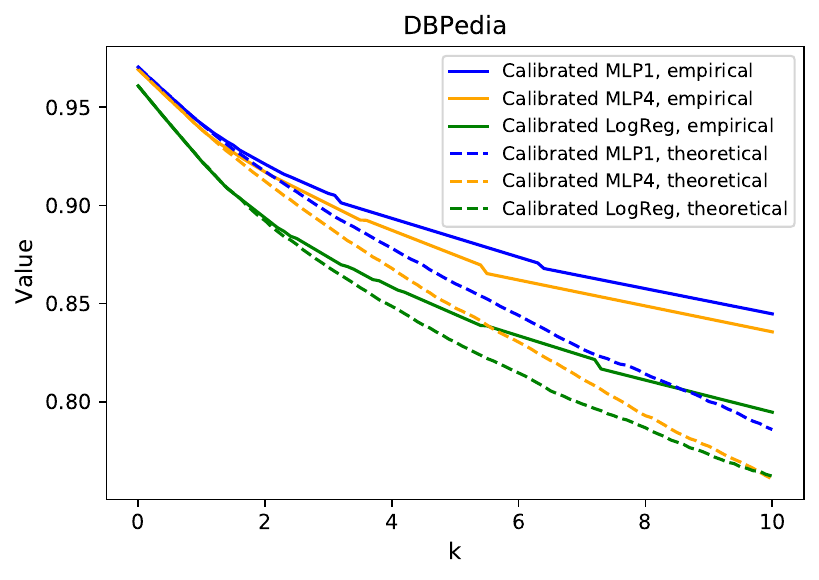} 
    \includegraphics[width=.3\linewidth]{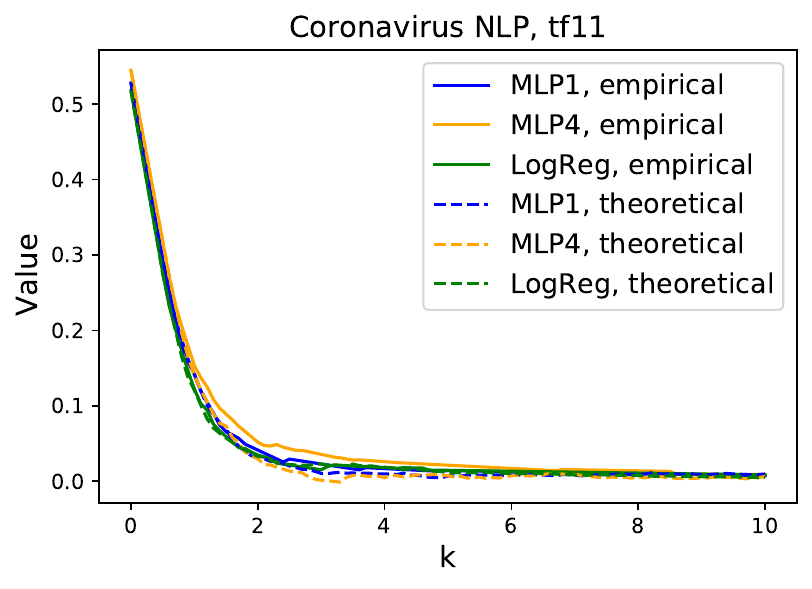} 
    \includegraphics[width=.3\linewidth]{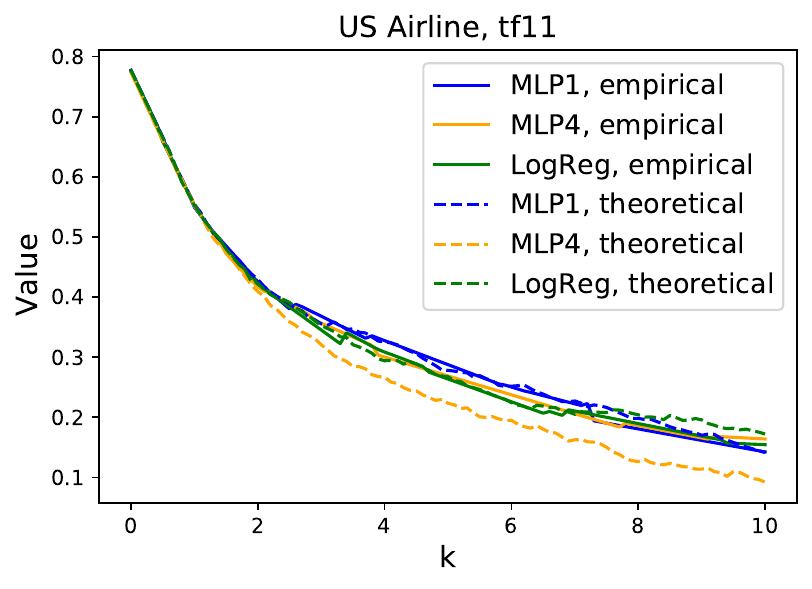}
    \includegraphics[width=.3\linewidth]{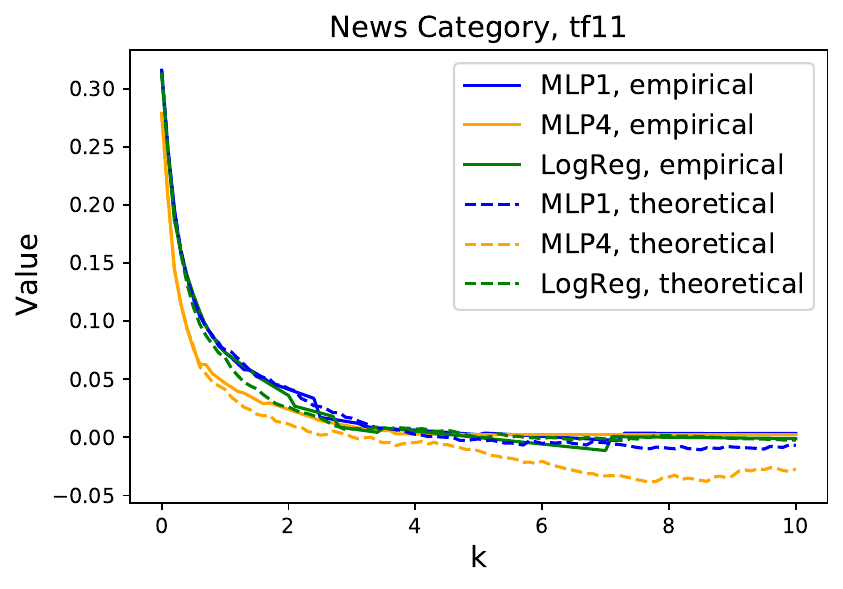}
    \includegraphics[width=.3\linewidth]{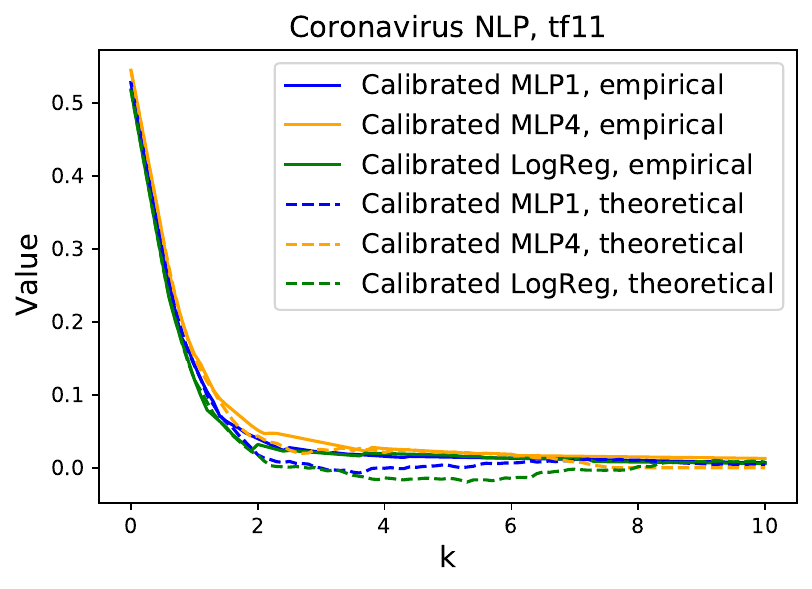} 
    \includegraphics[width=.3\linewidth]{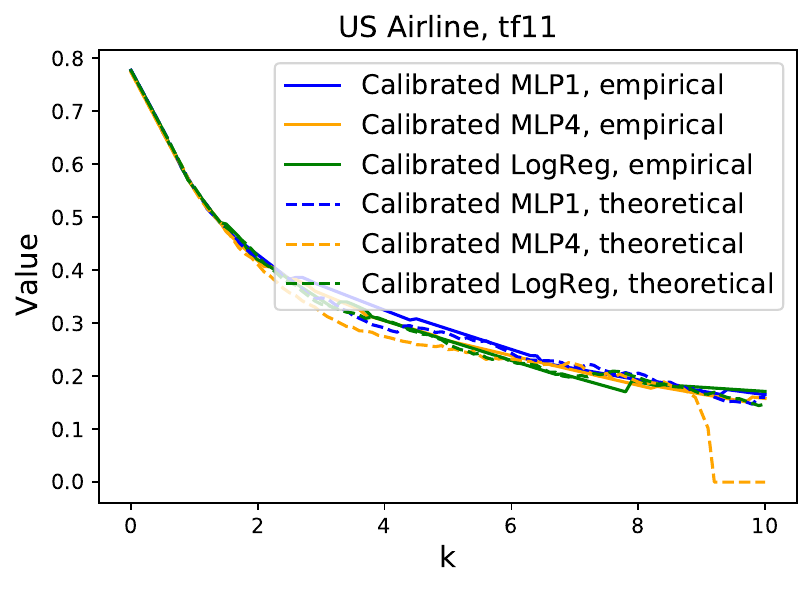}
    \includegraphics[width=.3\linewidth]{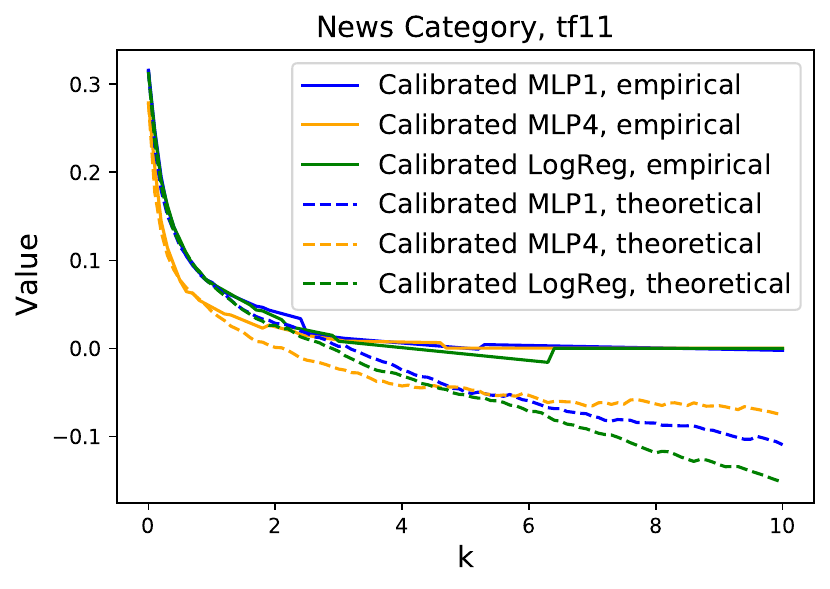} 
    
    \includegraphics[width=.3\linewidth]{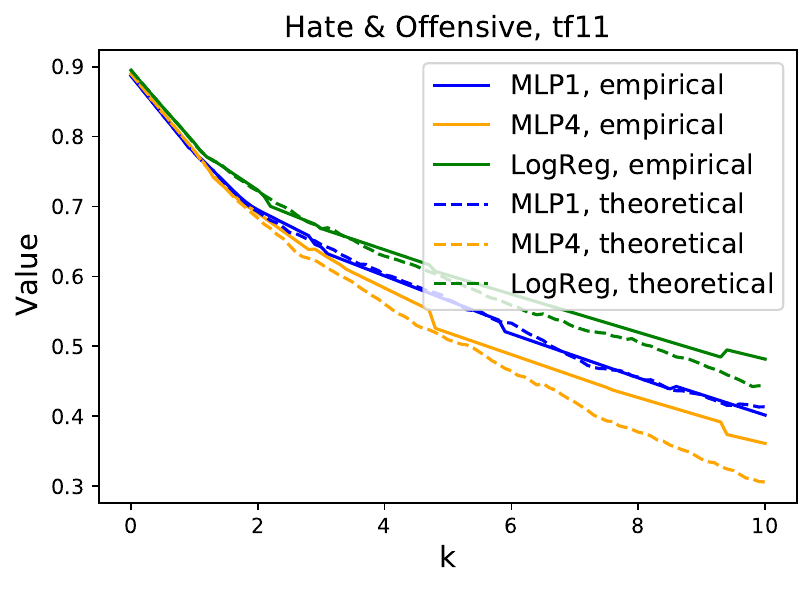}
    \includegraphics[width=.3\linewidth]{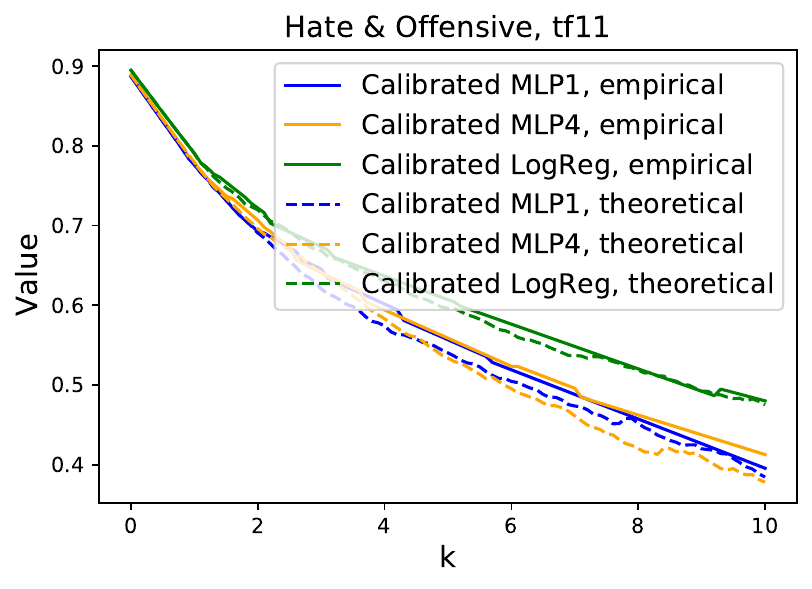}

    \caption{\label{fig:value_curve_optScaled_All}Value curves with theoretical and empirical
      threshold (on the validation set) for increasing $k$.}
      \vspace{-0.15in}
\end{figure*}%%

\begin{figure*}
 \centering
    \includegraphics[width=.3\linewidth]{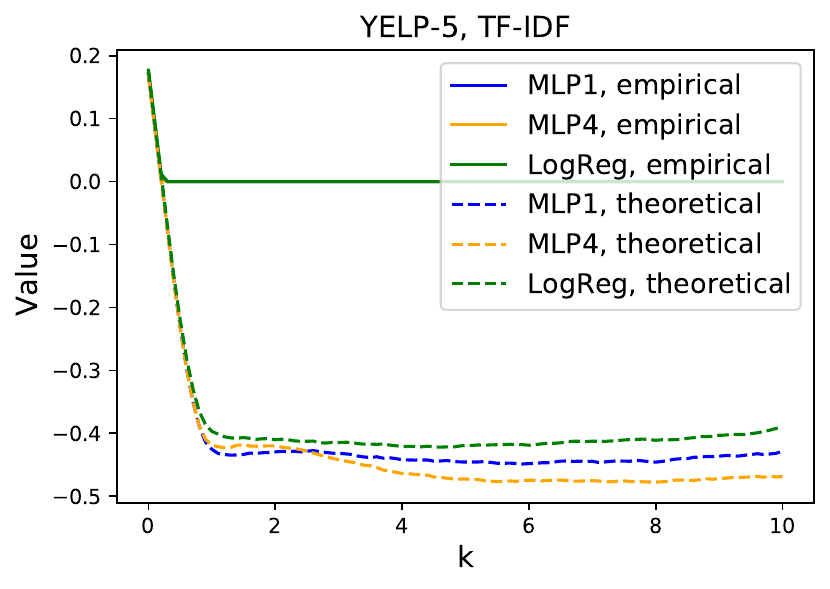}
    \includegraphics[width=.3\linewidth]{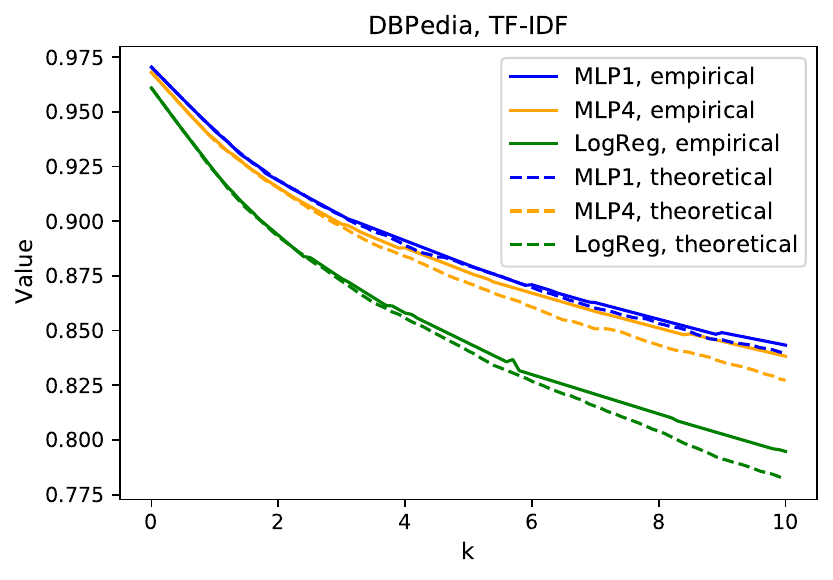}
    \includegraphics[width=.3\linewidth]{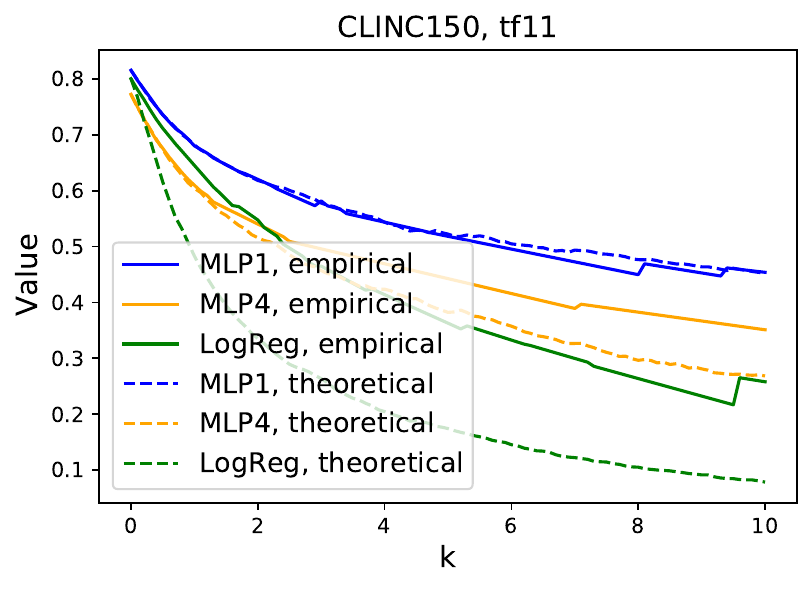}
    \includegraphics[width=.3\linewidth]{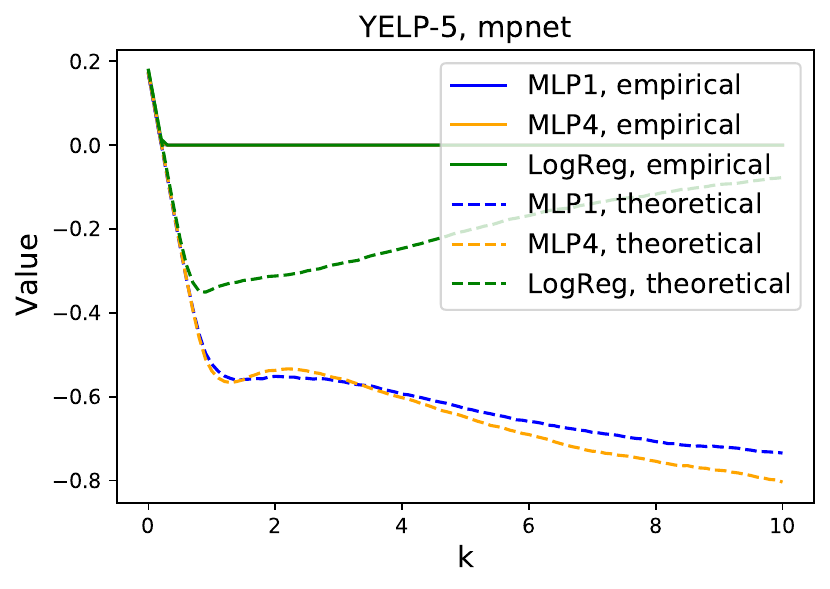}
    \includegraphics[width=.3\linewidth]{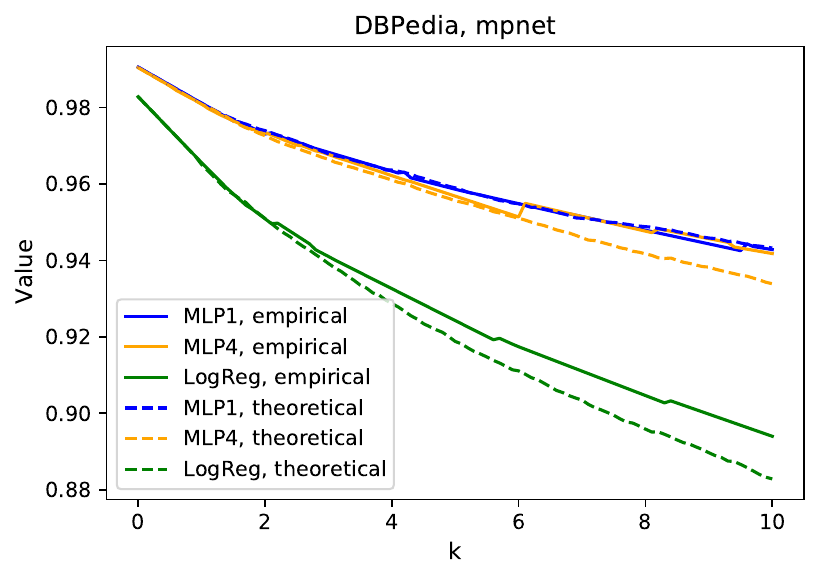}
    \includegraphics[width=.3\linewidth]{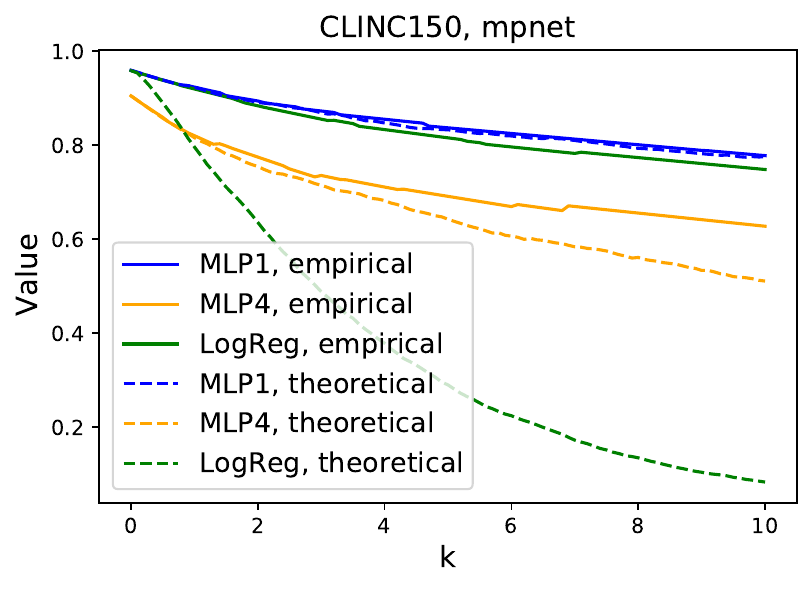}
    \includegraphics[width=.3\linewidth]{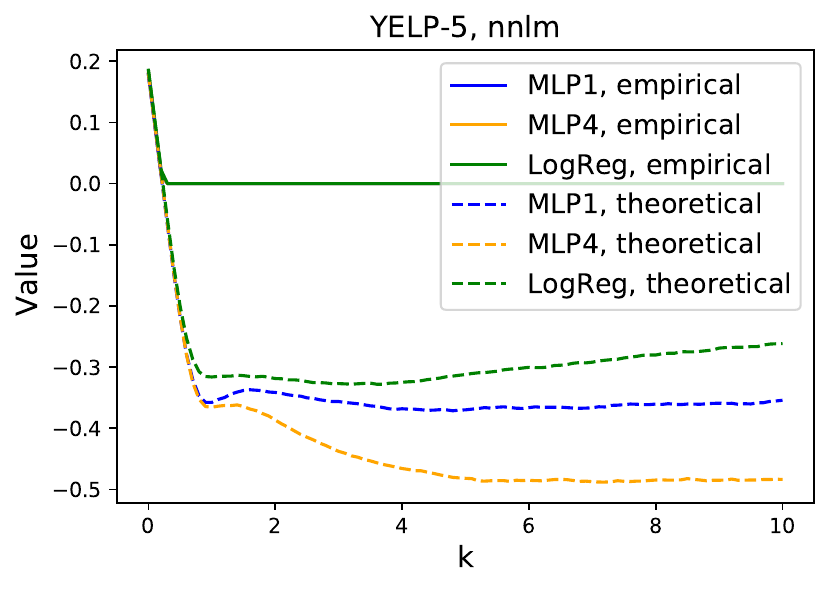}
    \includegraphics[width=.3\linewidth]{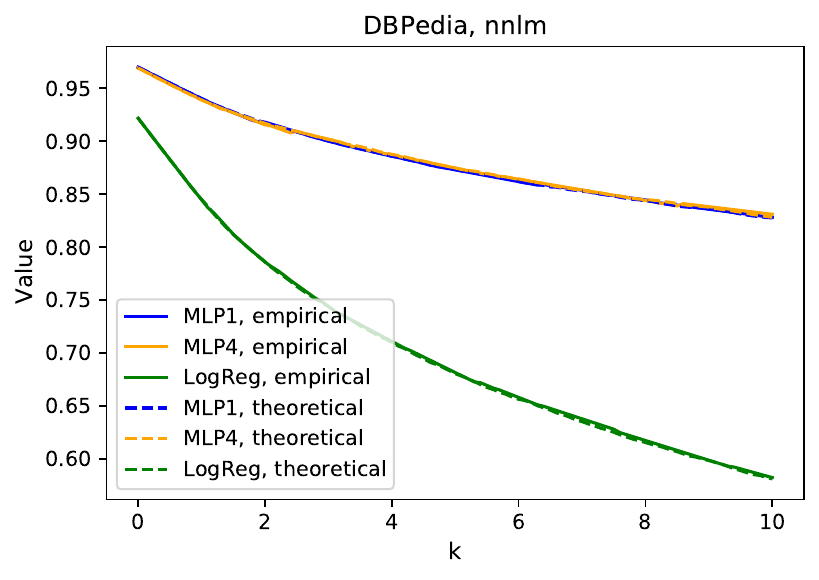}
    \includegraphics[width=.3\linewidth]{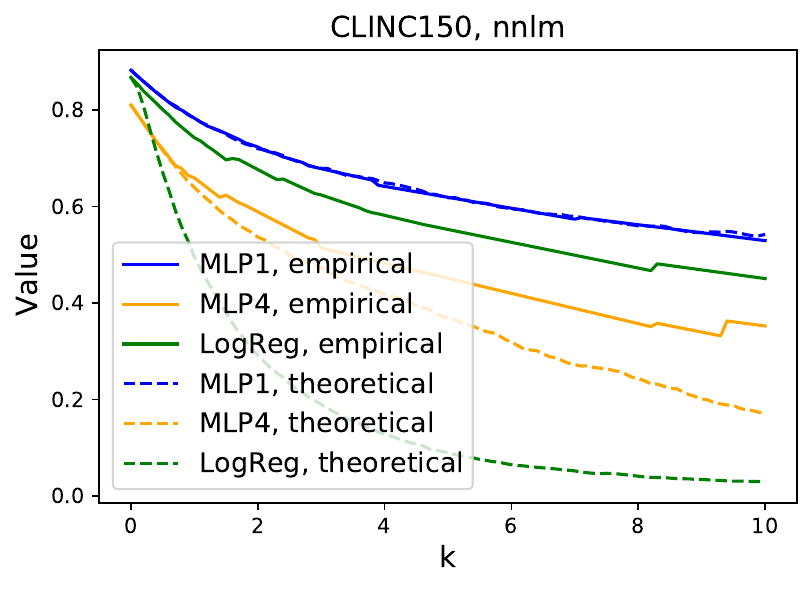}
    \includegraphics[width=.3\linewidth]{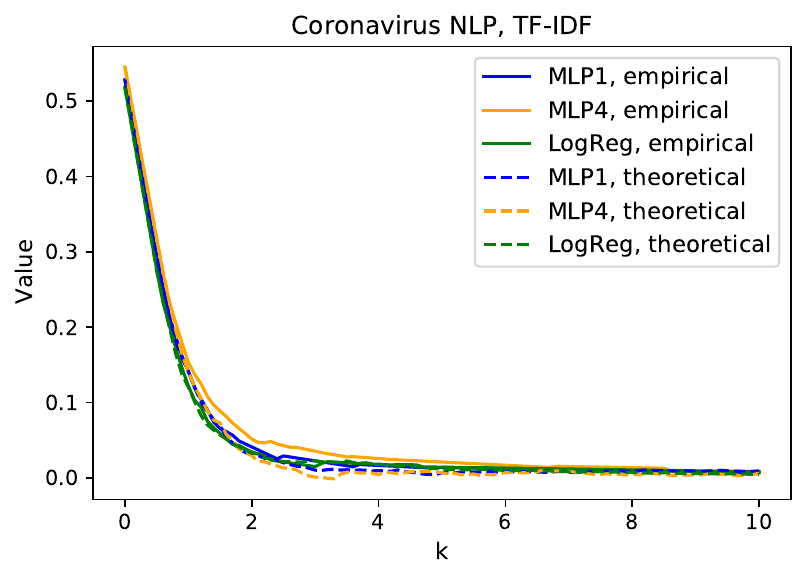}
    \includegraphics[width=.3\linewidth]{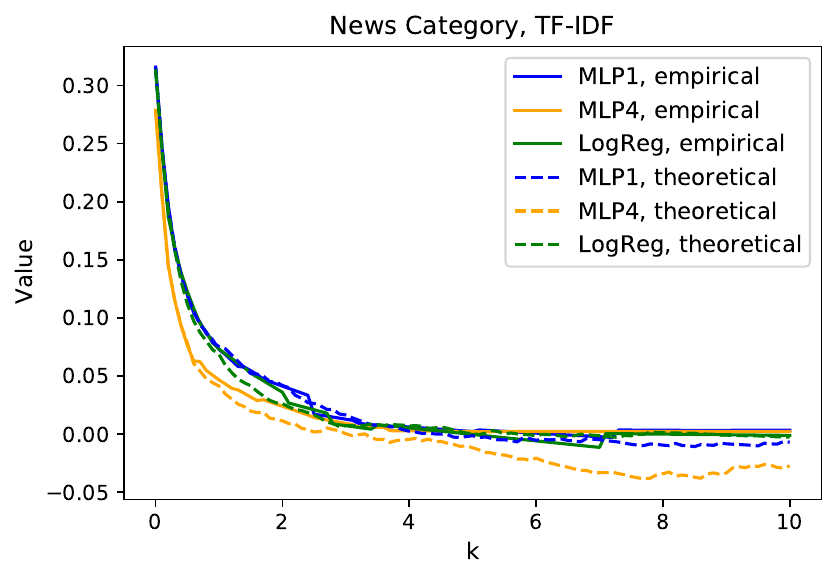}
    \includegraphics[width=.3\linewidth]{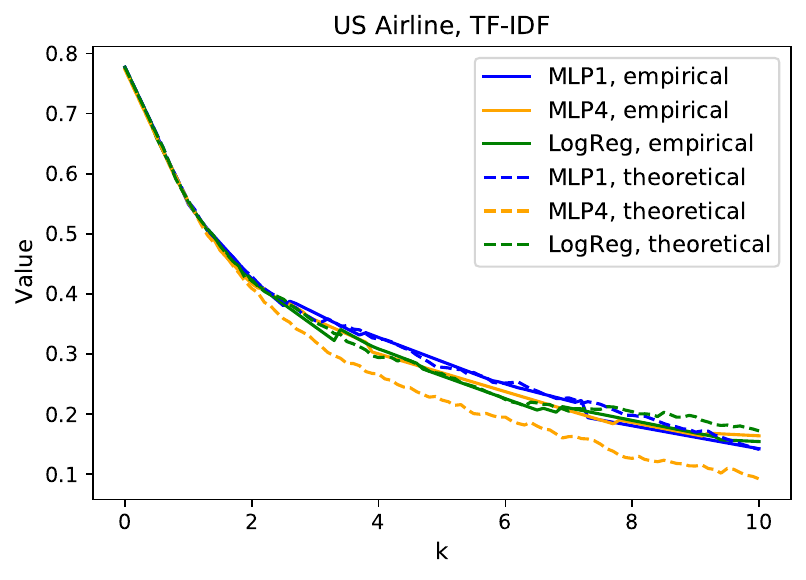}
    \includegraphics[width=.3\linewidth]{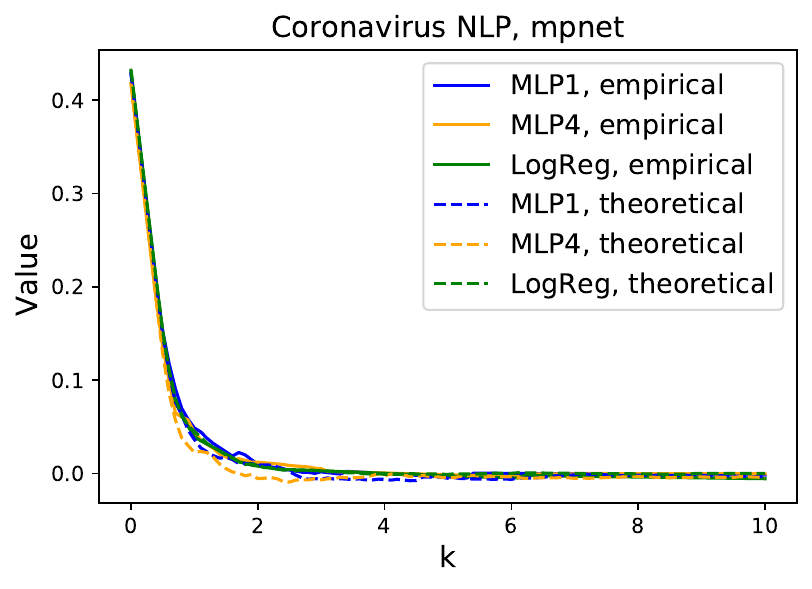}
    \includegraphics[width=.3\linewidth]{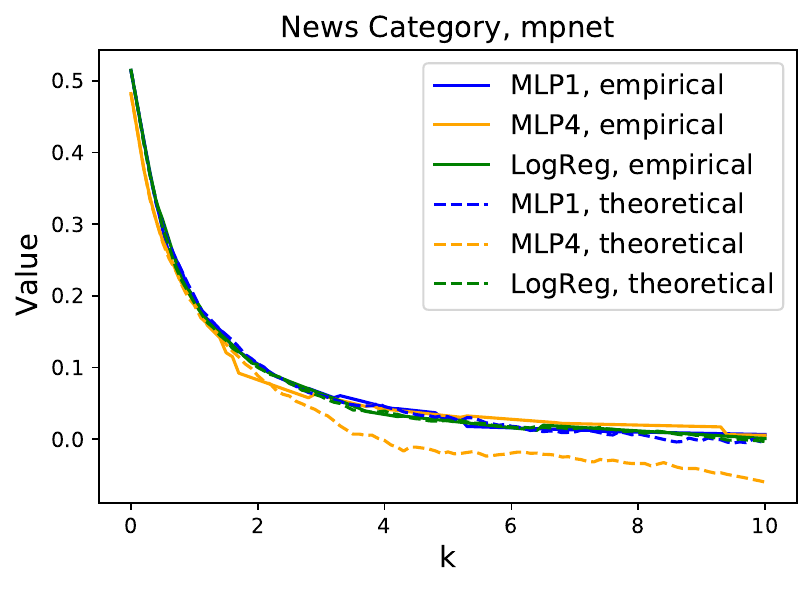}
    \includegraphics[width=.3\linewidth]{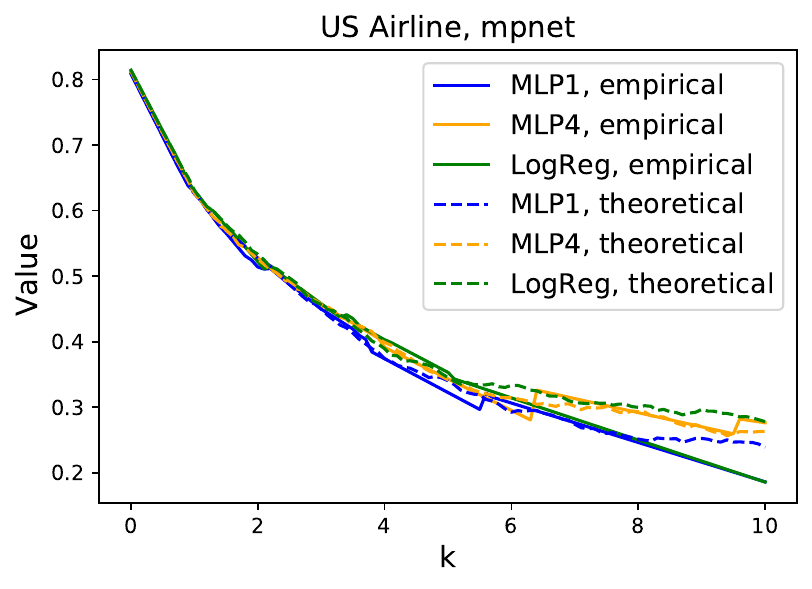}
    \includegraphics[width=.3\linewidth]{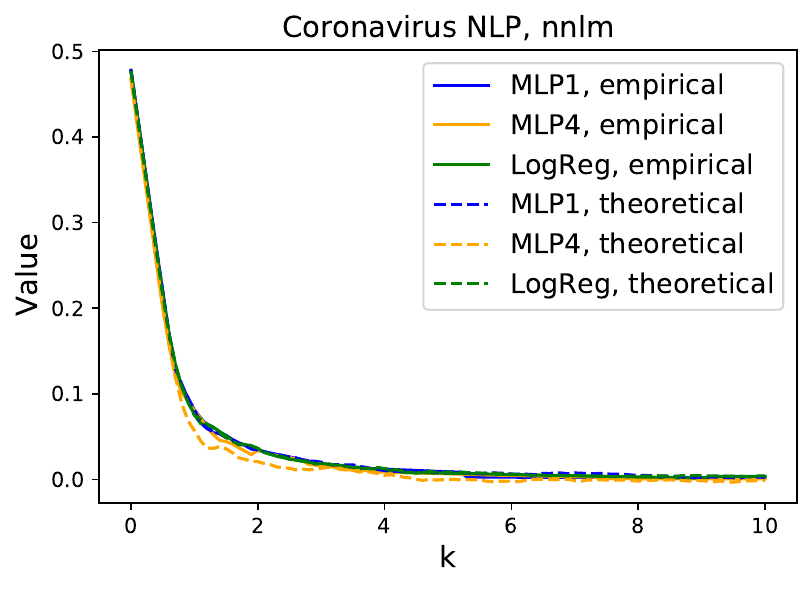}
    \includegraphics[width=.3\linewidth]{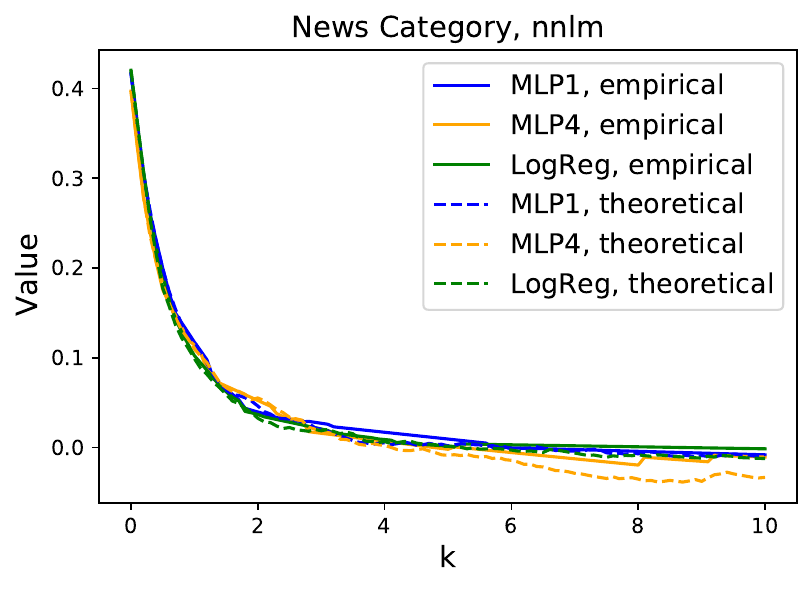}
    \includegraphics[width=.3\linewidth]{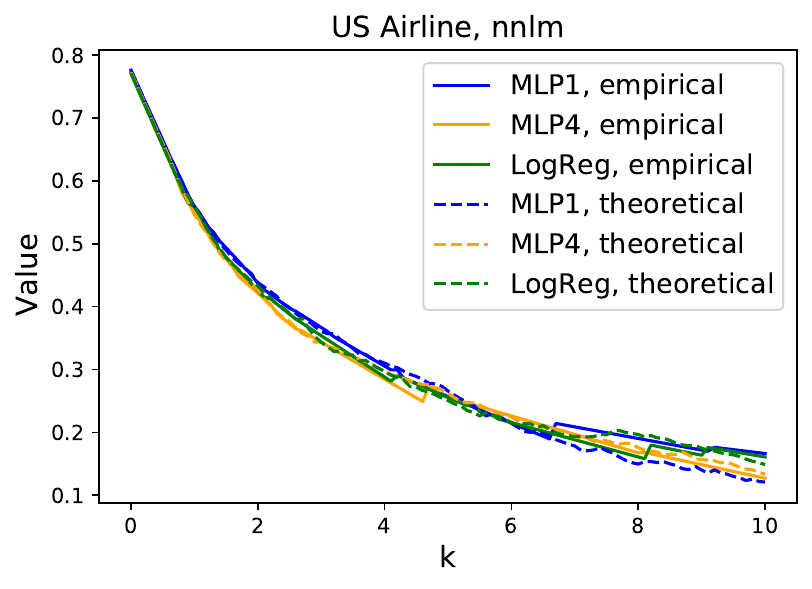}
    \includegraphics[width=.3\linewidth]{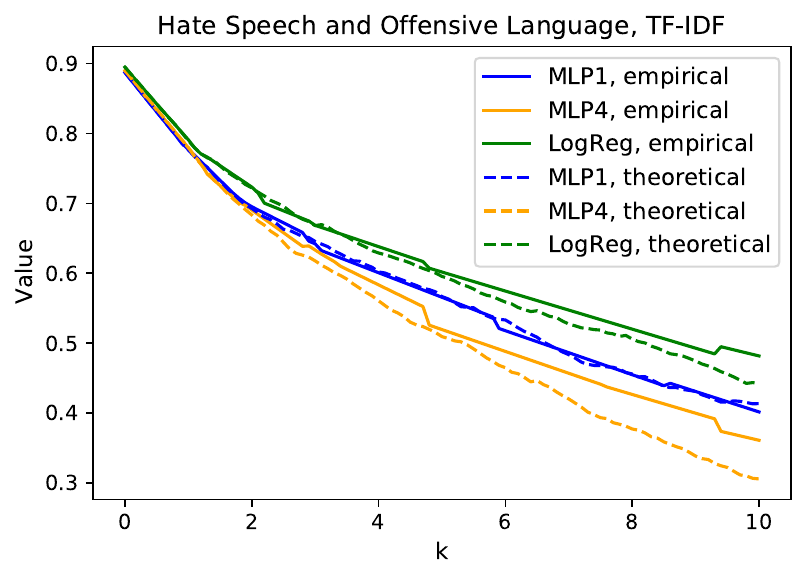}
    \includegraphics[width=.3\linewidth]{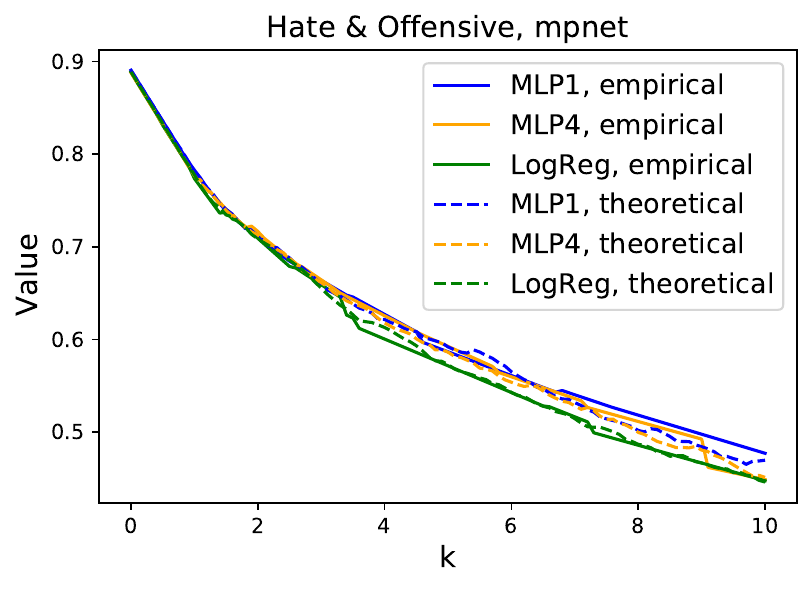}
    \includegraphics[width=.3\linewidth]{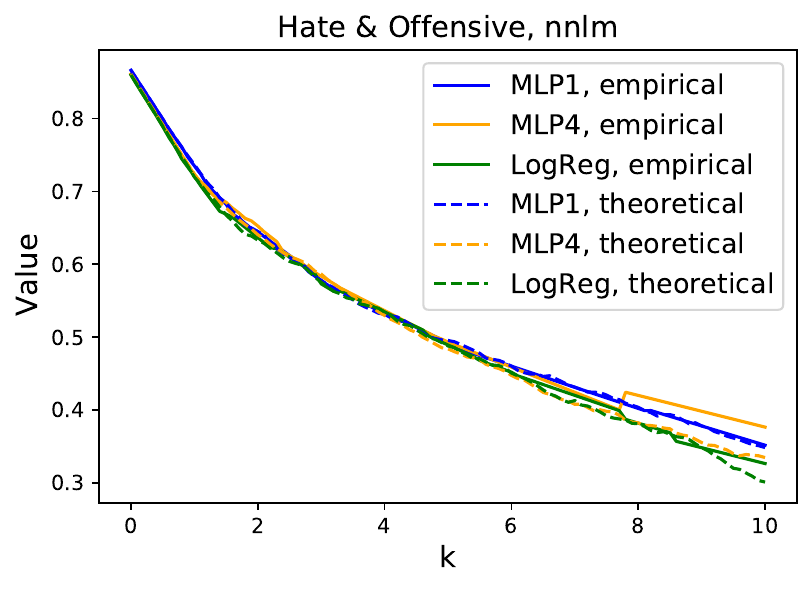}
    
    \caption{\label{fig:value_curve_effectOfEncoders}Effect of using different text encoders. Value curves with theoretical and empirical
      threshold (on the validation set) for increasing $k$.}
      \vspace{-0.15in}
\end{figure*}%%
